# Supplementary material for: The Quasar Feedback Survey: Discovering hidden Radio-AGN and their connection to the host galaxy ionised gas
Source: arXiv:2103.00014 ancillary file (2021-02-26)
Supplement: Supplementary file 1 [file QFeedS_supplement.pdf]

MNRAS 000, 1–13 (2020) Preprint 25 February 2021 Compiled using MNRAS LaTeX style file v3.0

# Supplementary information

This document contains the appendices to the main paper (The Quasar Feedback Survey: Discovering hidden Radio-AGN and their connection to the host galaxy ionised gas) including details of the VLA observations and imaging (Appendix A) and additional details on each of the sources in the sample (Appendix B).

## APPENDIX A: OBSERVATIONS AND IMAGES

This appendix contains a table listing the key properties of the VLA observations and images used in this work (Table A1). The noise in each image was calculated as the standard deviation from a square region with width 50 times the size of the beam major axis. The final noise measurements were calculated after applying $8\sigma$ clipping, repeated ten times, to remove all sources of emission.

## APPENDIX B: IMAGES AND NOTES ON INDIVIDUAL OBJECTS

In this appendix we provide images showcasing the data used in this paper for each source (Figs B1 – B41, except for the images for J1553+4407 that are shown in Fig. 2). We additionally discuss the radio data and any relevant literature results for individual sources in Sections B1 – B42.

### B1 J0749+4510

This Type 1 source is one of the five radio-loud sources in our sample, according to the Xu et al. (1999) criteria (Fig. 1). It has been well studied in previous literature. Specifically, it is a known gamma ray source, is optically variable and is known to contain a flat spectrum radio source (Nolan et al. 2012; Hovatta et al. 2014; Healey et al. 2007).

**Summary of radio properties:** We summarise the data used in this work for J0749+4510 in Fig. B1. We confirm the presence of a flat spectrum radio core ($\alpha$ = 0.3; see Table 2 and Fig. B1). This source is almost certain to host a powerful jet. However, the radio morphology for this source is unusual, with a possible lobe or hot spot visible in the FIRST image located 66.5 kpc southeast from the core. This feature is not detected in our higher resolution images, suggesting it is a diffuse radio structure. Our VLA L-band image shows a diffuse curved structure to the west of the core, possibly indicating procession or bending of the jet. The AGN origin of the radio emission in this source is unambiguous.

### B2 J0752+1935

This Type 1 source is known to be bright in hard X-rays, with a detection in the *Swift*-BAT all-sky survey indicating a hard-band luminosity of $L_{14-195\mathrm{keV}} = 10^{44.7}$ erg s$^{-1}$ (Oh et al. 2018). Far infrared spectroscopy with *Herschel* of J0752+1935 resulted in a detection of both the [O I]63$\mu$m and the [C II]158$\mu$m emission lines (Zhao et al. 2016). The [O I] line exhibits a broad velocity component with FWHM $\approx$ 730 km s$^{-1}$. We note that a broad component is also observed in the optical emission lines, but with a broader width of FWHM $\approx$ 1000 km s$^{-1}$ (Mullaney et al. 2013; Zhao et al. 2016). In contrast, the [C II] emission does not have any broad component detectable in the spectra, possibly because the high velocity gas is also at a high density and results in suppression of the [C II] emission (Zhao et al. 2016).

**Summary of radio properties:** We present the radio images used in this work for J0752+1935 in Fig. B2. This source is extended in our L-band image, although not resolved into distinct components. The higher resolution C-band image reveals extended structures to the northwest and to south of the source. This steep spectrum emission could be due to a disrupted jet. This could also be consistent with our finding that this source has a wide [O III] line and is possibly associated with a *Fermi* $\gamma$-ray source (Massaro et al. 2012). Nonetheless, we conclude that the AGN origin of the radio emission is ambiguous in the absence of further data.

### B3 J0759+5050

Villar Martín et al. (2014) used SDSS spectroscopy to study the [O III] kinematics of this Type 2 source. They identified this source as radio excess, consistent with our findings (Section 4.5), and attribute the broad [O III] line (FWHM = 958 km s$^{-1}$; Table 1; also see Mullaney et al. 2013) to an unseen <5 kpc jet.

**Summary of radio and ionised gas properties:** Our VLA C-band data for J0759+5050, presented in Fig. B3, reveals a 0.85 kpc lobe–core or jet-like structure. Due to the small separation between these structures, the $64\sigma$ contour was used to calculate the core spectral index in Section 4.3. *HST* continuum observations, reveal a regular lenticular host galaxy morphology and no co-spatial optical counterpart to this extended radio component (Zhao et al. 2019). There is evidence for a spatial connection between the radio emission and ionised gas kinematics by combining our knowledge of the radio emission with the *HST*/STIS long-slit data and the [O III] narrow-band images presented in Fischer et al. (2018) (also see Trindade Falcao et al. 2020). They observe irregular [O III] emission-line knots extended up to 3 arcsec along the same axis as the radio emission we have spatially resolved, i.e. along a PA of approximately 100°. Using the long-slit spectroscopy, Fischer et al. 2018 infer an outflow distance of 620 pc, based on the spatial extent of broad [O III] emission-line components. This is along the same axis as the radio emission, which we find is extended on scales of 850 pc (Fig. B3). The identification of a Radio-AGN in J0759+5050 is unambiguous.

© 2020 The Authors

**Table A1.** The key properties of the VLA observations and images used in this work. (1) Source name; (2) VLA calibrator used for the C-band A-array observations (referred to as the HR images throughout this work); (3) date of the C-band A-array observations in the format year-month-day; (4) noise ($\mu$Jy / beam) in the C-band A-array image; (5) size of the beam of the C-band A-array image (half power beam width - HPBW in arcsec, formatted as major axis size × minor axis size); (6) VLA calibrator used for the L-band A-array observations (referred to as the MR images throughout this work); (7) date of the L-band A-array observations in the format year-month-day; (8) noise ($\mu$Jy / beam) in the L-band A-array image; (9) size (HPBW in arcsec) of the beam of the L-band A-array image (major axis size × minor axis size).

| | C-band (HR) | | | | L-band (MR) | | | |
|---|---|---|---|---|---|---|---|---|
| Name | calibrator | obs date yyyy-mm-dd | noise ($\mu$Jy/beam) | beam size (arcsec) | calibrator | obs date yyyy-mm-dd | noise ($\mu$Jy/beam) | beam size (arcsec) |
| (1) | (2) | (3) | (4) | (5) | (6) | (7) | (8) | (9) |
| J0749+4510 | 0808+4950 | 2018-03-09 | 186 | 0.30×0.28 | 0818+4222 | 2018-03-18 | 234 | 1.21×1.05 |
| J0752+1935 | 0854+2006 | 2018-03-02 | 14 | 0.38×0.29 | 0854+2006 | 2018-03-05 | 64 | 1.17×1.15 |
| J0759+5050 | 0808+4950 | 2018-03-09 | 18 | 0.31×0.28 | 0818+4222 | 2018-03-18 | 91 | 1.24×1.00 |
| J0802+4643 | 0808+4950 | 2018-03-09 | 10 | 0.32×0.27 | 0818+4222 | 2018-03-18 | 47 | 1.18×1.02 |
| J0842+0759 | 0854+2006 | 2018-03-02 | 16 | 0.49×0.29 | 0854+2006 | 2018-03-05 | 72 | 1.16×1.03 |
| J0842+2048 | 0854+2006 | 2018-03-02 | 6 | 0.44×0.29 | 0854+2006 | 2018-03-05 | 38 | 1.12×1.04 |
| J0907+4620 | 0948+4039 | 2018-03-09 | 15 | 0.34×0.28 | 0818+4222 | 2018-03-18 | 61 | 1.41×1.01 |
| J0909+1052 | 0854+2006 | 2018-03-02 | 11 | 0.51×0.29 | 0854+2006 | 2018-03-05 | 47 | 1.18×1.09 |
| J0945+1737 | 0954+1743 | 2014-03-27 | 12 | 0.29×0.27 | 0954+1743 | 2014-05-13 | 89 | 1.59×1.11 |
| J0946+1319 | 0854+2006 | 2018-03-02 | 20 | 0.63×0.29 | 0854+2006 | 2018-03-05 | 46 | 1.16×1.03 |
| J0958+1439 | 0954+1743 | 2014-03-27 | 8 | 0.30×0.27 | 0954+1743 | 2014-05-13 | 25 | 1.73×1.11 |
| J1000+1242 | 0954+1743 | 2014-03-27 | 12 | 0.30×0.27 | 0954+1743 | 2014-05-13 | 41 | 1.64×1.12 |
| J1010+0612 | 1024-0052 | 2014-03-27 | 53 | 0.31×0.28 | 1041+0610 | 2014-05-13 | 480 | 1.98×0.90 |
| J1010+1413 | 0954+1743 | 2014-03-27 | 9 | 0.30×0.27 | 0954+1743 | 2014-05-13 | 146 | 1.68×0.91 |
| J1016+0028 | 1058+0133 | 2018-03-22 | 13 | 0.31×0.28 | 1120+1420 | 2018-03-19 | 44 | 1.65×1.11 |
| J1016+5358 | 0948+4039 | 2018-03-09 | 5 | 0.41×0.27 | 1035+5628 | 2018-03-18 | 27 | 1.64×0.96 |
| J1045+0843 | 1058+0133 | 2018-03-22 | 11 | 0.31×0.27 | 1120+1420 | 2018-03-19 | 49 | 1.34×1.20 |
| J1055+1102 | 1122+1805 | 2018-03-22 | 9 | 0.31×0.28 | 1120+1420 | 2018-03-19 | 28 | 1.29×1.14 |
| J1100+0846 | 1058+0133 | 2014-03-27 | 33 | 0.32×0.27 | 1041+0610 | 2014-05-13 | 105 | 1.58×1.12 |
| J1108+0659 | 1058+0133 | 2018-03-22 | 11 | 0.32×0.28 | 1120+1420 | 2018-03-19 | 56 | 1.27×1.05 |
| J1114+1939 | 1122+1805 | 2018-03-22 | 13 | 0.30×0.28 | 1120+1420 | 2018-03-19 | 34 | 1.18×1.13 |
| J1116+2200 | 1122+1805 | 2018-03-22 | 13 | 0.29×0.28 | 1120+1420 | 2018-03-19 | 47 | 1.15×1.12 |
| J1222-0007 | 1239+0730 | 2018-03-22 | 8 | 0.37×0.28 | 1254+1141 | 2018-03-19 | 49 | 1.29×1.09 |
| J1223+5409 | 1349+5341 | 2018-03-02 | 184 | 0.61×0.27 | 1354+5458 | 2018-03-07 | 1635 | 1.25×1.04 |
| J1227+0419 | 1239+0730 | 2018-03-22 | 10 | 0.35×0.29 | 1254+1141 | 2018-03-19 | 54 | 1.20×1.02 |
| J1300+0355 | 1239+0730 | 2018-03-22 | 73 | 0.39×0.28 | 1254+1141 | 2018-03-19 | 47 | 1.22×1.06 |
| J1302+1624 | 1239+0730 | 2018-03-22 | 18 | 0.35×0.28 | 1254+1141 | 2018-03-19 | 53 | 1.14×1.01 |
| J1316+1753 | 1327+2210 | 2014-03-27 | 8 | 0.33×0.28 | 1327+2210 | 2014-05-13 | 27 | 1.16×1.06 |
| J1324+5849 | 1349+5341 | 2018-03-02 | 10 | 0.47×0.28 | 1354+5458 | 2018-03-07 | 34 | 1.27×1.04 |
| J1347+1217 | – | 1985-03-03 | 75 | 0.41×0.40 | – | 1984-11-24 | 138 | 1.26×1.21 |
| J1355+2046 | 1430+1043 | 2018-03-20 | 6 | 0.29×0.27 | 1445+0958 | 2018-03-19 | 44 | 1.44×1.05 |
| J1356+1026 | 1415+1320 | 2014-03-27 | 59 | 0.36×0.28 | 1415+1320 | 2014-05-13 | 162 | 1.18×1.06 |
| J1430+1339 | 1415+1320 | 2014-03-27 | 13 | 0.40×0.29 | 1415+1320 | 2014-05-13 | 41 | 1.15×1.06 |
| J1436+4928 | 1349+5341 | 2018-03-02 | 12 | 0.41×0.28 | 1354+5458 | 2018-03-07 | 38 | 1.18×1.08 |
| J1454+0803 | 1430+1043 | 2018-03-20 | 13 | 0.31×0.28 | 1445+0958 | 2018-03-19 | 46 | 1.35×1.07 |
| J1509+1757 | 1430+1043 | 2018-03-20 | 12 | 0.29×0.28 | 1445+0958 | 2018-03-19 | 41 | 1.19×1.07 |
| J1518+1403 | 1430+1043 | 2018-03-20 | 12 | 0.31×0.28 | 1609+2641 | 2018-03-19 | 30 | 1.22×1.06 |
| J1553+4407 | 1638+5720 | 2018-03-02 | 6 | 0.34×0.28 | 1635+3808 | 2018-03-07 | 28 | 1.19×1.09 |
| J1555+5403 | 1638+5720 | 2018-03-02 | 6 | 0.35×0.27 | 1635+3808 | 2018-03-07 | 28 | 1.33×1.06 |
| J1655+2146 | 1658+0741 | 2018-03-20 | 8 | 0.36×0.28 | 1609+2641 | 2018-03-19 | 34 | 1.11×1.04 |
| J1701+2226 | 1658+0741 | 2018-03-20 | 13 | 0.36×0.28 | 1609+2641 | 2018-03-19 | 39 | 1.07×1.00 |
| J1715+6008 | 1638+5720 | 2018-03-02 | 14 | 0.34×0.27 | 1635+3808 | 2018-03-07 | 36 | 1.54×1.08 |

## B4 J0802+4643

We present the data used in this work for this radio-quiet Type 2 source in Fig. B4.

**Summary of radio properties:** J0802+4643 is unresolved in all of the radio images, except for our C-band image where it shows a structure extending to the southwest of a steep spectrum core. Due to blending of this extended structure and the radio core, the 64$\sigma$ contour was used to calculate the core spectral index for this source in Section 4.3. Although this has a jet-like morphology, due to a lack of ancillary information, we cannot confirm an AGN origin of this radio emission.

## B5 J0842+0759

This Type 1 source is detected in the *Swift*-BAT all-sky hard X-ray survey with a luminosity of $L_{14-195\mathrm{keV}} = 10^{44.8}\,\mathrm{erg\,s^{-1}}$ (Oh et al. 2018). Based upon the criteria of Xu et al. (1999) it is radio-quiet; however, it is moderately radio-loud, with $R = 1.2$, based upon the criteria of Ivezić et al. (2002) (see Section 2.4).

**Summary of radio properties:** Our data, presented in Fig. B5, reveal that J0842+0759 shows no distinct features in any of its radio images. However, the C-band data is marginally extended, with a deconvolved size of 1.8 kpc. Furthermore, this emission shows signatures of a flattening radio spectrum towards the peak ($\alpha = -0.4$; Fig. B5). This suggests that we are observing a barely resolved lobe–core–lobe structure; however, higher resolution radio images would be needed to confirm this hypothesis. Overall, we conclude an AGN origin for the radio emission in this source.

### B6 J0842+2048

This Type 1 source is classified as radio-quiet upon the criteria of Xu et al. (1999); however, it is moderately radio-loud, with $R = 1.1$ based upon the criteria of Ivezić et al. (2002) (see Section 2.4).

**Summary of radio properties:** Our radio data, presented in Fig. B6, reveal no distinct morphological features; however, the C-band image reveals marginally extended, steep spectrum radio emission (i.e. a deconvolved size of ~0.5 kpc and $\alpha = -0.7$). Due to the lack of ancillary data available, the origin of the radio emission in J0842+2048 remains ambiguous.

### B7 J0907+4620

The Type 2 source is classified as radio-loud based upon the criteria of Xu et al. (1999).

**Summary of radio properties:** The radio images, presented in Fig. B7, reveal a complex radio morphology. Due to blending of radio structures in the C-band data for this source the $64\sigma$ contour was used to calculate the core spectral index in Section 4.3. A radio lobe exists 35 kpc towards the west, as revealed by the FIRST image. This is detected with low significance in our L-band data but not at all in our C-band data. The lack of an optical counterpart for this radio emission suggests that it could originate from a jet. In our higher resolution images of J0907+4620 we observe additional signatures of deflected jets to the northeast and southwest of a radio core. The jet interpretation is further supported by the observation of a moderately flat spectrum core from our C-band spectral index map ($\alpha = -0.6$). We conclude an AGN origin of the radio emission for J0907+4620.

### B8 J0909+1052

We present the radio data for this radio-quiet Type 2 source in Fig. B8.

**Summary of radio properties:** This sources has steep spectrum radio emission with no notable features, although the C-band image is marginally extended over approximately a kiloparsec. Due to the lack of ancillary information available for J0909+1052 we cannot confirm an AGN origin of the radio emission.

### B9 J0945+1737

In agreement with our work, this source has previously been identified as a LIRG with a Type 2 AGN nucleus (Kim et al. 1995; Veilleux et al. 1995). *Spitzer* IRS spectroscopy reveal that the mid-infrared emission from J0945+1737 is dominated by AGN emission, with an infrared AGN luminosity of $\log(L_{\rm IR,AGN}/{\rm ergs}^{-1}) = 44.9$ (Sargsyan et al. 2008; Nardini et al. 2010). However, J0945+1737 is also bright in CO(2–1) emission, and is consistent with being a gas rich star-forming galaxy (Jarvis et al. 2020). We present the data used in this work for this source in Fig. B9.

**Summary of radio and ionised gas properties:** J0945+1737 has excess radio emission above that expected from star formation, indicating radio emission associated with an AGN (Section 4.5; also see Jarvis et al. 2019). Radio structures can be seen approximately 2 kpc to the east and 11 kpc to the northwest of the nucleus (Fig. B9; also see Jarvis et al. 2019). We have previously presented GMOS IFS data and radio imaging for this source, which revealed complex ionised kinematics associated with the radio structure to the east, indicative of a jet–ISM interaction (Harrison et al. 2014; Jarvis et al. 2019; also see Kang & Woo 2018). Furthermore, *HST* observations of this source reveal a single nucleus in the continuum (Cui et al. 2001) and confirm an extended and irregular emission line region, visible in narrow band filters covering both the [O III] and H$\alpha$+[N II] emission lines (Storchi-Bergmann et al. 2018). We have shown that these extended emission-line regions are spatially co-incident with the radio structures in Jarvis et al. (2019). We conclude that the radio emission in J0945+1737 is associated with the AGN.

### B10 J0946+1319

Far infrared spectroscopy of this radio-quiet Type 1 source from *Herschel* reveal a narrow [C II]158$\mu$m emission line (FWHM = 311 km s$^{-1}$) and no detection of the [O I]63$\mu$m emission line (Zhao et al. 2016). However, the optical spectroscopy reveals broad and complex emission line profiles and this source has one of the broadest [O III] emission line widths across the sample (FWHM$_{\rm [OIII]}$ = 1193 km s$^{-1}$; Table 1).

**Summary of radio properties:** The data used in this work, presented in Fig. B10, reveal no notable features in our L-band radio data. However, due to the spatial offset and structure in the spectral index map seen in the C-band data (i.e. flattening towards the south-east) there is evidence for a ~1.7 kpc extended radio structure. IFS data and higher resolution radio imaging are now required to establish any connection between the radio emission and the ionised gas kinematics. Based upon the excess radio emission, above that expected from star formation (see Section 4.5), we conclude that J0946+1319 hosts a Radio-AGN.

### B11 J0958+1439

This radio-quiet Type 2 source was previously presented by us in Harrison et al. (2014) and Jarvis et al. (2019) (also see Kang & Woo 2018). We present the data used in this work for this source in Fig. B11. It can be seen that the optical image indicates a regular disk/spiral galaxy morphology for the AGN host galaxy. Furthermore, the lack of a CO(2–1) detection in Jarvis et al. (2020) could not rule out that this source is a gas rich star-forming galaxy.

**Summary of radio and ionised gas properties:** In our previous works, by combining GMOS IFS data with radio imaging, we noted a spatial association between kinematic line splitting of the [O III] emission line and a double radio lobe structure separated by ~1 kpc (Jarvis et al. 2019). This radio structure can be seen in the C-band image presented in Fig. B11. Due to the small separation between these structures, the $75\sigma$ contour was used to calculate the core spectral index in Section 4.3, although we note that it is likely that both components are actually radio lobes with no detected radio core in this source with our images. Nonetheless, due to the symmetric double radio morphology of this source we define it as a Radio-AGN (see Section 4.2).

## B12 J1000+1242

We have previously presented IFS data and radio imaging for this Type 2 radio-quiet source in Harrison et al. (2014) and Jarvis et al. (2019). Optical *HST* imaging reveals double nuclei, separated by ∼1 arcsec, and filaments of emission-line gas running north-south (Jarvis et al. 2019). Based upon the infrared and CO(2–1) emission, we identified J1000+1242 as a gas rich star-forming galaxy in Jarvis et al. (2020). The radio images used in this work are presented in Fig. B12.

**Summary of radio and ionised gas properties:** In Jarvis et al. (2019), using VIMOS IFS data, we detected a giant emission-line region to the north and south of the nucleus. This extended emission line region can be seen in the optical imaging in Fig. B12 because the green band is dominated by high equivalent width line emission. This emission-line region was previously identified by Sun et al. (2017) using long-slit observations; however, our IFS data enabled us to associate the northern emission with a giant (i.e. ∼15 kpc) outflowing bubble using the [O III] kinematics. Furthermore, the regions of brightened and kinematically disturbed ionised gas are associated with co-spatial radio emission. As can been seen in Fig. B12, the radio hot spots, surrounded by diffuse radio lobes are tracing the emission line region (in green). We note that, in Jarvis et al. (2019) we used our VLA B-array C-band image (see white contours in Fig. B12) to measure the spatial extent of the radio emission, compared to using the A-array L-band image in this work. Consequently, in Jarvis et al. (2019) we measured a slightly larger radio size of 25 kpc, compared to the measurement of 21 kpc used in this work. Beam residuals in the C-band data for this source led to the $64\sigma$ contour being used to calculate the core spectral index in Section 4.3. Due to the excess radio emission above that expected from star formation (Section 4.5) and the high brightness temperature (Section 4.4), the AGN origin of the radio emission in J1000+1242 is unambiguous.

## B13 J1010+0612

Using SDSS spectra of this Type 2 radio-quiet source, the [O III] kinematics were studied by Villar Martín et al. (2014) who identified an ionised outflow (also see Mullaney et al. 2013) and proposed it was triggered by a small scale radio jet. We previously presented GMOS IFS data and radio imaging for J1010+0612 in Harrison et al. (2014) and Jarvis et al. (2019) (also see Kang & Woo 2018). In Jarvis et al. (2020) we determined that the host is a gas rich star-forming galaxy using SED fitting and CO(2–1) data.

**Summary of radio and ionised gas properties:** Our data confirm the presence of highly disturbed [O III] emission and bright radio emission (Harrison et al. 2014; Jarvis et al. 2019, Fig. B13). However, the radio images for this source, which are presented in Fig. B13, reveal that the radio emission is compact on scales of about 100 pc. Higher resolution radio imaging is required to firmly establish the properties of any jets in this source. Due to the excess radio emission above that expected from star formation (Section 4.5) and the high brightness temperature (Section 4.4) we confirm an AGN origin of the radio emission in J1010+0612.

## B14 J1010+1413

This Type 2 radio-quiet AGN has been the subject of several studies. We have previously presented GMOS and VIMOS IFS data for this source and combined these data with radio imaging (Harrison et al. 2014; Jarvis et al. 2019; also see Kang & Woo 2018). In Jarvis et al. (2020) we identified this source as a gas rich star-forming galaxy using SED fitting and CO(2–1) data.

Interestingly, this source appears to have undergone a merger based largely upon the disturbed morphology (Goulding et al. 2019). It could be that the jets in this source are colliding with tidally stripped material, left over by the merger and are ionising and kinematically disturbing this gas (see Fig. B14 and Jarvis et al. 2019). Goulding et al. (2019) even propose that this source may host a binary quasar as a result of a merger. They used *HST* observations to identify two continuum and [O III] emitting cores separated by ∼430 pc (or 0.13 arcsec). *Chandra* observations presented by Goulding et al. (2019) reveal marginally extended soft (0.5–3.5 keV) X-ray emission with $r \approx 1.9$ arcsec, for which the favoured interpretation is quasar-produced scattered light; however, these X-ray data are insufficient to spatially-resolve the two optical sources.

**Summary of radio and ionised gas properties:** The radio images used in this work are presented in Fig. B14. Due to jet-like extension of the core emission of this source in the C-band data, the $64\sigma$ contour was used to calculate the core spectral index in Section 4.3.

Our results on this source, first presented in Jarvis et al. (2019), reveal a giant ($\gtrsim$15 kpc) and irregular emission line region extending to the north and south of the nucleus. This extended emission line region can be seen in the optical imaging presented in Fig. B14 because the green band is dominated by high equivalent width line emission. This is also seen in the long-slit observations and *HST* imaging presented by Sun et al. (2017) and Goulding et al. (2019), respectively. It can also be seen in Fig. B14 that the radio emission is spatially coincident with the emission line region. In particular, we see the signature of a bent jet due to a jet–ISM interaction in the north (see Jarvis et al. 2019 for more details). We note that, in Jarvis et al. (2019) we used our VLA B-array C-band image to measure the spatial extent of the radio emission (see white contours in Fig. B14) and in this work we use the the A-array L-band image. Consequently, we measured a larger radio size of 15 kpc in Jarvis et al. (2019), compared to 10 kpc used in this work. We note that, based on our images, we do not see evidence for radio counterparts to both of the binary optical sources presented in Goulding et al. (2019). However, deep and higher resolution radio images are required to confirm the presence, or not, of radio emission associated with each of the optical components.

When we consider the infrared luminosity from the careful SED fitting see Jarvis et al. 2019, 2020, rather than the rough estimate from Section 4.5, we find that J1010+1413 is classified as having excess radio emission. Based upon this result and the observed radio morphology, we conclude that J1010+1413 contains a Radio-AGN.

## B15 J1016+0028

We present the images used in this work for this Type 2 radio-quiet source in Fig. B15.

**Summary of radio properties:** J1016+0028 has previously been identified as a "compact" double radio source by Jimenez-Gallardo et al. (2019). The double radio lobes are observed in both the FIRST image and our L-band image that are presented in Fig. B15. The lack of optical counterparts to these lobes suggests that these are radio lobes emitted from an undetected jet. J1016+0028 is completely undetected in our VLA C-band image and has no detected core emission in either the FIRST or L-band image. Deep and higher frequency data may allow for the identification of a flat spectrum core. However, the clear symmetric double

radio morphology centred on the AGN-host galaxy means that we classify J1016+0028 as a Radio-AGN.

## B16 J1016+5358

The data for this radio-quiet Type 2 source are shown in Fig. B16.

**Summary of radio properties:** The radio emission is featureless in both the FIRST image and our L-band image. However, the C-band data reveals an extended, steep spectrum, radio structure protruding ∼1 kpc to the north. However, the lack of ancillary data means that we cannot confirm an AGN origin of the radio emission for J1016+5358.

## B17 J1045+0843

This Type 1 source is classified as radio-quiet upon the criteria of Xu et al. (1999); however, it is on the boundary of radio-loudness, with $R = 1.0$ based upon the criteria of Ivezić et al. (2002) (see Section 2.4).

**Summary of radio properties:** All three radio images presented in Fig. B17 reveal no features beyond a compact, steep spectrum core. The lack of ancillary data for J1045+0843 means that we cannot confirm an AGN origin of the radio emission.

## B18 J1055+1102

Sun et al. (2017) presented long-slit data around the [O III] and H$\beta$ emission lines for this Type 2 radio-quiet source. They found that the emission line region radius is 6.6±1.3 kpc but there is no kinematically disturbed gas (defined as where $W_{80} > 600\,\mathrm{km\,s^{-1}}$).

**Summary of radio properties:** Our radio images, presented in Fig. B18, reveal a radio structure extending ∼3 kpc to the east. The 'green blob' observed in the optical image at the end of the radio emission (Fig. B18) could be a high equivalent width emission line region associated with this radio emission, similar to those observed in J1000+1242 (Fig. B12) and J1010+1413 (Fig. B14). It is interesting to note that the slit PA used in Sun et al. (2017) (i.e. at 180°) does not follow the direction of extended radio emission and therefore they are likely to have missed any kinematic disturbance associated with this radio emission. The lack of ancillary data for J1055+1102 means that we cannot confirm an AGN origin of the radio emission.

## B19 J1100+0846

Using SDSS spectra, the [O III] kinematics of this Type 2 radio-quiet source were studied by Villar Martín et al. (2014) and they identified it as having outflows based on the [O III] emission line (also seen by Mullaney et al. 2013). They proposed that the extreme ionised gas kinematics were driven by a compact jet. In Jarvis et al. (2020), based on SED fitting and CO(2–1) measurements, we showed that the host galaxy of this AGN is consistent with being a gas rich star-forming galaxy.

**Summary of radio and ionised gas properties:** The radio images used in this work are presented in Fig. B19 and we find that the majority of the radio emission is compact on $\lesssim$200 pc scales. However, in Jarvis et al. (2019) we found tentative evidence for a radio structure located 800 pc north of the nucleus based on 1.4 GHz imaging from e-MERLIN. We have previously presented GMOS IFS data for J1100+0846 in Harrison et al. (2014) and Jarvis et al. (2019) and in these works we confirmed the presence of kinematically disturbed ionised gas (also see Kang & Woo 2018). Fischer et al. 2018 (also see Trindade Falcao et al. 2020) confirm the disturbed kinematics in this source using *HST*/STIS long-slit observations around the [O III] emission line. They find that the emission line is broad (FWHM > 1000 km s$^{-1}$) across the nucleus. The outflow distance is measured by the authors, from the maximum extent of these high line widths, to be 450 pc northwest of the nucleus. This high velocity gas is found to be in the general direction of the tentative radio feature presented in Jarvis et al. 2019. Higher quality integral field spectroscopy and deeper radio observations are required to further understand the connection between the radio emission and ionised gas kinematics in this source.

We find that the level of radio emission is in excess of that expected from star formation (Section 4.5; also see Jarvis et al. 2019). Therefore, we conclude that J1100+0846 hosts a Radio-AGN.

## B20 J1108+0659

This radio-quiet Type 2 source has a double peaked [O III] emission-line profile in the SDSS fibre spectrum (see Fig. B20; Liu et al. 2010a). Therefore, J1108+0659 has been repeatedly investigated as a candidate for hosting a dual AGN using multi-wavelength surveys. Indeed, deep near-infrared and optical imaging, combined with spatially-resolved spectroscopy, reveal a double stellar bulge with a projected separation of about 0.6–0.7 arcsec (i.e. ∼2 kpc) at a PA of 140° and the two [O III] velocity components are spatially coincident with these continuum sources (but potentially with slightly larger separation; Liu et al. 2010b; Fu et al. 2011, 2012; Shen et al. 2011; Liu et al. 2013). These observations imply a major merger between two galaxies which have approximately equal near-infrared luminosity, and therefore equal stellar mass, but with different colours. Although it remains clear there is at least one AGN in this source (based upon the optical emission line ratios; Liu et al. 2010a; Fu et al. 2011, 2012; Mullaney et al. 2013), detailed analyses of the X-ray emission and infrared spectroscopy fail to robustly identify an AGN associated with each nucleus (Shangguan et al. 2016; Barrows et al. 2017; McGurk et al. 2015).

**Summary of radio properties:** We present the radio images used in this work for J1108+0659 in Fig. B20. As can be seen in the figure, the radio emission is extended but with no distinct spatially resolved features in our L-band data. In contrast, in the C-band it is resolved into three spatially distinct components. Bondi et al. (2016) obtained radio images at 1.4, 5.0 and 8.5 GHz of J1108+0659. Their imaging at 5.0 GHz is in excellent agreement with our own (Fig. B20). However, the higher spatial resolution provided by their 8.5 GHz imaging (i.e. ∼0.2 arcsec) reveals that the central component we observe is resolved into a compact core (their 'C1') and a resolved component to the west which they tentatively identify as a jet (their 'C2'). C1 is a candidate AGN radio core with a spectral index of $\alpha = -0.3 \pm 0.2$. However, they note this is offset by 0.2 arcsec from the nuclear optical and X-ray positions and it is not detected at the sensitivity of their European VLBI Network observations at 5 GHz, nor is it detected by Liu et al. (2018) using 8.4 GHz, ∼1.5 milliarcsecond resolution VLBA observations. Nonetheless, we use this information to suggest that J1108+0659 contains a Radio-AGN.

Liu et al. (2013) detected extended soft X-ray emission, over 1–2 arcsec north of the nucleus, which may be associated with the extended radio emission observed in this work and in Bondi et al. (2016), and the extended emission line region which is situated to

the north. Bondi et al. (2016) use *HST UV* imaging to associate both the northern and southern radio structures, also seen in our VLA data (Fig. B20), with star formation. Indeed, they derive a star formation rate for this source from the total $L_{\rm IR}$ of SFR = 100 $M_\odot$ yr$^{-1}$ and that excluding the central radio component, which they identify as an AGN, the radio derived star formation rate of the remaining extended structures gives SFR = 110 $M_\odot$ yr$^{-1}$, which is consistent within errors. This is further evidence that the radio *core* is from an AGN and not from star formation. We finally note that the spatial coincidence of the radio and *UV* features could alternatively be indicative of jet-induced star formation. Detailed analyses of spatially-resolved spectroscopy, in combination with these radio images will shed further light on the connection between the star formation, gas kinematics and AGN in J1108+0659.

### B21 J1114+1939

The images used in this work for this Type 2 radio-quiet source are presented in Fig. B21.

**Summary of radio properties:** All three radio images for this source are featureless (Fig. B21). Even our highest resolution C-band image reveals only compact, steep spectrum emission. The lack of ancillary data for J1114+1939 means that we cannot confirm an AGN origin of the radio emission.

### B22 J1116+2200

The data used in this work for this Type 2 radio-quiet source are presented in Fig. B22.

**Summary of radio properties:** Both the FIRST image and our L-band image are featureless. However, the C-band image shows a weak radio feature extended ~1.3 kpc to the southwest. The lack of ancillary data for J1116+2200 means that we cannot confirm an AGN origin of the radio emission.

### B23 J1222−0007

This Type 2 radio-quiet source appears to be part of an on-going merger (see imaging in Fig. B23). J1222-0007 has been previously studied using long slit spectroscopy in Greene et al. (2011). The authors identified the signatures of AGN driven disruption in the ionised gas throughout the host galaxy. Further long slit observations were obtained by Hainline et al. (2013) but were not included in their narrow line region size results due to the merger affecting their analyses. Liu et al. (2011) classified this source as an AGN pair with the secondary component in the merger (4.7 arcsec away) having a Seyfert classification. Comerford & Greene (2014) also selected this source as a candidate offset AGN (i.e. where the AGN is kinematically offset from the gravitational centre of the galaxy) based upon a ~100 km s$^{-1}$ velocity offset between the stellar absorption and both the forbidden lines and the Balmer lines in the SDSS spectra. We present the radio images, used in this work, for this source in Fig. B23.

**Summary of radio properties:** Our C-band image shows a possible triple (lobe – core – lobe) structure (Fig. B23). Indeed, the L-band image is extended along the same position angle, providing confidence that these structures are real. Taken together with the long-slit spectroscopy results of Greene et al. (2011), this could indicate that J1222-0007 has a jet or quasar wind triggered by a merger that is interacting strongly with the host galaxy ISM. We do not detect any radio emission associated with the secondary optical source presented in Liu et al. (2011) (Fig. B23). Due to the radio morphology, we classify J1222-0007 as a Radio-AGN.

### B24 J1223+5409

This Type 1 source is a known radio-loud source, meeting the radio-loud criteria of Xu et al. (1999) and appears in the fourth radio Cambridge Survey Catalogue as 4C+54.27 (Gower et al. 1967).

**Summary of radio properties:** Although unresolved in FIRST, it shows a distinct triple (lobe - core - lobe) morphology in both our L and C-band images presented in Fig. B24. The flat spectrum core ($\alpha = -0.5$), further demonstrates that this source contains a radio jet. The classification as a Radio-AGN for J1223+5409 is unambiguous.

### B25 J1227+0419

We present the radio images for this Type 2 radio-quiet source in Fig. B25.

**Summary of radio properties:** The radio images are all featureless, and our C-band data reveal a steep spectrum core, which is marginally resolved with a size of ~0.5 kpc. Due to a lack of ancillary data for this source, we cannot confirm an AGN origin for the radio emission for J1227+0419.

### B26 J1300+0355

This Type 1 source is classified as radio-quiet on the criteria of Xu et al. (1999); however, is moderately radio-loud based upon the criteria of Ivezić et al. (2002), with $R = 1.4$ (see Section 2.4). The optical imaging reveals two sources north of the primary target (Fig. B26).

**Summary of radio properties:** We identify radio emission with the brighter of the secondary optical components at 16.5 kpc north of the primary target (see Fig. B26). However, SDSS spectroscopy reveals that it is associated with a $z = 0.30$, Type 2 AGN, unrelated to our target AGN at $z = 0.18$. We note that this secondary source will also contaminate the radio classifications based solely on the FIRST data. The radio core, observed in our C-band spectral index image, is flat ($\alpha = 0.2$; Fig. B26). This suggests that it is the base of a jet. In combination with the high brightness temperature of this core (Section 4.4) we conclude that J1300+0355 hosts a Radio-AGN.

### B27 J1302+1624

This Type 1 source is a Markarian galaxy, Mrk 783. It was identified as a Narrow line Seyfert 1 galaxy by Osterbrock & Pogge (1985) and is detected in the *Swift*-BAT all-sky hard X-ray survey with a luminosity of $L_{14-195\rm keV} = 10^{44.2}$ erg s$^{-1}$ (Oh et al. 2018) (also see Panessa et al. 2011). Interestingly, asymmetric Balmer lines indicate an outflow with a velocity of ~500 km s$^{-1}$ but no such outflow component is seen in the forbidden lines, including [O III]$\lambda$5007 (Mullaney et al. 2013; Berton et al. 2016; Fig. B27). Citizen scientists using Galaxy Zoo identified this source as a candidate of having an extended emission line region based upon the SDSS imaging (Keel et al. 2012).

**Summary of radio properties:** We present our radio images for this source in Fig. B27. We observe an extended 'C' shaped structure in our L-band image, spanning several arcseconds to the southeast. Congiu et al. (2017) also obtained VLA observations

of this source at 5 GHz in A configuration and, they too, identified the extended curved radio structure (also confirmed by Berton et al. 2018). Congiu et al. (2017) measure a steep spectral index ($\alpha = -2.02$) for this radio structure, and use this to suggest that this emission is a relic from a past period of jet activity as seen in, e.g. NCG 4235 (Kharb et al. 2016). Alternatively, a strong interaction between a jet and the interstellar medium of the galaxy could result in greater radiative losses and a steep spectral index. In their lower resolution (tapered) image, Congiu et al. (2017) also identify extended radio emission up to a projected distance of 12.5 kpc in the northwest direction. This double-lobe shape resembles the radio emission seen in some Seyfert galaxies (e.g. Hota & Saikia 2006; Kharb et al. 2006).

In our ~0.3 arcsec resolution C-band image we only detect a featureless radio core (Fig. B27). Furthermore, Doi et al. (2013) used VLBI observations of the nucleus of this source and detected only a compact core with a measured brightness temperature of at least $7.7{\times}10^7$ K. These results indicate a non-thermal process driven by a central jet (see also Section 4.4). However, this core emission at 1.7 GHz represents only 4 percent of the total 1.4 GHz flux from NVSS indicating extensive extended radio emission that was resolved out in the VLBI observations. The source was undetected in the 22 GHz VLBI observations of Doi et al. (2016). In contrast, recent VLBI and e-MERLIN imaging for this source (Congiu et al. 2020) reveal a kpc jet-like structure, suggesting a precessing intermittent jet.

In agreement with our work, Congiu et al. (2017) also identify J1302+1624 as a radio excess source (Section 4.5). All of the evidence from our work presented here, and that presented in the literature, leads to our conclusion that this galaxy hosts a Radio-AGN.

## B28 J1316+1753

Due to the strongly double peaked [O III] emission line profile observed in the SDSS spectrum of this Type 2 radio-quiet source, it has been previously identified as a duel AGN candidate (Xu & Komossa 2009; Smith et al. 2010; Lyu & Liu 2016; Baron & Poznanski 2017; see Fig. B28). In Jarvis et al. (2020) we used CO(2–1) data and SED fitting to demonstrate that this source is consistent with being a gas rich star-forming galaxy. We previously presented GMOS IFS observations and radio imaging for this source in Harrison et al. (2014) and Jarvis et al. (2019). With our IFS observations, we noted that there were not two continuum peaks associated with the two [O III] emission-line components. Combined with the similarity of the emission-line ratios in both kinematic components, this suggests that these kinematic components may be illuminated by a single ionising source (also see Xu & Komossa 2009; Smith et al. 2010).

**Summary of radio and ionised gas properties:** We present the radio images used in this work in Fig. B28. The ~2 kpc radio jets identified in J1316+1753 appear to be co-spatial with the two [O III] kinematic components, favouring jet–ISM interactions as the origin of the double emission line peaks observed in the SDSS spectrum (Jarvis et al. 2019). Interestingly, Smith et al. (2010) find that radio-detected quasars are three times more likely to exhibit a double-peaked [O III] profile than quasars with no detected radio flux, in favour of jet interactions being important for double-peaked profiles across the population.

The identification of this source being a morphological 'triple' indicative of a jet is taken from the Gaussian fitting techniques from Jarvis et al. (2019) not the by eye classification employed in this work. Due to blending of the morphological features in the C-band data for this source the $64\sigma$ contour was used to calculate the core spectral index in Section 4.3. We note that the variations in methods between this work and Jarvis et al. (2019) results in quoted radio size measurements of 2.4 kpc and 1.4 kpc, respectively. Based upon the core and jet-like morphology of the radio emission (Fig. B28) and the hints of a flattening of the spectral index in the core (based on the analyses presented in Jarvis et al. 2019) we conclude that J1316+1753 contains a Radio-AGN.

## B29 J1324+5849

We present the radio images for this Type 1 source in Fig. B29.

**Summary of radio properties:** Based upon the criteria of Xu et al. (1999) this source is radio-quiet; however, based upon the criteria of Ivezić et al. (2002) it is on the boundary of radio-loudness ($R = 1.0$; see Section 2.4). Nonetheless, due to the featureless radio morphology and a lack of ancillary data, we are unable to confidently conclude that the radio emission is due to the AGN.

## B30 J1347+1217

This Type 2 radio-loud source,[1] is well studied and is commonly referred to as 4C+12.50 or PKS 1345+125. It has long been identified as undergoing a merger based on the identification of a ~2 arcsec separated double nucleus in optical and near infrared imaging data (Gilmore & Shaw 1986; Heckman et al. 1986; Shaw et al. 1992; Emonts et al. 2016). It is an ultraluminous IRAS galaxy, indicating high levels of star formation (Sanders et al. 1988; Evans et al. 1999), and the nuclear regions of the galaxy are gas rich based upon measurements of H I and CO (Mirabel et al. 1989; Mirabel 1989; Evans et al. 1999; Morganti et al. 2005b). The main radio source is coincident with the western, Type 2 nucleus (Stanghellini et al. 1997; Evans et al. 1999). This radio source is one of the GPS sources used to originally define the population (see e.g. O'Dea 1998; Stanghellini et al. 1998) and is associated with both an X-ray nucleus and extended X-ray bubble (O'Dea et al. 2000; Siemiginowska et al. 2008). All of the images considered directly in this work for this source are presented in Fig. B30.

**Summary of ionised gas properties:** This is source has the most extreme [O III] emission line width across our whole sample ($\mathrm{FWHM}_{[\mathrm{OIII}]}$ = 1730 km s$^{-1}$; see Fig. B30). The extreme ionised gas kinematics have been observed in several spectroscopic campaigns and likely trace a compact outflow (e.g. Grandi 1977; Gilmore & Shaw 1986; Holt et al. 2003, 2011; Tadhunter et al. 2018). Furthermore, it has an extended emission line region over 10 kpc in all directions, as traced by the [O III] emission (Holt et al. 2003). Outflows and gas heating are also observed through observations of neutral and molecular emission and absorption lines (Morganti et al. 2004, 2005a; Dasyra & Combes 2011, 2012; Dasyra et al. 2014; Guillard et al. 2012; Morganti et al. 2013; Spoon et al. 2013; Veilleux et al. 2013; Fotopoulou et al. 2019). These effects are likely caused by the compact radio jets interacting with the ISM (e.g. Batcheldor et al. 2007; Morganti et al. 2013; Fotopoulou et al. 2019).

**Summary of radio properties:** This source was not observed with the VLA as part of this project because of the extensive archival data available (it is a VLA calibrator source). Therefore, we use

[1] We note that this source is miss-classified as a Type 1 AGN in Mullaney et al. (2013).

archival images in the L- and C-band with A-configuration. Specifically, in the analysis for this work we use calibrated images from the NRAO VLA Archive Survey Images Pilot Page,[2] which are equivalent to the images we have used for the rest of the sample (see Table A1).[3]

Since these images do not contain spectral information, we calculate the core spectral index for this source in Section 4.3 between 3 and 4.85 GHz using the flux densities and errors from the The Very Large Array Sky Survey (3.827±0.018 Jy; Lacy et al. 2020) and the Green Bank 6 cm survey (3.11±0.28 Jy; Gregory et al. 1996) and assume this spectral slope continues linearly to ∼6GHz.

We observe no morphological features in any of the radio images used in this work. However, high resolution, multi-frequency radio imaging has revealed that J1347+1217 has a distorted, triple morphology aligned along a PA of 160° (e.g. Stanghellini et al. 1997). The brighter, superluminal precessing jet extends southeast, bending and expanding into a diffuse lobe and a bright knot towards the northern limit of the jet is tentatively identified as the core (Shaw et al. 1992; Stanghellini et al. 1997, 2001; Lister et al. 2003). Sensitive, low resolution observations reveal that there is additionally faint, diffuse radio emission extended across roughly 100 kpc in a roughly north-south direction (Stanghellini et al. 2005). The overall radio spectrum is typical of GPS radio spectrum, peaking at ∼0.6 GHz with a sharp spectral cut-off near 400 MHz (Stanghellini et al. 1998; Healey et al. 2007). We note that the radio size used throughout this work of 0.08 kpc, derived from the C-band image using CASA 'imfit' (Section 4.1), is roughly half the extent of the nuclear jets identified in previous works (i.e. ∼ 0.2 kpc; e.g. Stanghellini et al. 1997; O'Dea 1998). J1347+1217 is firmly classified as a Radio-AGN.

## B31 J1355+2046

We present the radio images for this Type 1 radio-quiet source in Fig. B31.

**Summary of radio properties:** J1355+2046 is unresolved in all but our C-band image where it shows a jet-like morphology extending to the south-east with an additional, lower significance jet-like extension to the north-west. This jet-like morphology caused us to use the 32$\sigma$ contour to calculate the core spectral index for this source in Section 4.3. Due to the lack of ancillary data for J1355+2046 however, we are unable to confirm an AGN origin for the radio emission.

## B32 J1356+1026

This Type 2 radio-quiet source is well studied in the literature. The [O III] emission-line profile in SDSS has inspired investigations into the possibility of this galaxy hosting a dual AGN (e.g. Liu et al. 2010a). Two merging galactic nuclei, with a projected separation of ∼2.5 kpc are seen in the optical and near-infrared (Fu et al. 2011, 2012; Shen et al. 2011; Greene et al. 2012). Spatially resolved spectroscopy shows distinct emission line ratios for these two nuclei and implies two distinct Type 2 AGN (Greene et al. 2012; Harrison et al. 2014). However, no radio emission has yet been associated with the secondary nucleus (Jarvis et al. 2019).

Spatially-resolved CO(1–0) and CO(3–2) data presented by Sun et al. (2014) reveal that the cold molecular gas is mostly distributed in a compact rotating disk, at the primary nucleus, with an extended tidal arm. They also find a compact ($r \approx 0.3$ kpc) high-velocity ($v \approx 500$ km s$^{-1}$) CO feature to the north of the nucleus, which they interpret as a likely molecular outflow. However, this is not associated with the giant ionised outflow located to the south of the nucleus. It is interesting to note that J1356+1026 was the only one of the nine targets, all of which are selected from the full sample present here, where Jarvis et al. (2020) noted any possible evidence for a reduced molecular gas supply compared the overall star-forming galaxy population (matched in stellar mass, redshift and star-formation rate). This was mostly based upon the non detection of CO(2–1) emission in our APEX data and the ALMA CO(1–0) flux measurement from Sun et al. (2014). Further work to measure robust molecular gas masses, trace the molecular gas kinematics and the star formation is required to firmly establish if this galaxy is in the process of being quenched by the observed outflows.

**Summary of ionised gas properties:** Using long-slit observations, Greene et al. (2012) (also see Greene et al. 2011) revealed [O III] emission extended over tens of kiloparsecs. In particular, they reveal a 'bubble' of [O III] emission with a spatial extent of 12 kpc to the south and high-velocity 'clumps' to the north. *Chandra* X-ray observations were presented by Greene et al. (2014) for J1356+1026. They detected soft X-ray emission in the region of the ionised outflowing bubble which could either be explained by the presence of a hot wind or by photoionized line emission (Greene et al. 2014; Stern et al. 2016). There is also evidence for a secondary X-ray point source in addition to the primary, more luminous nucleus (Comerford et al. 2015; Foord et al. 2020). Spatially-resolved *UV* emission spectroscopy was presented by Somalwar et al. (2020). Based upon the observed emission line ratios, which are similar from 100 pc to 10 kpc, they rule out the presence of a dynamically important hot wind and conclude that their best fit model of radiation pressure confined clouds is also consistent with the observed diffuse X-ray spectrum.

**Summary of radio properties:** We present the radio images used in this work for J1356+1026 in Fig. B32. These images do not show any morphological structures. Due to slight beam residuals in the C-band data for this source the 32$\sigma$ contour was used to calculate the core spectral index in Section 4.3. In Jarvis et al. (2019) we concatenated A-array and B-array, C-band VLA data to reveal a weak radio structure that extends ∼6 kpc south of the primary nucleus (see magenta contours in Fig. B32). Consequently, we measured a larger radio size of 5.6 kpc in Jarvis et al. (2019), compared to the 0.25 kpc presented here (measured in a consistent manner to the rest of the sample; Section 4.1). The extended radio structure terminates at the base of the outflowing bubble of ionised gas (Jarvis et al. 2019). The origin of this radio emission is yet to be established. J1356+1026 has significant excess emission above that expected from star formation (Section 4.5; also see; Harrison et al. 2014; Jarvis et al. 2019, 2020), and a high brightness temperature (see Section 4.4), therefore, we conclude an AGN origin of the radio emission.

## B33 J1430+1339

This radio-quiet Type 2 source is well studied in the literature. Using a citizen science campaign to search for extended emission-line regions in SDSS images, participants of the "Galaxy Zoo" project (Lintott et al. 2008) identified J1430+1339 as having an interesting extended emission line region morphology, with a loop shaped

[2] http://www.aoc.nrao.edu/~vlbacald/read.shtml
[3] Credit for both of these images goes to NRAO/VLA Archive Survey, (c) 2005-2009 AUI/NRAO.

"handle" of emission-line gas extending ~12 kpc to the northeast of the main galaxy (Keel et al. 2012; later confirmed by *HST* imaging; Keel et al. 2015). This work resulted in the nickname for this source as the "Teacup AGN" due to its morphological appearance in the SDSS imaging. The *HST* imaging also reveals that J1430+1339 resides in a bulge-dominated galaxy, with shell-like features, indicative of previous merger activity (Keel et al. 2015; Harrison et al. 2015). Our CO(2–1) observations and SED analyses demonstrate that J1430+1339 is consistent with being a gas rich star-forming galaxy (Jarvis et al. 2020).

X-ray observations by Lansbury et al. (2018) show that J1430+1339 contains a heavily obscured AGN ($N_{\rm H}$ = [4.2 − 6.5] × $10^{23}$ cm$^{-2}$) with an intrinsic luminosity of $L_{2-10\,\rm keV}$ = (0.8 − 1.4) × $10^{44}$ erg s$^{-1}$ (also see Oh et al. 2018). This robust measurement of the instantaneous luminosity challenges previous ideas that this source is a rapidly dying/fading quasar, which were based upon spatially-resolved analyses of spectroscopic data and emission line imaging and assumed a lower current bolometric luminosity (Gagne et al. 2014; Keel et al. 2017; Villar-Martín et al. 2018).

Using the high-resolution *Chandra* imaging, Lansbury et al. (2018) identified a loop of X-ray emission, co-spatial with the eastern bubble seen in the radio emission and ionized gas. The X-ray emission from this structure is in good agreement with shocked thermal gas, with $T \approx 10^6$ K, and there is evidence for a possible additional hot component with $T \approx 10^7$ K. Although the Teacup is a radiatively dominated AGN, the estimated ratio between the bubble power and the X-ray luminosity is in remarkable agreement with observations of ellipticals, groups, and clusters of galaxies undergoing AGN feedback due to powerful jets. Nonetheless, deeper X-ray observations are required for a more robust spectral and spatial analyses to confirm the origin of the extended X-ray emission.

**Summary of radio and ionised gas properties:** We present the radio images for J1430+1339 in Fig. B33. We previously studied our VLA radio images in detail in Harrison et al. (2015) and Jarvis et al. (2019). These works revealed "bubbles" of radio emission that are extended 10-12 kpc to both the east and west of the nucleus. The edge of the brighter eastern bubble is co-spatial with the loop of ionised emission-line gas described above. We also demonstrated the presence of a compact radio structure, located ~0.8 kpc from the core position, at the base of the eastern bubble. This radio structure is co-spatial with an [O III] outflow with an observed projected velocity of $v \approx -700$ km s$^{-1}$ that we identified in both our GMOS and VIMOS IFS data (Harrison et al. 2014, 2015). We inferred that this likely corresponds to a jet, or possibly a quasar wind, interacting with the interstellar medium at this position. We note that, in Jarvis et al. (2019) we used our VLA C-band image to measure the spatial extent of the radio emission (compared to using the A-array L-band image in this work). As shown by the white contours in Fig. B33, this image reveals more of the western radio bubble. Consequently, we measured a larger radio size of 19 kpc in Jarvis et al. (2019), compared to the 14 kpc presented here (determined using a consistent method to the rest of the sample; Section 4.1).

Near infrared IFS data presented by Ramos Almeida et al. (2017) confirmed the presence of nuclear, high velocity ionised gas through measurements of the hydrogen recombination lines (Pa$\alpha$, Br$\delta$ and Br$\gamma$) and also in the coronal line [Si VI]$\lambda$1.963$\mu$m. However, the narrow component of [Si VI] emission is redshifted with respect to the other lines, indicating that the coronal lines region is not co-spatial with the narrow-line region. In contrast to the ionised gas kinematics, Ramos Almeida et al. (2017) find that the warm molecular gas kinematics, as traced by the $H_2$ lines, appear to be dominated by galaxy rotation, with only a subtle hint of a ~50 km s$^{-1}$ blueshift in these emission lines. Deep long-slit observations obtained also reveal a diffuse extended emission line region out to a distance of ~100 kpc, way beyond the strong ~12 kpc emission-line loop (Villar-Martín et al. 2018).

J1430+1339 is classified as a radio excess source, with radio emission an order of magnitude higher than that expected from star formation alone (Section 4.5; also see Villar Martín et al. 2014; Harrison et al. 2014; Jarvis et al. 2019, 2020). Combined with the observed radio morphology, we conclude that radio emission from J1430+1339 is associated with an AGN.

## B34 J1436+4928

We present our radio images for this Type 2 radio-quiet source in Fig. B34.

**Summary of radio properties:** The radio data reveal no notable morphological features, but the C-band image contains steep-spectrum, marginally extended emission (LLS ≈ 800 pc). Due to a lack of ancillary data we are unable to confirm an AGN origin of the radio emission from J1454+0803.

## B35 J1454+0803

We present our radio images for this Type 1 radio-quiet source in Fig. B35.

**Summary of radio properties:** Our radio data reveal no notable morphological features, however the C-band emission is marginally extended with a size of 1.7 kpc. Due to a lack of ancillary data we are unable to confirm an AGN origin of the radio emission from J1454+0803.

## B36 J1509+1757

This source was detected at 60 $\mu$m and 100 $\mu$m by IRAS and consequently identified as a ULIRG, with spectroscopy confirming it hosts a Type 1 AGN (Zheng et al. 2002; Hao et al. 2005). Since then, it has been the subject of several follow-up studies, which have included detecting CO(1–0) with IRAM (Xia et al. 2012) and a campaign to search for OH Megamasers, which resulted in a non-detection (Darling & Giovanelli 2002; Chen et al. 2007; Zhang et al. 2014).

**Summary of radio properties:** We show the radio images used in this work for this source in Fig. B36. We identify two radio components, one associated with the main optical source and one associated with a secondary optical source located about 2.5 arcsec (i.e. ~7 kpc) to the northwest. We do not have optical spectroscopic data of the northern source; however, spatially-resolved CO data reveals that both components are CO(1–0) emitters, with comparable CO luminosities, at the same redshift (Tan et al. 2019). Tan et al. 2019 show that the two components are connected by a bridge of CO-emitting gas, further indicating this source is undergoing a merger. Although this source lies on the radio–infrared correlation of star-forming galaxies (see Section 4.5), it is also on the boundary of radio loudness based on the criteria of Ivezić et al. (2002), with $R$ = 1.0. Overall, we are unable to confirm an AGN origin of the radio emission from J1509+1757.

### B37 J1518+1403

This Type 2 radio-quiet source appears to be undergoing a merger, due to the optical source located about 13 kpc to the northeast of the primary target (Fig. B37). However, spectroscopy of the secondary source is required to firmly establish if these two sources are associated.

**Summary of radio properties:** Our radio images, presented in Fig. B37 also reveal that both optical sources have radio counterparts. The C-band image of the primary target shows slightly extended steep spectrum radio emission to the north of the nucleus. However, due to the lack of ancillary data, we are unable to confirm an AGN origin of the radio emission from J1518+1403.

### B38 J1553+4407

We present the radio images used in this work for this Type 2 radio-quiet source as an example in the main manuscript, Fig. 2.

**Summary of radio properties:** Since the C-band radio data for this source has no points with $>16\sigma$, the $8\sigma$ contour was used to calculate the core spectral index for this source in Section 4.3. This source shows a classical 'triple' morphology indicative of lobe – core – lobe structure from a radio jet in both our L and C-band data. The jet interpretation is further supported by the core showing a flat spectral index (−0.2). We therefore conclude an AGN origin of the radio emission from J1553+4407.

### B39 J1555+5403

We present the radio images used in this work for this Type 1 radio-quiet source in Fig. B38.

**Summary of radio properties:** J1555+5403 is unresolved in all but our C-band image where it reveals a jet-like structure extending towards the south-west, roughly aligned with the visible galactic disc in the optical image. If the extended radio emission observed originates from a jet / quasar wind driving into the disc this would provide a good explanation for the high velocities observed in the [O III] emission of this source (FWHM = 741 km $s^{-1}$). However, due to a lack of ancillary data, we are unable to confidently confirm an AGN origin of the radio emission from J1555+5403.

### B40 J1655+2146

We present the radio images used in this work for this Type 1 radio-quiet source in Fig. B39.

**Summary of radio and ionised gas properties:** We identify a steep spectrum jet-like radio structure in our C-band image, extending 1.8 kpc to the southwest. Due to the small separation of these components, the $64\sigma$ contour was used to calculate the core spectral index in Section 4.3. Husemann et al. (2013) presented optical integral field spectroscopy of this source. They do not see any evidence for extreme velocities in the galaxy-wide gas kinematics; however, they do identify asymmetric [O III] emission-line profiles close to the nucleus which they speculate could be due to jet–ISM interaction. Based on our data, the radio emission is extended along a PA of approximately 45° and extended over 0.7 arcsec (i.e. ∼1.8 kpc), which may be in favour of this idea. However, the alignment of this structure with the asymmetric [O III] emission needs to be tested with comparable spatial resolution integral field spectroscopy. Overall, we are unable to unambiguously confirm the AGN as the origin of the radio emission from J1655+2146.

### B41 J1701+2226

This Type 1 source is one of the few radio-loud AGN in our sample based upon both the Xu et al. (1999) and Ivezić et al. (2002) criteria (see Section 2.4). We show the radio images for this source in Fig. B40.

**Summary of radio properties:** The FIRST image reveals a structure located 19 kpc to the north-west consisting of a bright peak with diffuse structure curving up towards the north. We observe a similar morphology in our L-band image. The peak of the structure in the north-west is marginally detected in our C-band data, where it appears to be diffuse and not point-like. The central component of this source is resolved into a jet-like structure in our C-band image. The blending of these HR components caused us to use the $64\sigma$ contour to calculate the core spectral index in Section 4.3, revealing a flat spectrum core ($\alpha = -0.1$). A possible explanation for this is that this source contains a radio jet, the outer lobe of which is being swept back due to motion relative to an external medium (see e.g. Rudnick & Owen 1977). J1701+2226 is unambiguously a Radio-AGN.

### B42 J1715+6008

Due to the double peaked [O III] emission-line profile in the SDSS spectrum, with a velocity separation of 350 km $s^{-1}$ (Liu et al. 2010a; Smith et al. 2010; see Fig. B41), this radio-quiet Type 2 source has been the subject of several multi-wavelength studies to assess if it harbours a dual AGN (Fu et al. 2011; Comerford et al. 2011, 2012; Müller-Sánchez et al. 2015; Villforth & Hamann 2015; McGurk et al. 2015). Two sources are seen in both [O III] and X-rays that are separated by 0.7 arsec (i.e. ∼1.9 kpc; Comerford et al. 2011, 2012). However, deep optical imaging and adaptive optics assisted infrared imaging do not reveal a double nuclei or signs of a merger (Fu et al. 2011; Villforth & Hamann 2015; McGurk et al. 2015). We summarise the data used in this work for J1715+6008 in Fig. B41.

**Summary of radio and ionised gas properties:** This source shows no radio structures in our radio images, with only a compact steep spectrum core detected. Müller-Sánchez et al. (2015) studied this source using 8–12 GHz VLA observations with ∼0.2 arcsec resolution, combined with long-slit spectroscopy (that was originally presented in Comerford et al. 2012). The long-slit spectroscopy reveals that this source has a giant [O III] emitting region extending over about 11 arcsec (i.e. ∼30 kpc). The authors find that the radio emission has a steep spectrum and is extended along the same position angle (PA = 146°) as the [O III] emission, albeit on a much smaller scale of ∼0.1 arcsec. We note that this is in the same direction, but smaller than, the deconvolved radio size used in this work of 0.25 arcsec, possibly due to the higher resolution and/or higher frequency observations used in their work. The highest resolution radio image presented by Müller-Sánchez et al. (2015) also reveals two unresolved components that have a relatively flat spectral index and are separated by 0.1 arcsec, with the secondary peak in the southeast of the core.

Although along the same position angle, the radio structures identified by Müller-Sánchez et al. (2015) are not spatially coincident with the location of the two spatially distinct components seen in [O III] and X-rays. Müller-Sánchez et al. (2015) conclude that this source contains a one-sided radio jet that is driving an [O III] outflow, countering previous ideas that this was one of the best dual AGN candidates (e.g. Comerford et al. 2011, 2012; Wang & Zhou 2012). Indeed, the similar intensities of the two [O III] emission-line components and the fact that the gas kinematics do not trace that of

the stellar kinematics, also favours a jet-driven outflow origin over a dual AGN origin of the double peaked [O III] profile (Smith et al. 2012; Villforth & Hamann 2015). We use the archival observations to conclude that J1715+6008 hosts a Radio-AGN.

## REFERENCES


Baron D., Poznanski D., 2017, MNRAS, 465, 4530
Barrows R. S., Comerford J. M., Greene J. E., Pooley D., 2017, ApJ, 838, 129
Batcheldor D., Tadhunter C., Holt J., Morganti R., O'Dea C. P., Axon D. J., Koekemoer A., 2007, ApJ, 661, 70
Berton M., Foschini L., Ciroi S., Cracco V., La Mura G., Di Mille F., Rafanelli P., 2016, A&A, 591, A88
Berton M., et al., 2018, A&A, 614, A87
Bondi M., Pérez-Torres M. A., Piconcelli E., Fu H., 2016, A&A, 588, A102
Chen P. S., Shan H. G., Gao Y. F., 2007, AJ, 133, 496
Comerford J. M., Greene J. E., 2014, ApJ, 789, 112
Comerford J. M., Pooley D., Gerke B. F., Madejski G. M., 2011, ApJ, 737, L19
Comerford J. M., Gerke B. F., Stern D., Cooper M. C., Weiner B. J., Newman J. A., Madsen K., Barrows R. S., 2012, ApJ, 753, 42
Comerford J. M., Pooley D., Barrows R. S., Greene J. E., Zakamska N. L., Madejski G. M., Cooper M. C., 2015, ApJ, 806, 219
Congiu E., et al., 2017, A&A, 603, A32
Congiu E., et al., 2020, arXiv e-prints, p. arXiv:2009.13529
Cui J., Xia X. Y., Deng Z. G., Mao S., Zou Z. L., 2001, AJ, 122, 63
Darling J., Giovanelli R., 2002, AJ, 124, 100
Dasyra K. M., Combes F., 2011, A&A, 533, L10
Dasyra K. M., Combes F., 2012, A&A, 541, L7
Dasyra K. M., Combes F., Novak G. S., Bremer M., Spinoglio L., Pereira Santaella M., Salomé P., Falgarone E., 2014, A&A, 565, A46
Doi A., Asada K., Fujisawa K., Nagai H., Hagiwara Y., Wajima K., Inoue M., 2013, ApJ, 765, 69
Doi A., Oyama T., Kono Y., Yamauchi A., Suzuki S., Matsumoto N., Tazaki F., 2016, PASJ, 68, 73
Emonts B. H. C., Morganti R., Villar-Martín M., Hodgson J., Brogt E., Tadhunter C. N., Mahony E., Oosterloo T. A., 2016, A&A, 596, A19
Evans A. S., Kim D. C., Mazzarella J. M., Scoville N. Z., Sanders D. B., 1999, ApJ, 521, L107
Fischer T. C., et al., 2018, ApJ, 856, 102
Foord A., Gültekin K., Nevin R., Comerford J. M., Hodges-Kluck E., Barrows R. S., Goulding A. D., Greene J. E., 2020, ApJ, 892, 29
Fotopoulou C. M., Dasyra K. M., Combes F., Salomé P., Papachristou M., 2019, A&A, 629, A30
Fu H., Myers A. D., Djorgovski S. G., Yan L., 2011, ApJ, 733, 103
Fu H., Yan L., Myers A. D., Stockton A., Djorgovski S. G., Aldering G., Rich J. A., 2012, ApJ, 745, 67
Gagne J. P., et al., 2014, ApJ, 792, 72
Gilmore G., Shaw M. A., 1986, Nature, 321, 750
Goulding A. D., Pardo K., Greene J. E., Mingarelli C. M. F., Nyland K., Strauss M. A., 2019, ApJ, 879, L21
Gower J. F. R., Scott P. F., Wills D., 1967, Mem. RAS, 71, 49
Grandi S. A., 1977, ApJ, 215, 446
Greene J. E., Zakamska N. L., Ho L. C., Barth A. J., 2011, ApJ, 732, 9
Greene J. E., Zakamska N. L., Smith P. S., 2012, ApJ, 746, 86
Greene J. E., Pooley D., Zakamska N. L., Comerford J. M., Sun A.-L., 2014, ApJ, 788, 54
Gregory P. C., Scott W. K., Douglas K., Condon J. J., 1996, ApJS, 103, 427
Guillard P., et al., 2012, ApJ, 747, 95
Hainline K. N., Hickox R., Greene J. E., Myers A. D., Zakamska N. L., 2013, ApJ, 774, 145
Hao C. N., Xia X. Y., Mao S., Wu H., Deng Z. G., 2005, ApJ, 625, 78
Harrison C. M., Alexander D. M., Mullaney J. R., Swinbank A. M., 2014, MNRAS, 441, 3306
Harrison C. M., Thomson A. P., Alexander D. M., Bauer F. E., Edge A. C., Hogan M. T., Mullaney J. R., Swinbank A. M., 2015, ApJ, 800, 45
Healey S. E., Romani R. W., Taylor G. B., Sadler E. M., Ricci R., Murphy T., Ulvestad J. S., Winn J. N., 2007, ApJS, 171, 61
Heckman T. M., Smith E. P., Baum S. A., van Breugel W. J. M., Miley G. K., Illingworth G. D., Bothun G. D., Balick B., 1986, ApJ, 311, 526
Holt J., Tadhunter C. N., Morganti R., 2003, MNRAS, 342, 227
Holt J., Tadhunter C. N., Morganti R., Emonts B. H. C., 2011, MNRAS, 410, 1527
Hota A., Saikia D. J., 2006, MNRAS, 371, 945
Hovatta T., et al., 2014, MNRAS, 439, 690
Husemann B., Wisotzki L., Sánchez S. F., Jahnke K., 2013, A&A, 549, A43
Ivezić Ž., et al., 2002, AJ, 124, 2364
Jarvis M. E., et al., 2019, MNRAS, 485, 2710
Jarvis M. E., et al., 2020, MNRAS, 498, 1560
Jimenez-Gallardo A., et al., 2019, A&A, 627, A108
Kang D., Woo J.-H., 2018, ApJ, 864, 124
Keel W. C., et al., 2012, MNRAS, 420, 878
Keel W. C., et al., 2015, AJ, 149, 155
Keel W. C., et al., 2017, ApJ, 835, 256
Kharb P., O'Dea C. P., Baum S. A., Colbert E. J. M., Xu C., 2006, ApJ, 652, 177
Kharb P., Srivastava S., Singh V., Gallimore J. F., Ishwara-Chandra C. H., Ananda H., 2016, MNRAS, 459, 1310
Kim D. C., Sanders D. B., Veilleux S., Mazzarella J. M., Soifer B. T., 1995, ApJS, 98, 129
Lacy M., et al., 2020, PASP, 132, 035001
Lansbury G. B., Jarvis M. E., Harrison C. M., Alexander D. M., Del Moro A., Edge A. C., Mullaney J. R., Thomson A. P., 2018, ApJ, 856, L1
Lintott C. J., et al., 2008, MNRAS, 389, 1179
Lister M. L., Kellermann K. I., Vermeulen R. C., Cohen M. H., Zensus J. A., Ros E., 2003, ApJ, 584, 135
Liu X., Shen Y., Strauss M. A., Greene J. E., 2010a, ApJ, 708, 427
Liu X., Greene J. E., Shen Y., Strauss M. A., 2010b, ApJ, 715, L30
Liu X., Shen Y., Strauss M. A., Hao L., 2011, ApJ, 737, 101
Liu X., Civano F., Shen Y., Green P., Greene J. E., Strauss M. A., 2013, ApJ, 762, 110
Liu X., Lazio T. J. W., Shen Y., Strauss M. A., 2018, ApJ, 854, 169
Lyu Y., Liu X., 2016, MNRAS, 463, 24
Massaro F., D'Abrusco R., Tosti G., Ajello M., Paggi A., Gasparrini D., 2012, ApJ, 752, 61
McGurk R. C., Max C. E., Medling A. M., Shields G. A., Comerford J. M., 2015, ApJ, 811, 14
Mirabel I. F., 1989, ApJ, 340, L13
Mirabel I. F., Sanders D. B., Kazes I., 1989, ApJ, 340, L9
Morganti R., Oosterloo T. A., Tadhunter C. N., Vermeulen R., Pihlström Y. M., van Moorsel G., Wills K. A., 2004, A&A, 424, 119
Morganti R., Oosterloo T. A., Tadhunter C. N., van Moorsel G., Emonts B., 2005a, A&A, 439, 521
Morganti R., Tadhunter C. N., Oosterloo T. A., 2005b, A&A, 444, L9
Morganti R., Fogasy J., Paragi Z., Oosterloo T., Orienti M., 2013, Science, 341, 1082
Mullaney J. R., Alexander D. M., Fine S., Goulding A. D., Harrison C. M., Hickox R. C., 2013, MNRAS, 433, 622
Müller-Sánchez F., Comerford J. M., Nevin R., Barrows R. S., Cooper M. C., Greene J. E., 2015, ApJ, 813, 103
Nardini E., Risaliti G., Watabe Y., Salvati M., Sani E., 2010, MNRAS, 405, 2505
Nolan P. L., et al., 2012, ApJS, 199, 31
O'Dea C. P., 1998, PASP, 110, 493
O'Dea C. P., De Vries W. H., Worrall D. M., Baum S. A., Koekemoer A., 2000, AJ, 119, 478
Oh K., et al., 2018, ApJS, 235, 4
Osterbrock D. E., Pogge R. W., 1985, ApJ, 297, 166
Panessa F., et al., 2011, MNRAS, 417, 2426
Ramos Almeida C., Piqueras López J., Villar-Martín M., Bessiere P. S., 2017, MNRAS, 470, 964
Rudnick L., Owen F. N., 1977, AJ, 82, 1
Sanders D. B., Soifer B. T., Elias J. H., Neugebauer G., Matthews K., 1988, ApJ, 328, L35

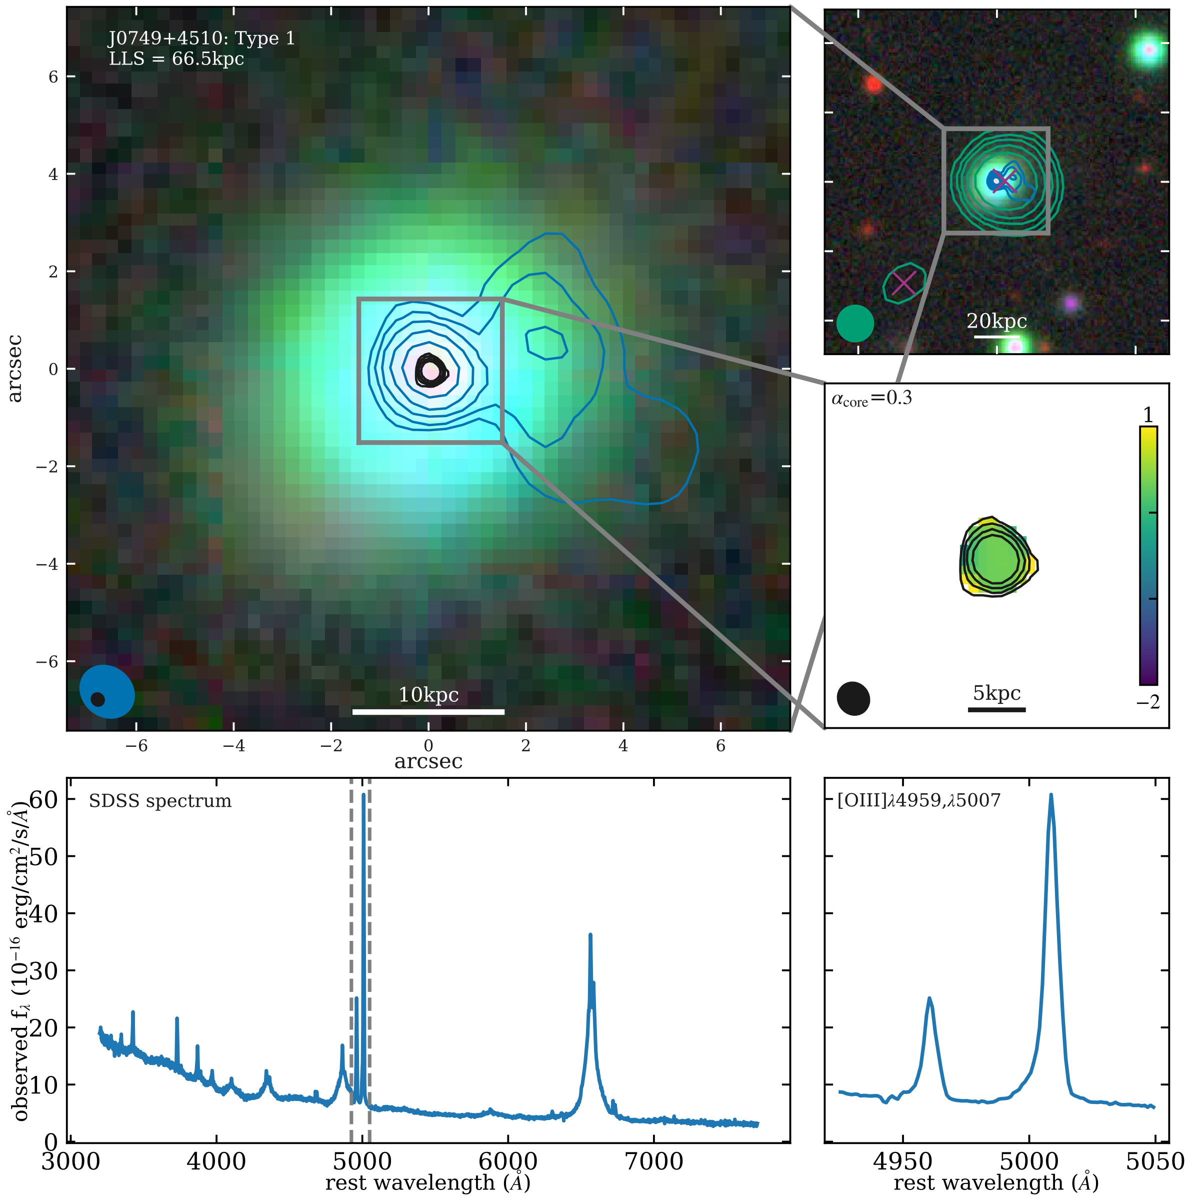


**Figure B1.** As Fig. 2 but for J0749+4510. Radio contours are plotted at ±[8, 16, 32, 64, 128]$\sigma$ in FIRST and our L-band image and at ±[16, 32, 64, 128]$\sigma$ for the C-band data.


Sargsyan L., Mickaelian A., Weedman D., Houck J., 2008, ApJ, 683, 114

Shangguan J., Liu X., Ho L. C., Shen Y., Peng C. Y., Greene J. E., Strauss M. A., 2016, ApJ, 823, 50

Shaw M. A., Tzioumis A. K., Pedlar A., 1992, MNRAS, 256, 6P

Shen Y., Liu X., Greene J. E., Strauss M. A., 2011, ApJ, 735, 48

Siemiginowska A., LaMassa S., Aldcroft T. L., Bechtold J., Elvis M., 2008, ApJ, 684, 811

Smith K. L., Shields G. A., Bonning E. W., McMullen C. C., Rosario D. J., Salviander S., 2010, ApJ, 716, 866

Smith K. L., Shields G. A., Salviander S., Stevens A. C., Rosario D. J., 2012, ApJ, 752, 63

Somalwar J., Johnson S. D., Stern J., Goulding A. D., Greene J. E., Zakamska N. L., Alexandroff R. M., Chen H.-W., 2020, ApJ, 890, L28

Spoon H. W. W., et al., 2013, ApJ, 775, 127

Stanghellini C., O'Dea C. P., Baum S. A., Dallacasa D., Fanti R., Fanti C., 1997, A&A, 325, 943

Stanghellini C., O'Dea C. P., Dallacasa D., Baum S. A., Fanti R., Fanti C., 1998, A&AS, 131, 303

Stanghellini C., Dallacasa D., O'Dea C. P., Baum S. A., Fanti R., Fanti C., 2001, A&A, 377, 377

Stanghellini C., O'Dea C. P., Dallacasa D., Cassaro P., Baum S. A., Fanti R., Fanti C., 2005, A&A, 443, 891

Stern J., Faucher-Giguère C.-A., Zakamska N. L., Hennawi J. F., 2016, ApJ, 819, 130

Storchi-Bergmann T., et al., 2018, ApJ, 868, 14

Sun A.-L., Greene J. E., Zakamska N. L., Nesvadba N. P. H., 2014, ApJ, 790, 160

Sun A.-L., Greene J. E., Zakamska N. L., 2017, ApJ, 835, 222

Tadhunter C., et al., 2018, MNRAS, 478, 1558

Tan Q.-H., et al., 2019, ApJ, 887, 24

Trindade Falcao A., et al., 2020, arXiv e-prints, p. arXiv:2010.08050

Veilleux S., Kim D. C., Sanders D. B., Mazzarella J. M., Soifer B. T., 1995,

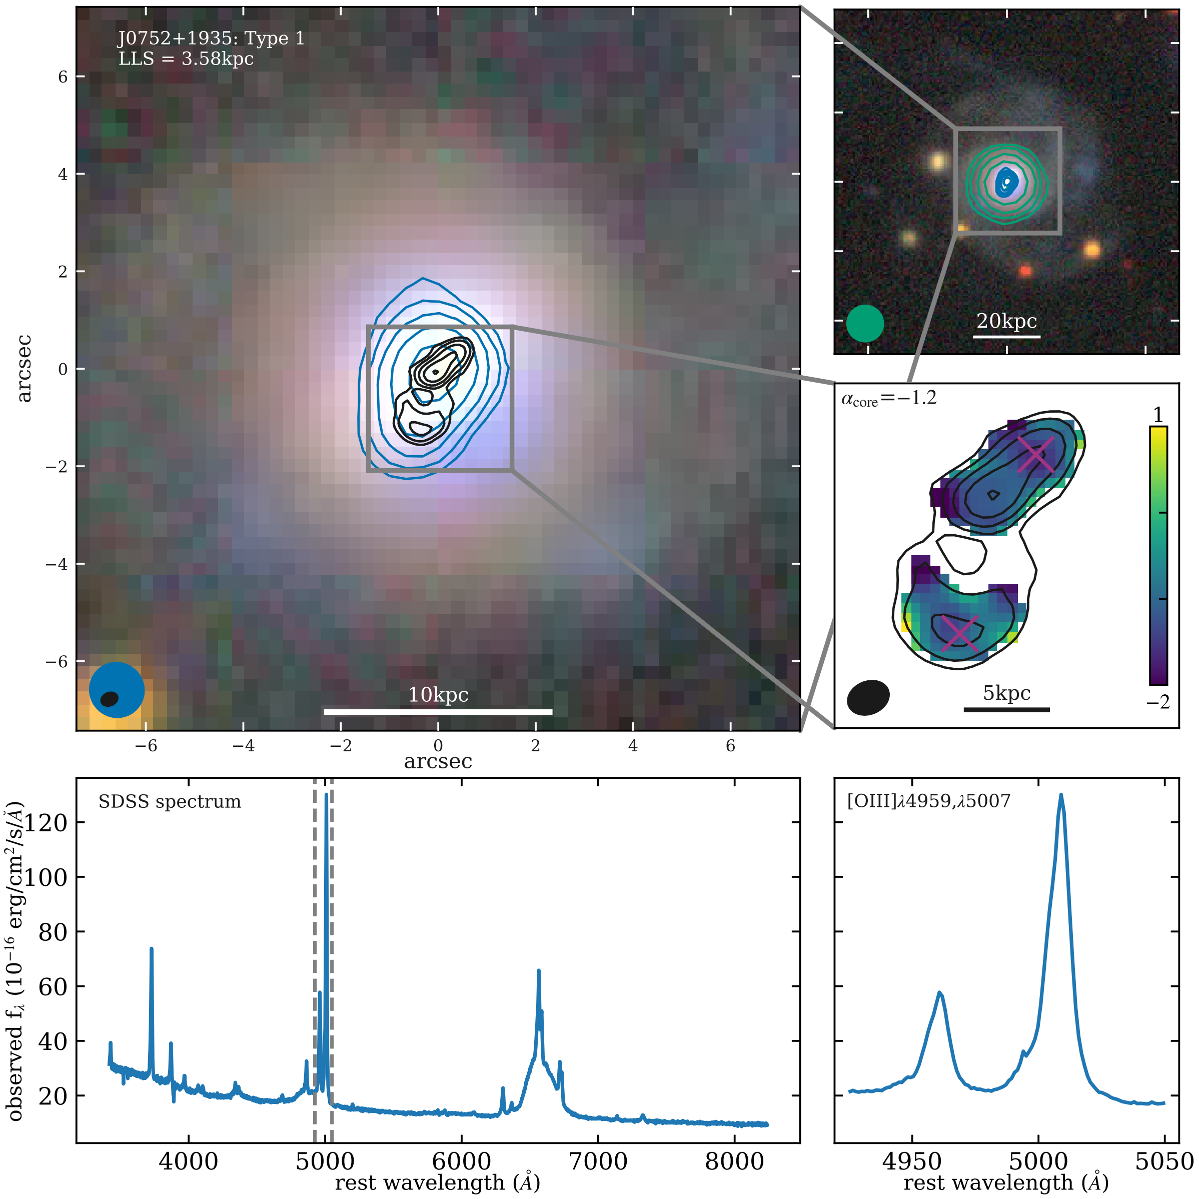


**Figure B2.** As Fig. 2 but for J0752+1935. Radio contours for all data are plotted at ±[8, 16, 32, 64, 128]$\sigma$.


ApJS, 98, 171
Veilleux S., et al., 2013, ApJ, 776, 27
Villar Martín M., Emonts B., Humphrey A., Cabrera Lavers A., Binette L., 2014, MNRAS, 440, 3202
Villar-Martín M., Cabrera-Lavers A., Humphrey A., Silva M., Ramos Almeida C., Piqueras-López J., Emonts B., 2018, MNRAS, 474, 2302
Villforth C., Hamann F., 2015, AJ, 149, 92
Wang X. W., Zhou H. Y., 2012, ApJ, 757, 124
Xia X. Y., et al., 2012, ApJ, 750, 92
Xu D., Komossa S., 2009, ApJ, 705, L20
Xu C., Livio M., Baum S., 1999, AJ, 118, 1169
Zhang J. S., Wang J. Z., Di G. X., Zhu Q. F., Guo Q., Wang J., 2014, A&A, 570, A110
Zhao Y., Yan L., Tsai C.-W., 2016, ApJ, 824, 146
Zhao D., Ho L. C., Zhao Y., Shangguan J., Kim M., 2019, ApJ, 877, 52
Zheng X. Z., Xia X. Y., Mao S., Wu H., Deng Z. G., 2002, AJ, 124, 18


This paper has been typeset from a TEX/LATEX file prepared by the author.

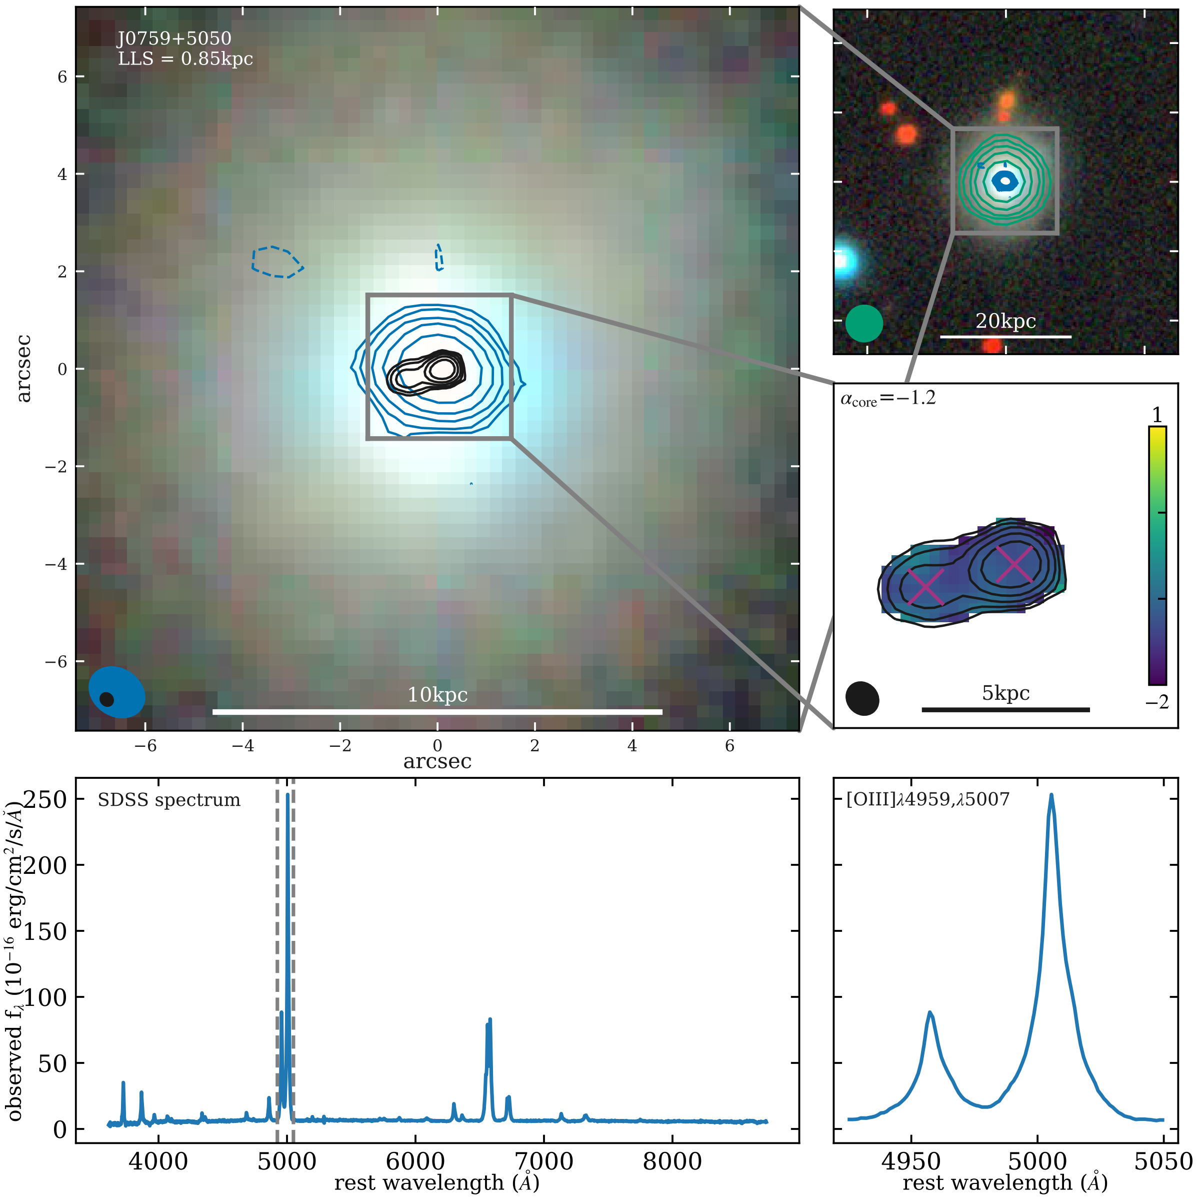


**Figure B3.** As Fig. 2 but for J0759+5050. Radio contours for all data are plotted at ±[8, 16, 32, 64, 128]$\sigma$.

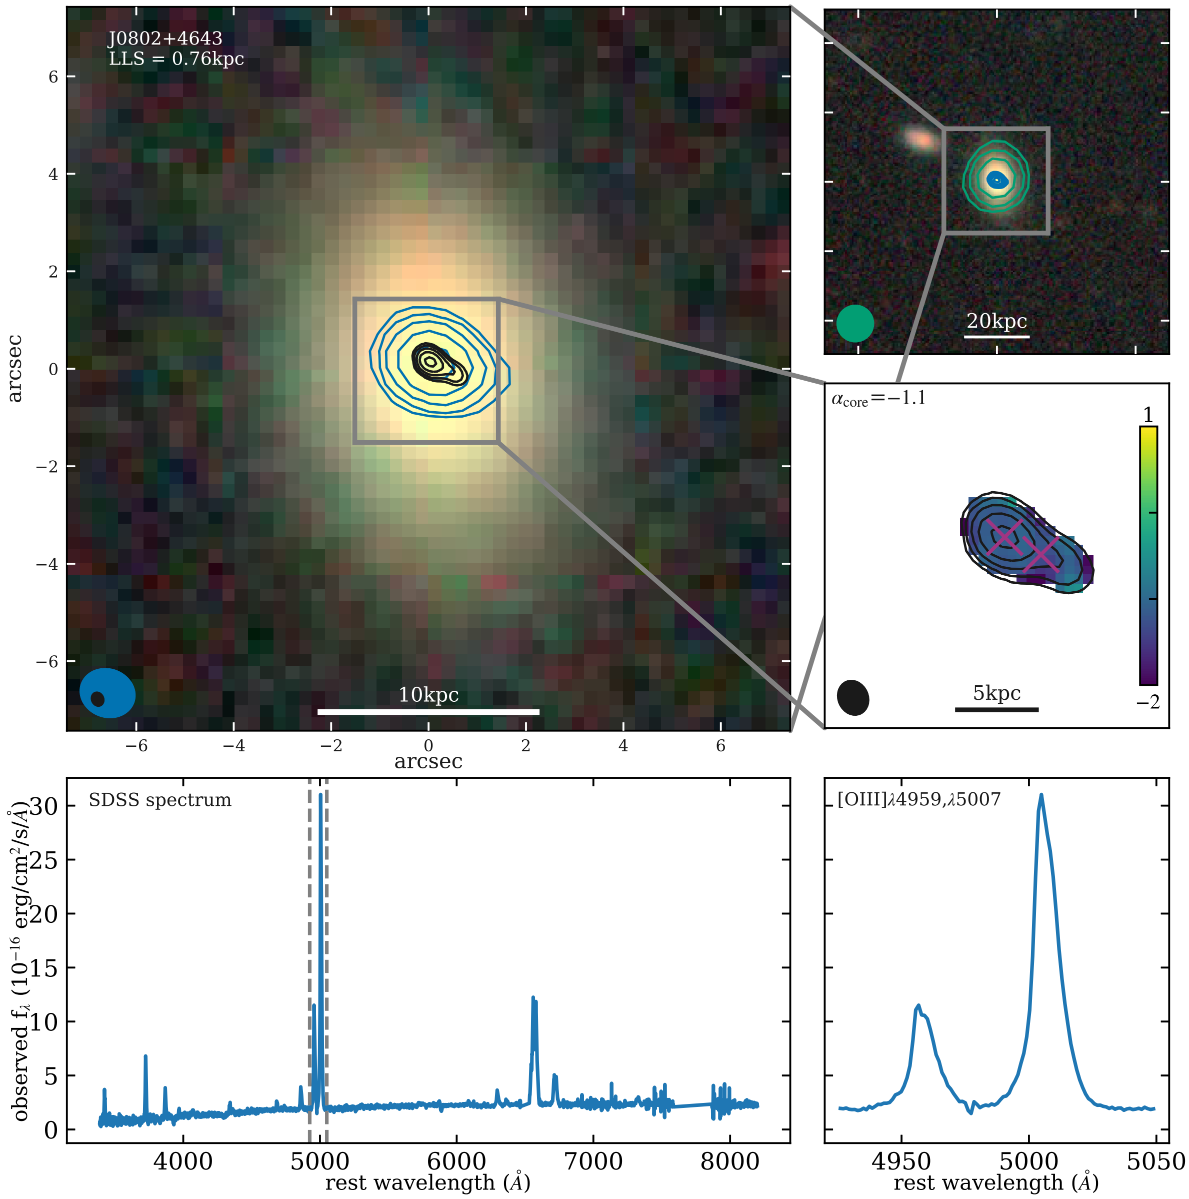


**Figure B4.** As Fig. 2 but for J0802+4643. Radio contours for all data are plotted at ±[8, 16, 32, 64, 128]$\sigma$.

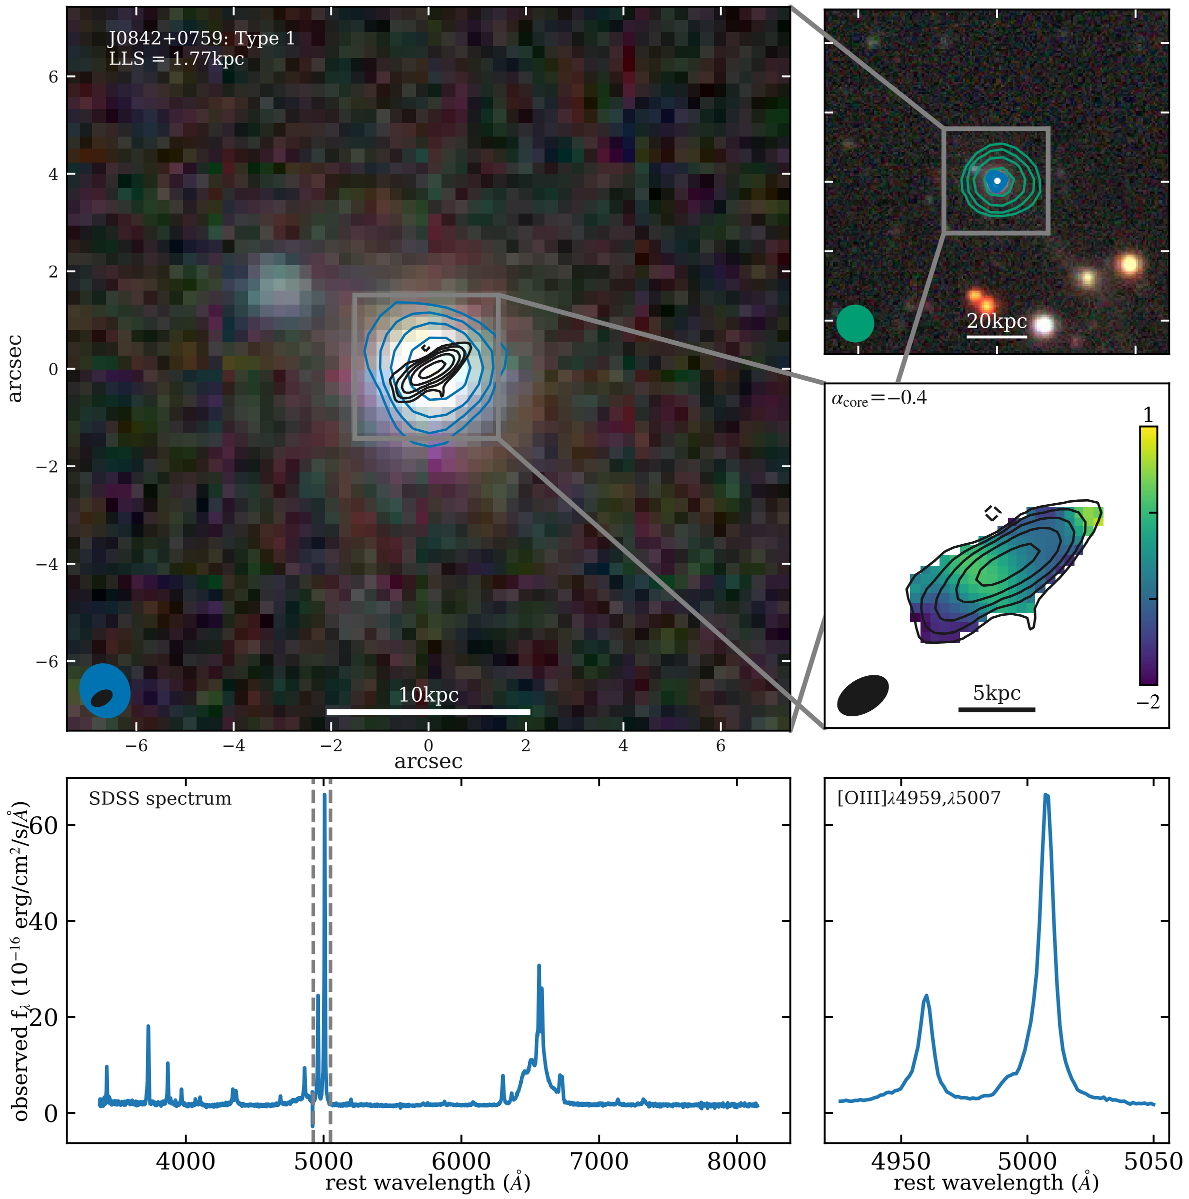


**Figure B5.** As Fig. 2 but for J0842+0759. Radio contours for all data are plotted at ±[8, 16, 32, 64, 128]$\sigma$. We note that the spectral index measured for this source (−0.4) is dominated by the visible flattening of the spectral index map, shown here, just to the south-east of the peak of the radio emission.

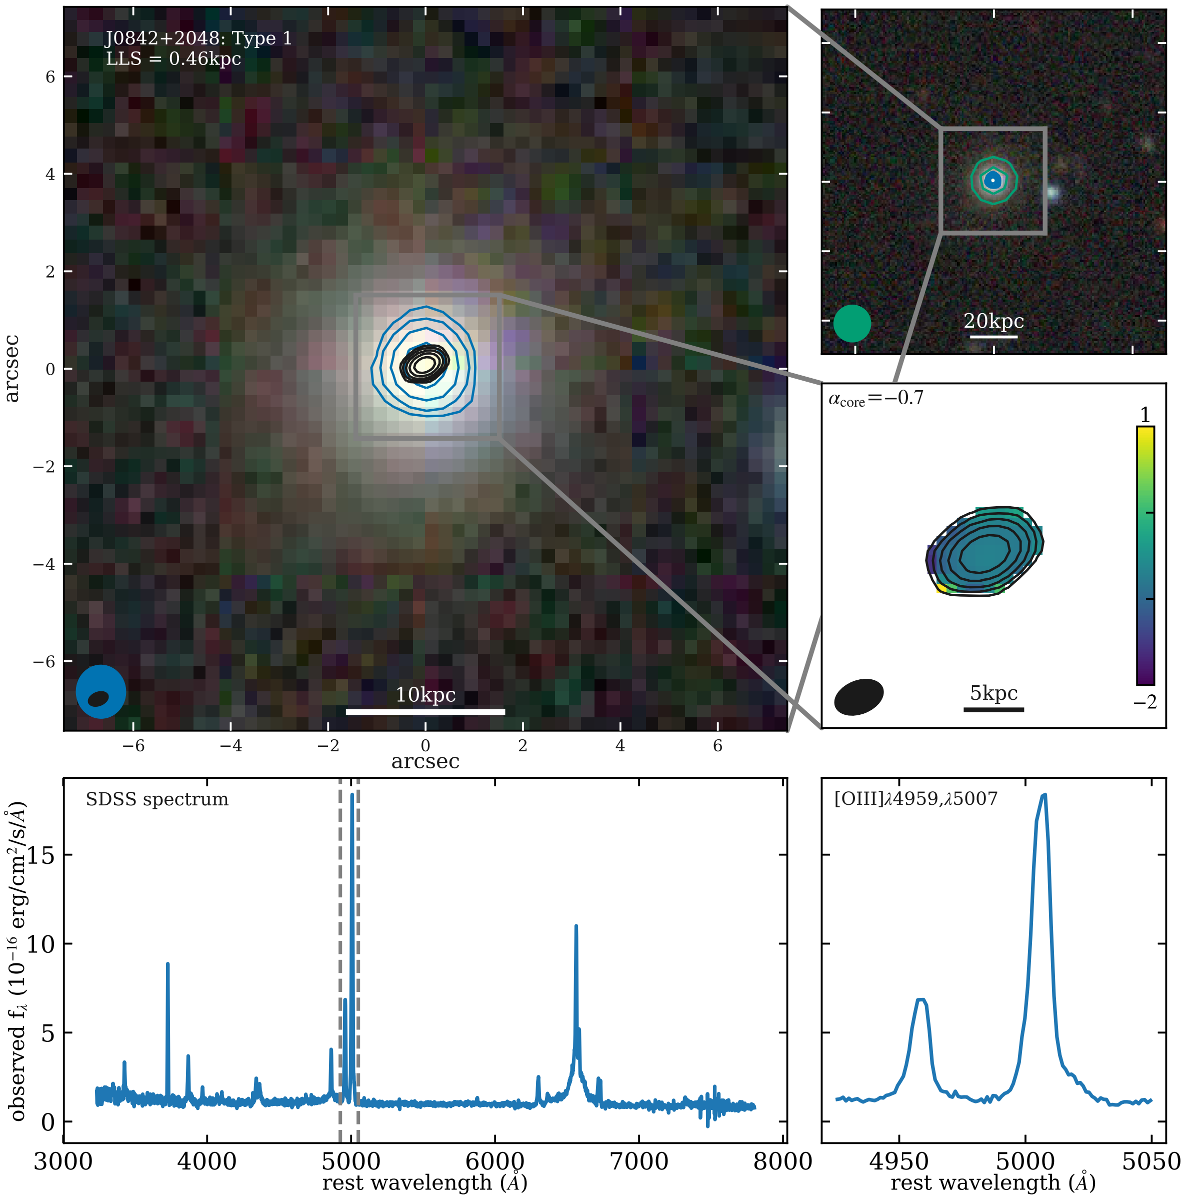


**Figure B6.** As Fig. 2 but for J0842+2048. Radio contours for all data are plotted at ±[8, 16, 32, 64, 128]$\sigma$.

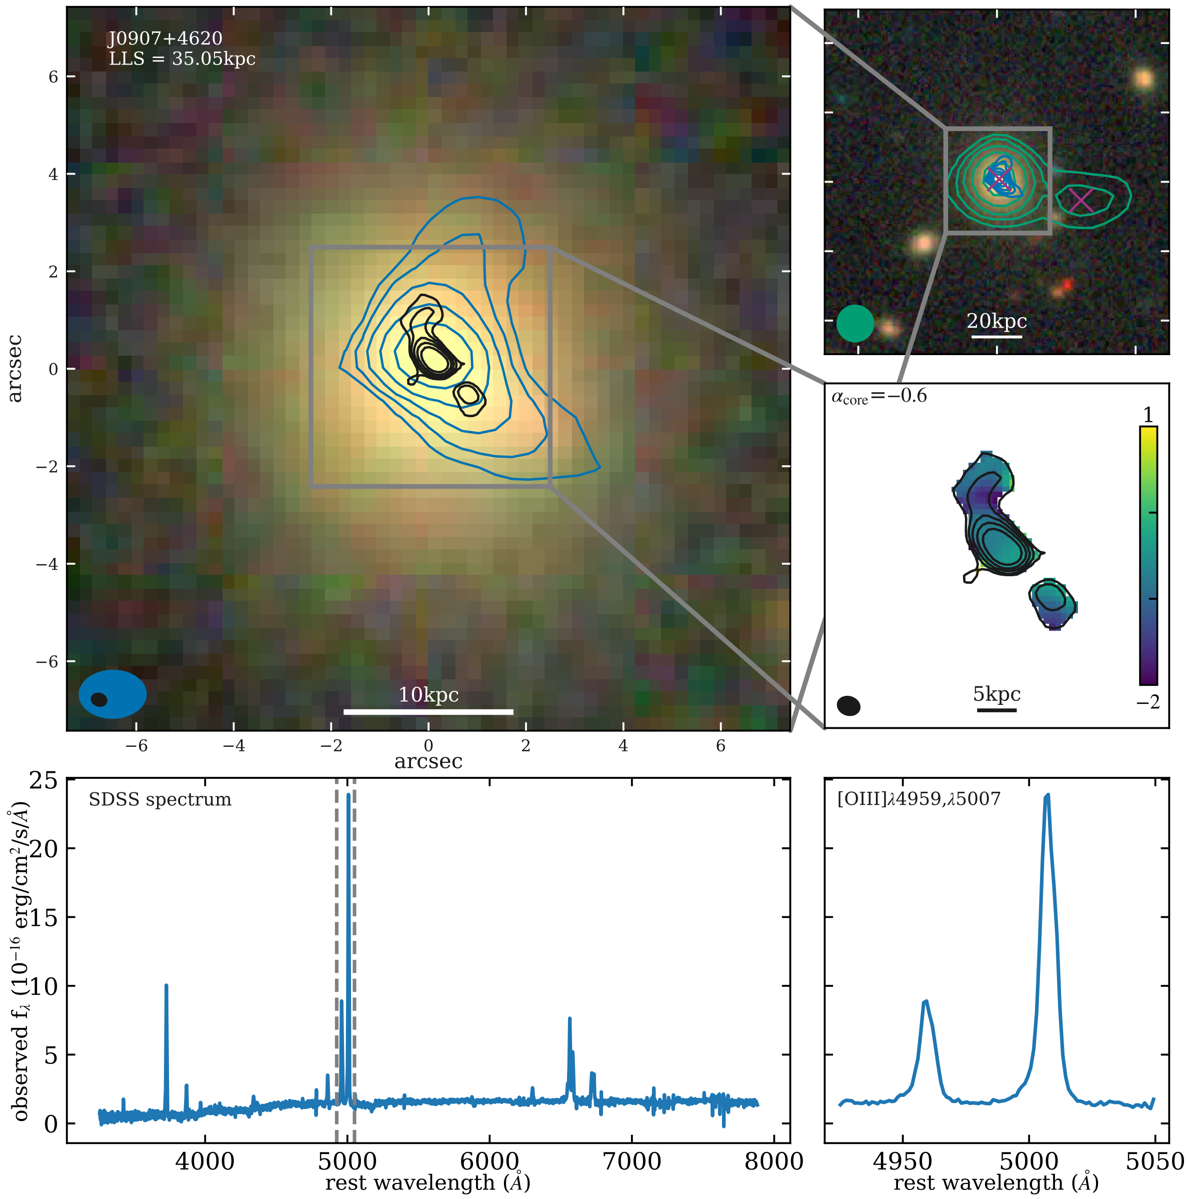


**Figure B7.** As Fig. 2 but for J0907+4620. Radio contours for all data are plotted at ±[8, 16, 32, 64, 128]$\sigma$. We note that the FIRST image reveals a lobe like feature 35 kpc to the west, which is used to measure the largest linear size of this source (see magenta crosses).

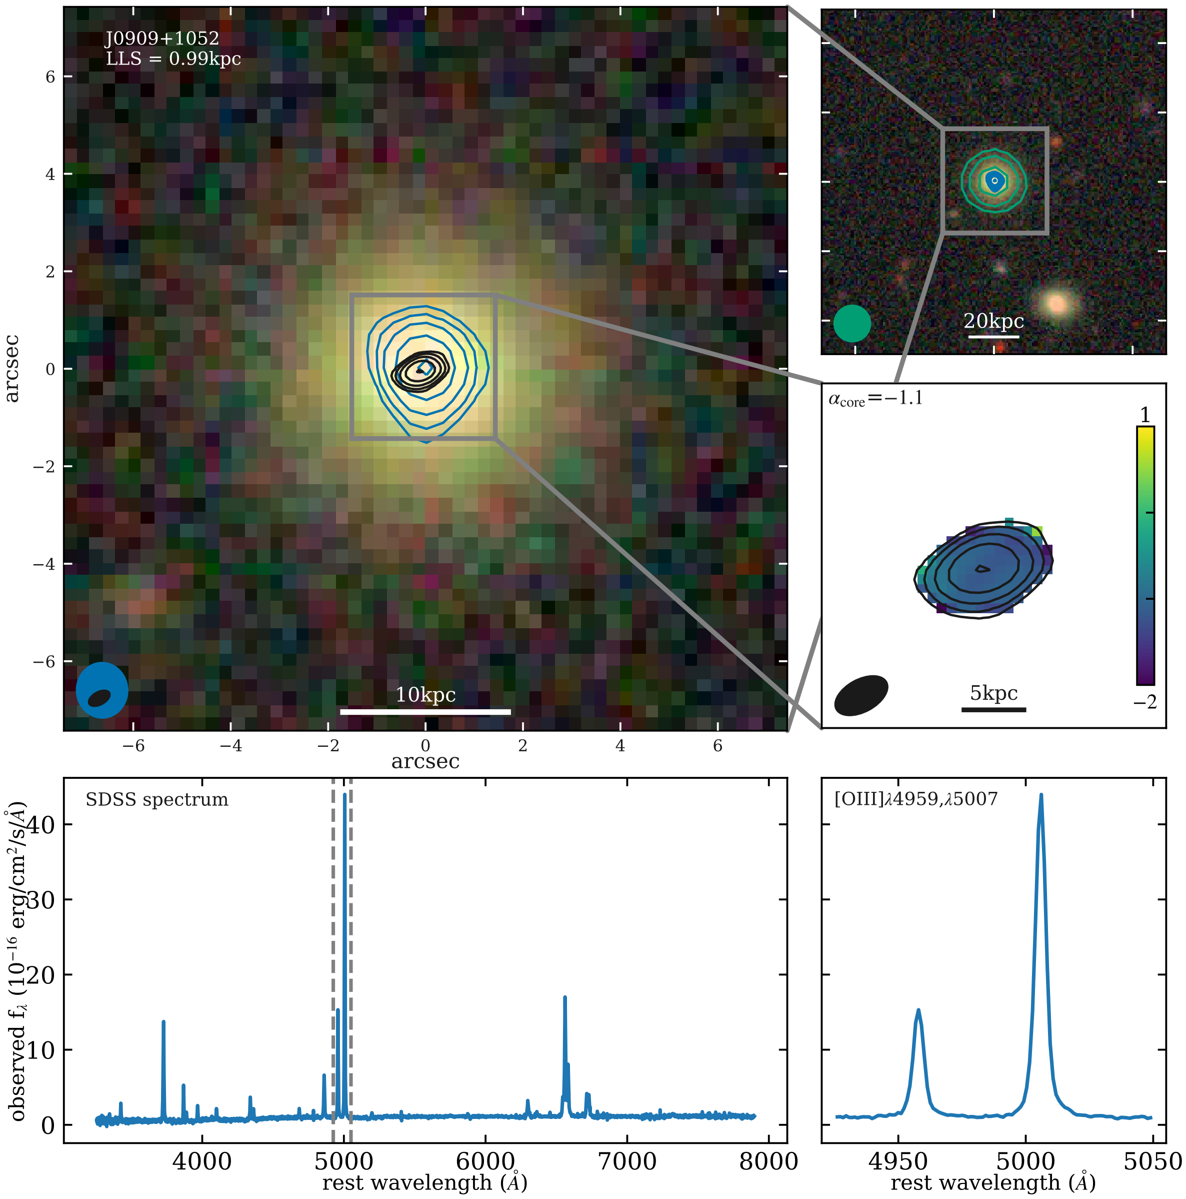


**Figure B8.** As Fig. 2 but for J0909+1052. Radio contours for all data are plotted at ±[8, 16, 32, 64, 128]$\sigma$.

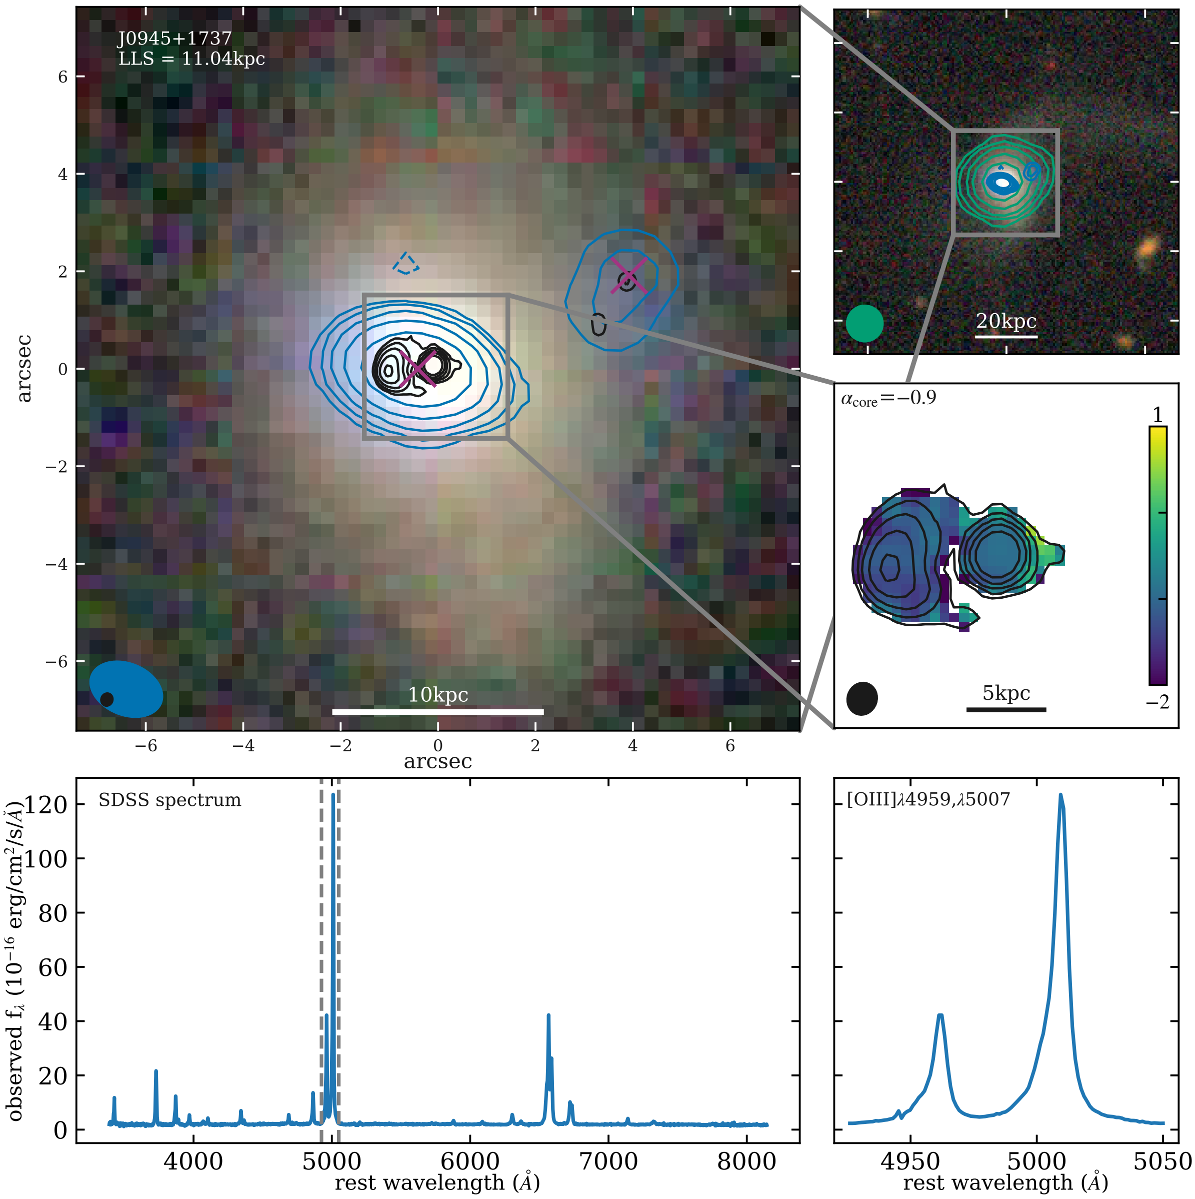


**Figure B9.** As Fig. 2 but for J0945+1737. Radio contours for all data are plotted at ±[8, 16, 32, 64, 128]$\sigma$.

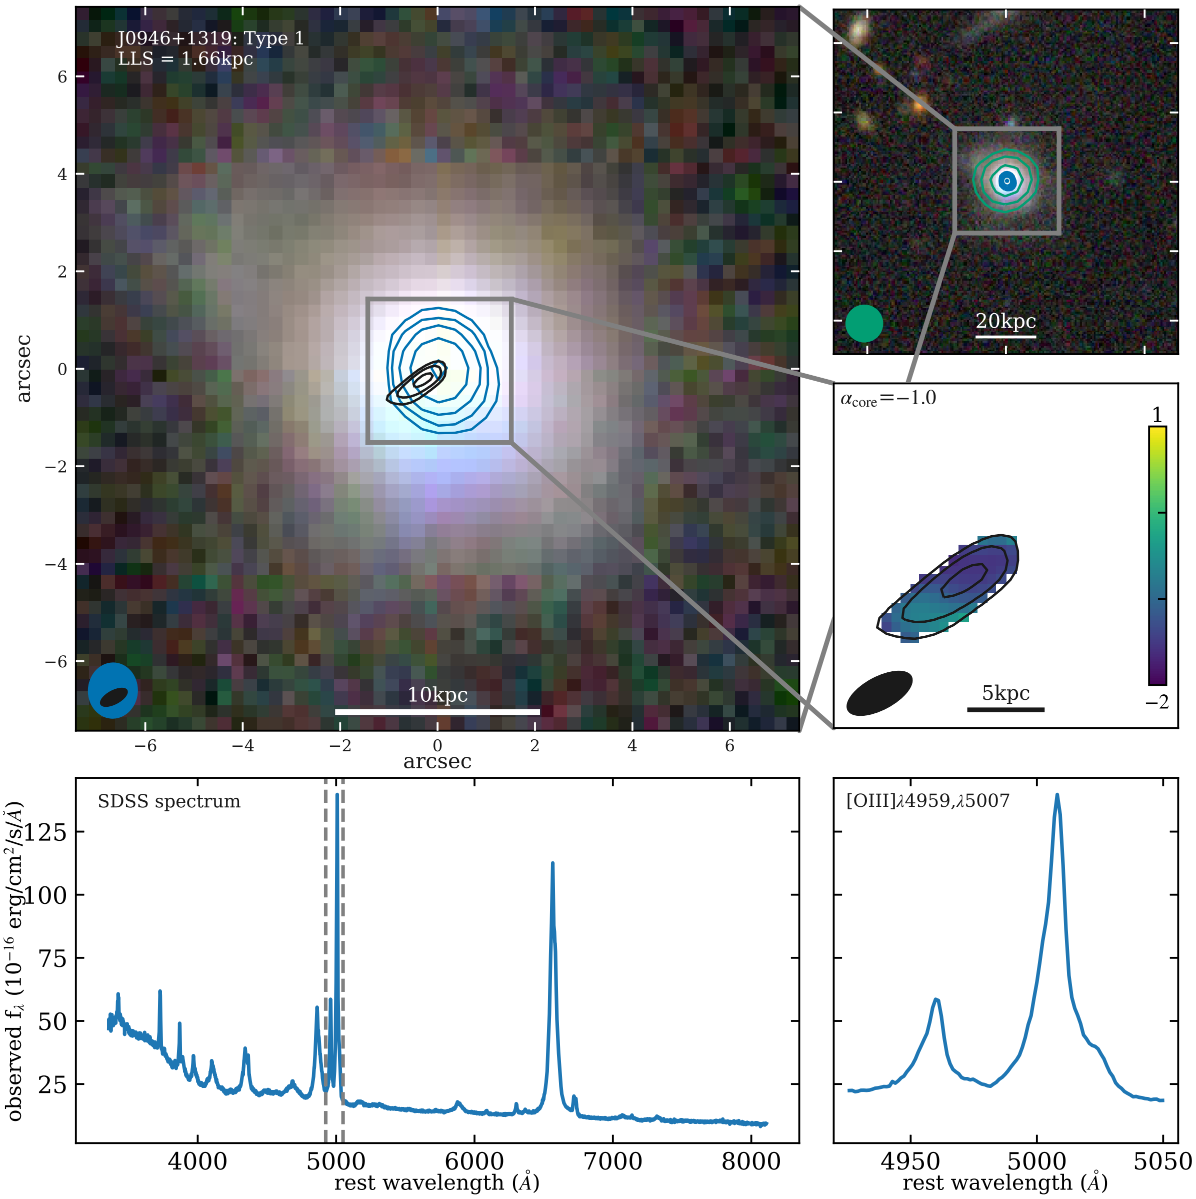


**Figure B10.** As Fig. 2 but for J0946+1319. Radio contours are plotted at ±[8, 16, 32, 64, 128]$\sigma$ in FIRST and our L-band image and at ±[16, 32, 64, 128]$\sigma$ for the C-band data.

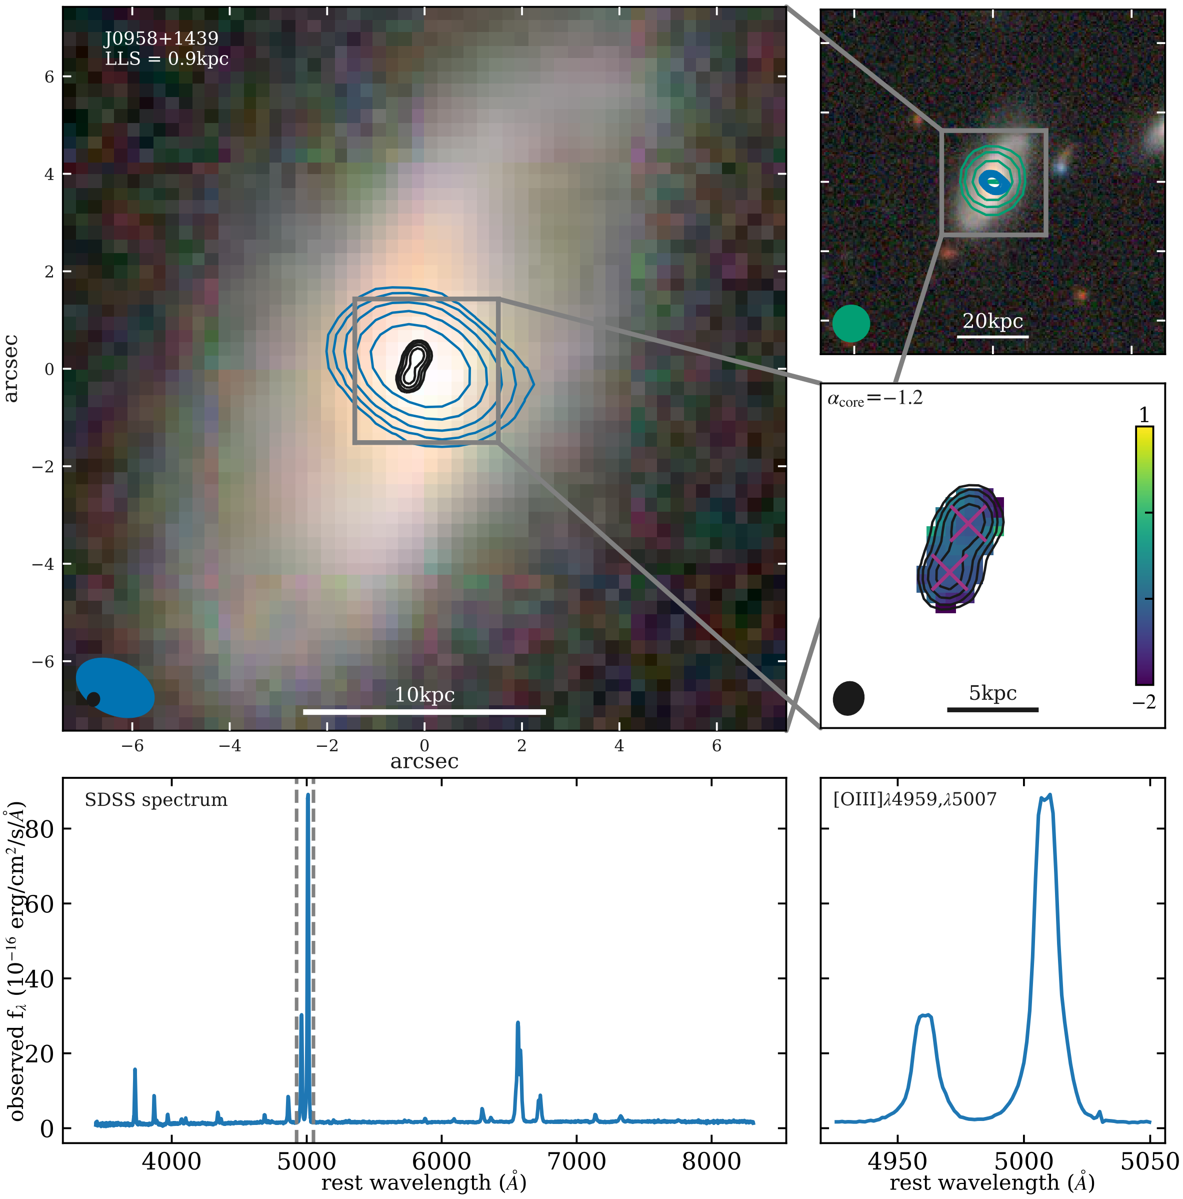


**Figure B11.** As Fig. 2 but for J0958+1439. Radio contours for all data are plotted at ±[8, 16, 32, 64, 128]$\sigma$.

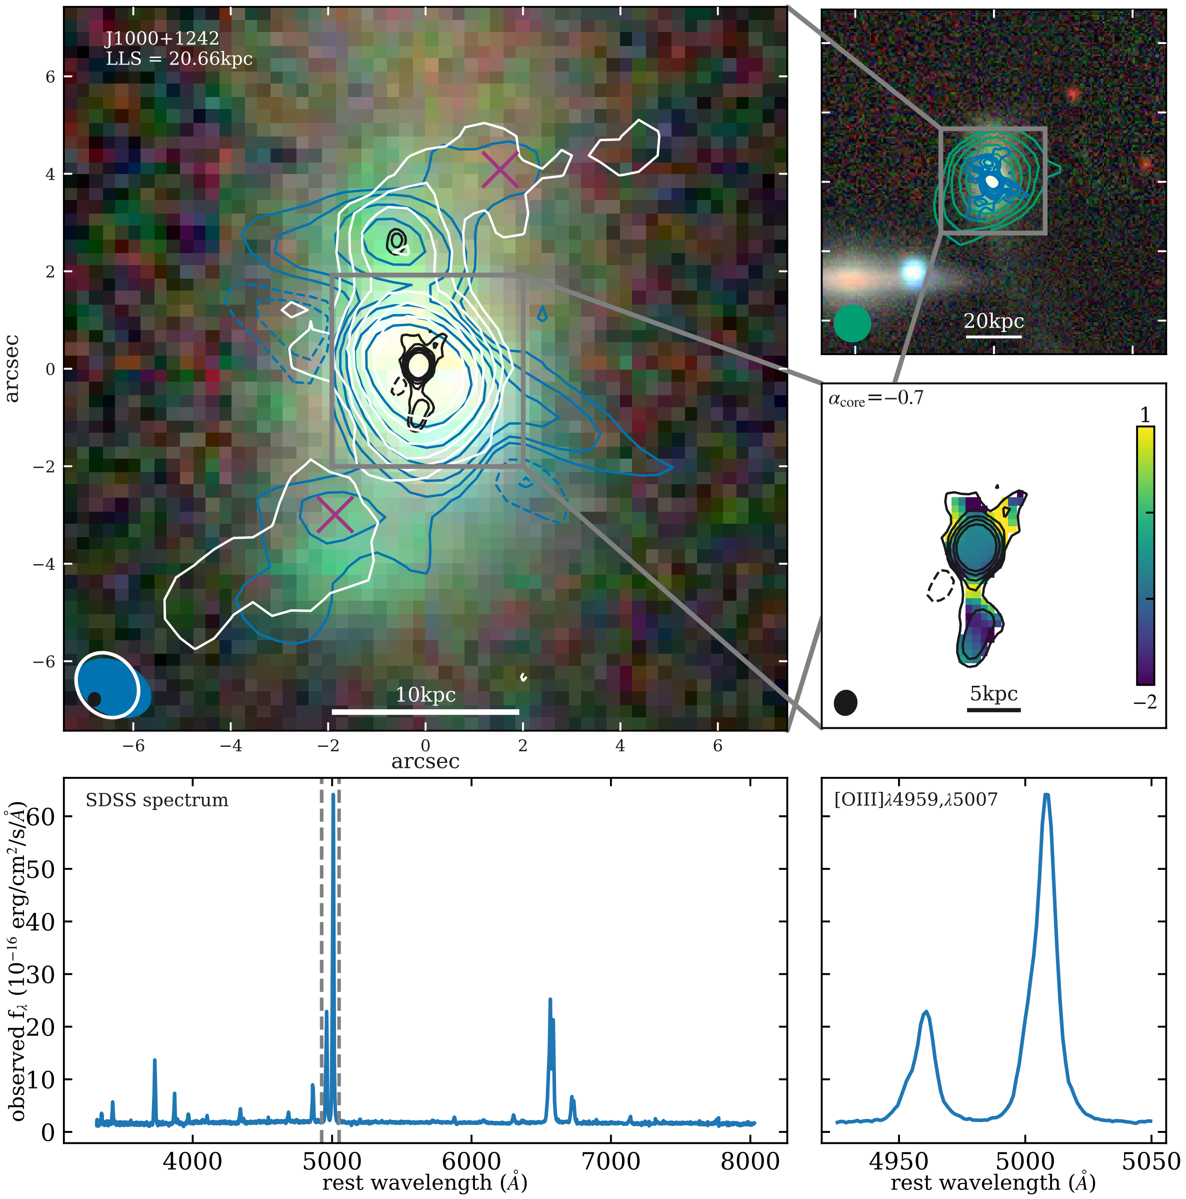


**Figure B12.** As Fig. 2 but for J1000+1242. Radio contours are plotted at ±[4, 8, 16, 32, 64, 128]$\sigma$ in FIRST and our L-band image and at ±[8, 16, 32, 64, 128]$\sigma$ for the C-band data. The white contours show the ∼1 arcsec C-band radio contours from figure 5 of Jarvis et al. (2019) with contours at the same intervals of $\sigma$ as the L-band data and the beam shown as a white outline in the bottom left corner. We additionally note that the prominent spike to the west of the core is a beam effect (as confirmed by the presence of symmetric negative contours of similar significance around this feature).

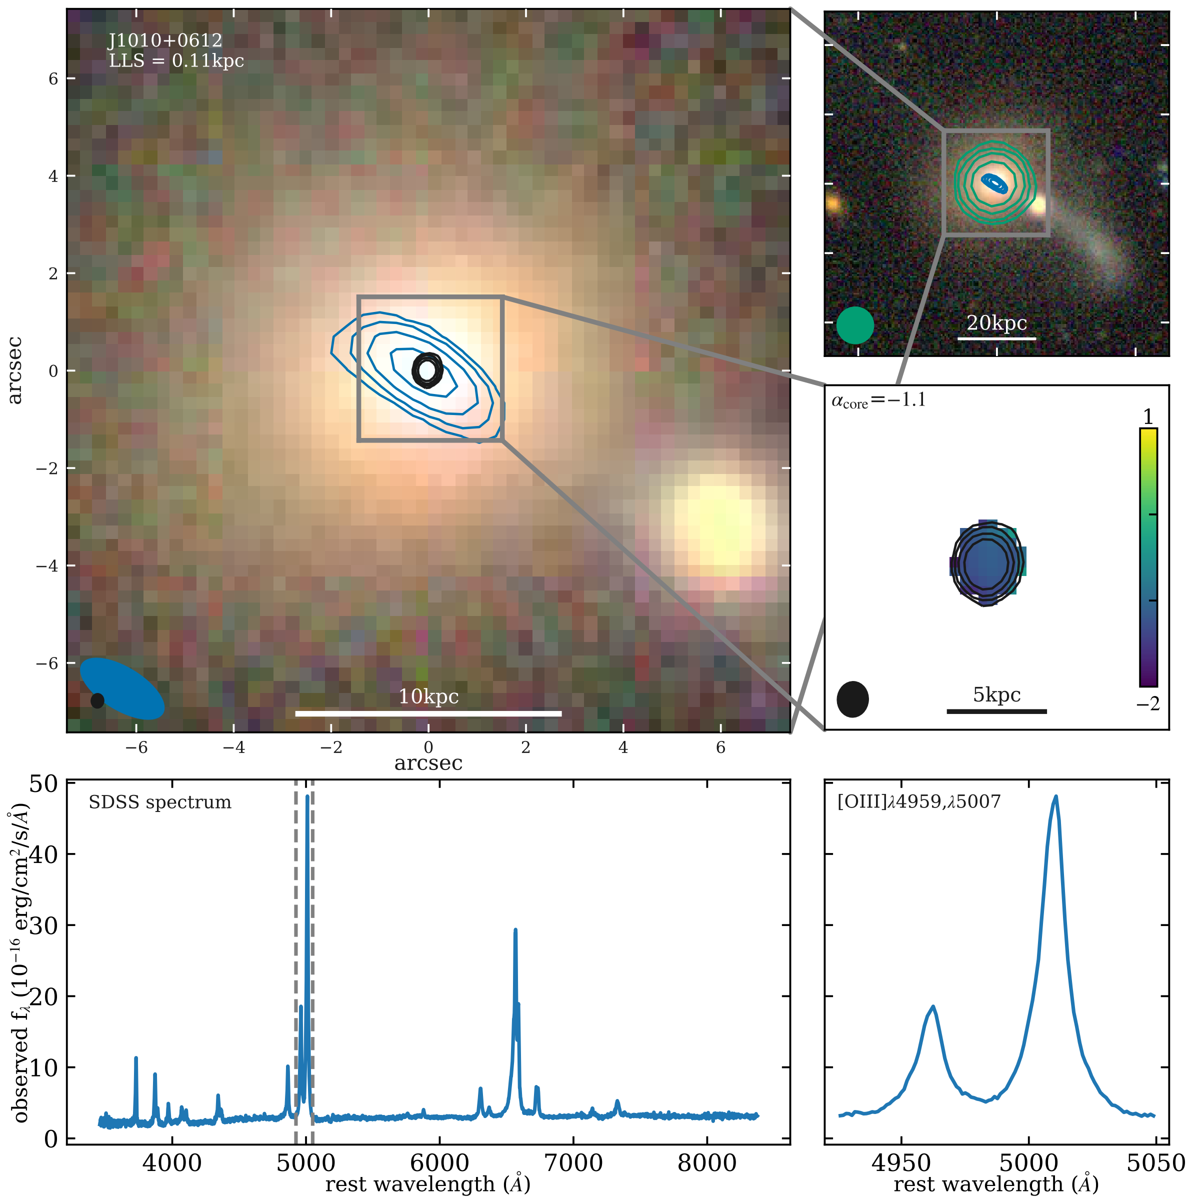


**Figure B13.** As Fig. 2 but for J1010+0612. Radio contours for all data are plotted at ±[16, 32, 64, 128]$\sigma$.

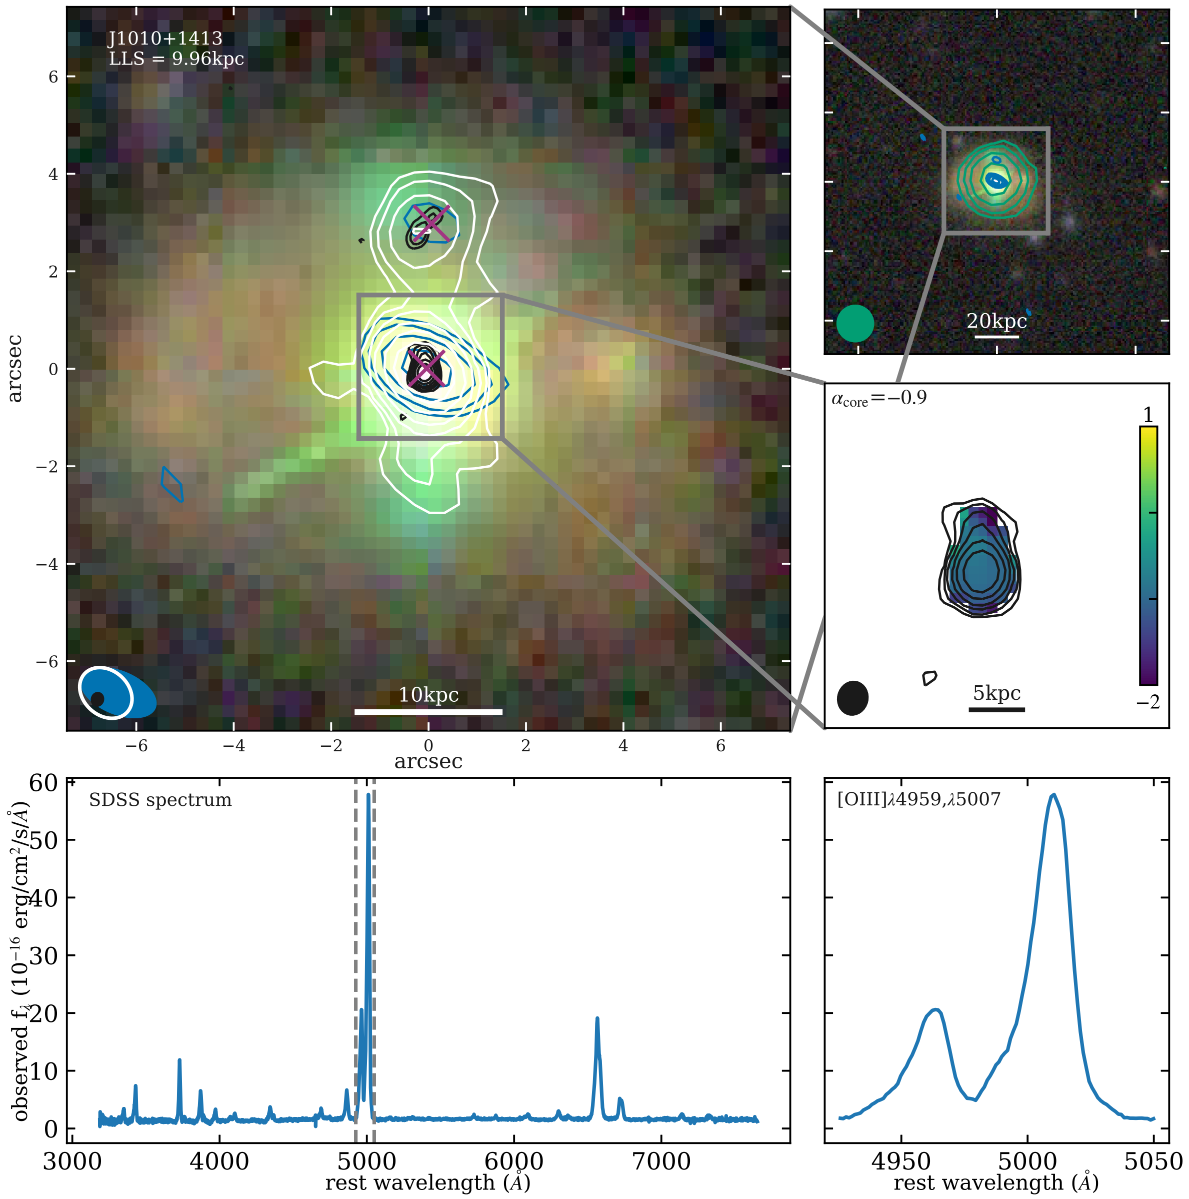


**Figure B14.** As Fig. 2 but for J1010+1413. Radio contours for all data are plotted at ±[4, 8, 16, 32, 64, 128]$\sigma$. The white contours show the ∼1 arcsec C-band radio contours from figure 5 of Jarvis et al. (2019) with contours at the same intervals of $\sigma$ as the images from this work and the beam shown as a white outline in the bottom left corner.

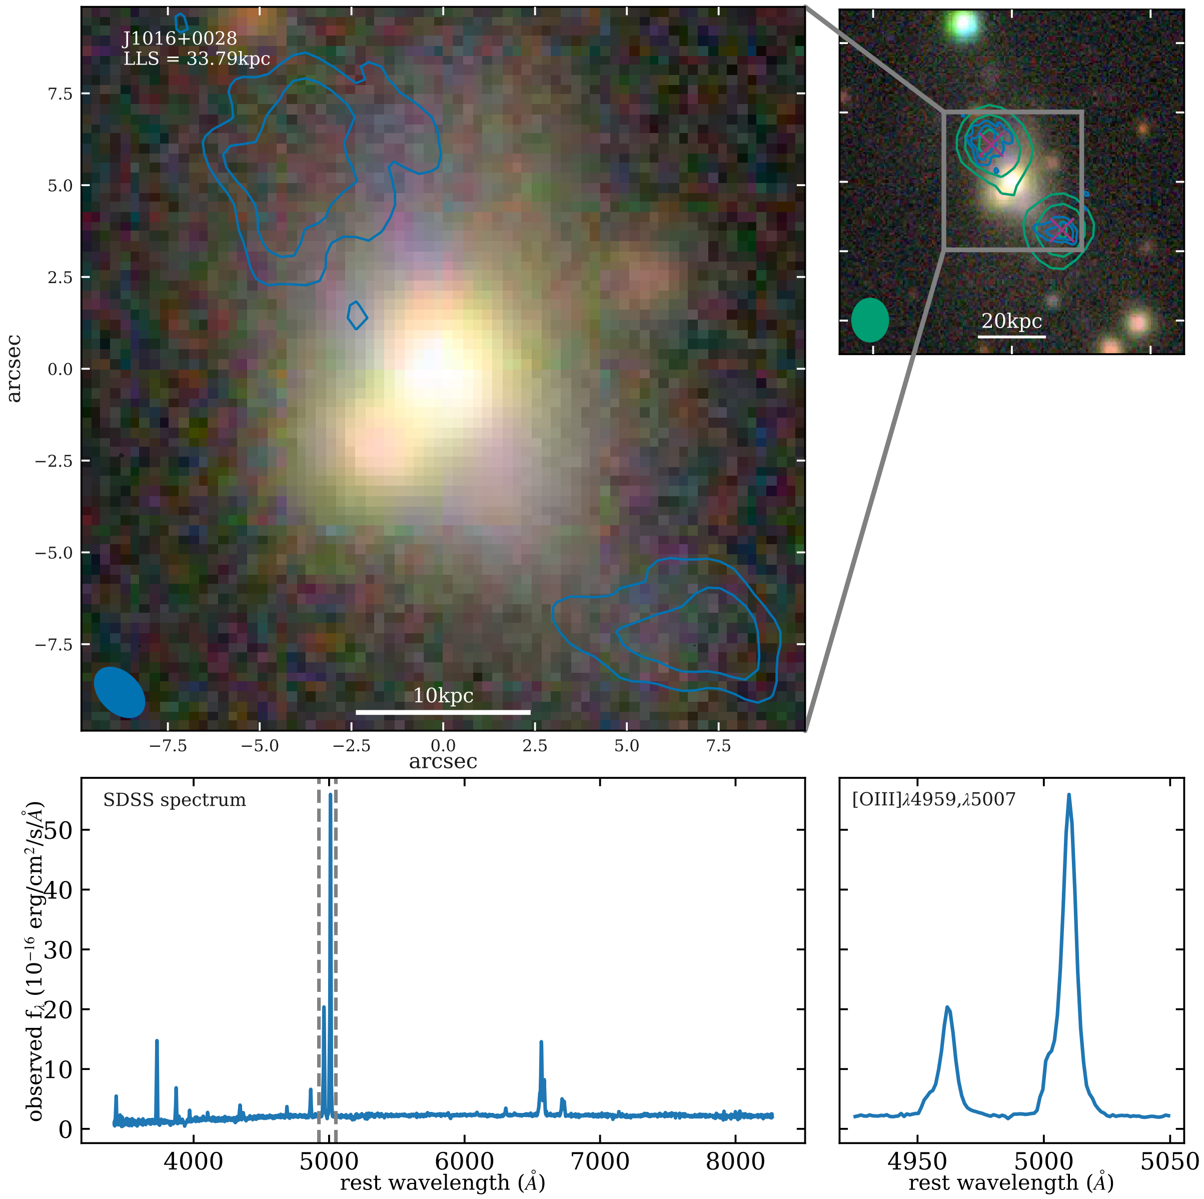


**Figure B15.** As Fig. 2 but for J1016+0028. Radio contours for all data are plotted at ±[4, 8, 16, 32, 64, 128]$\sigma$. This source is completely undetected in the C-band data and therefore no spectral index map is shown.

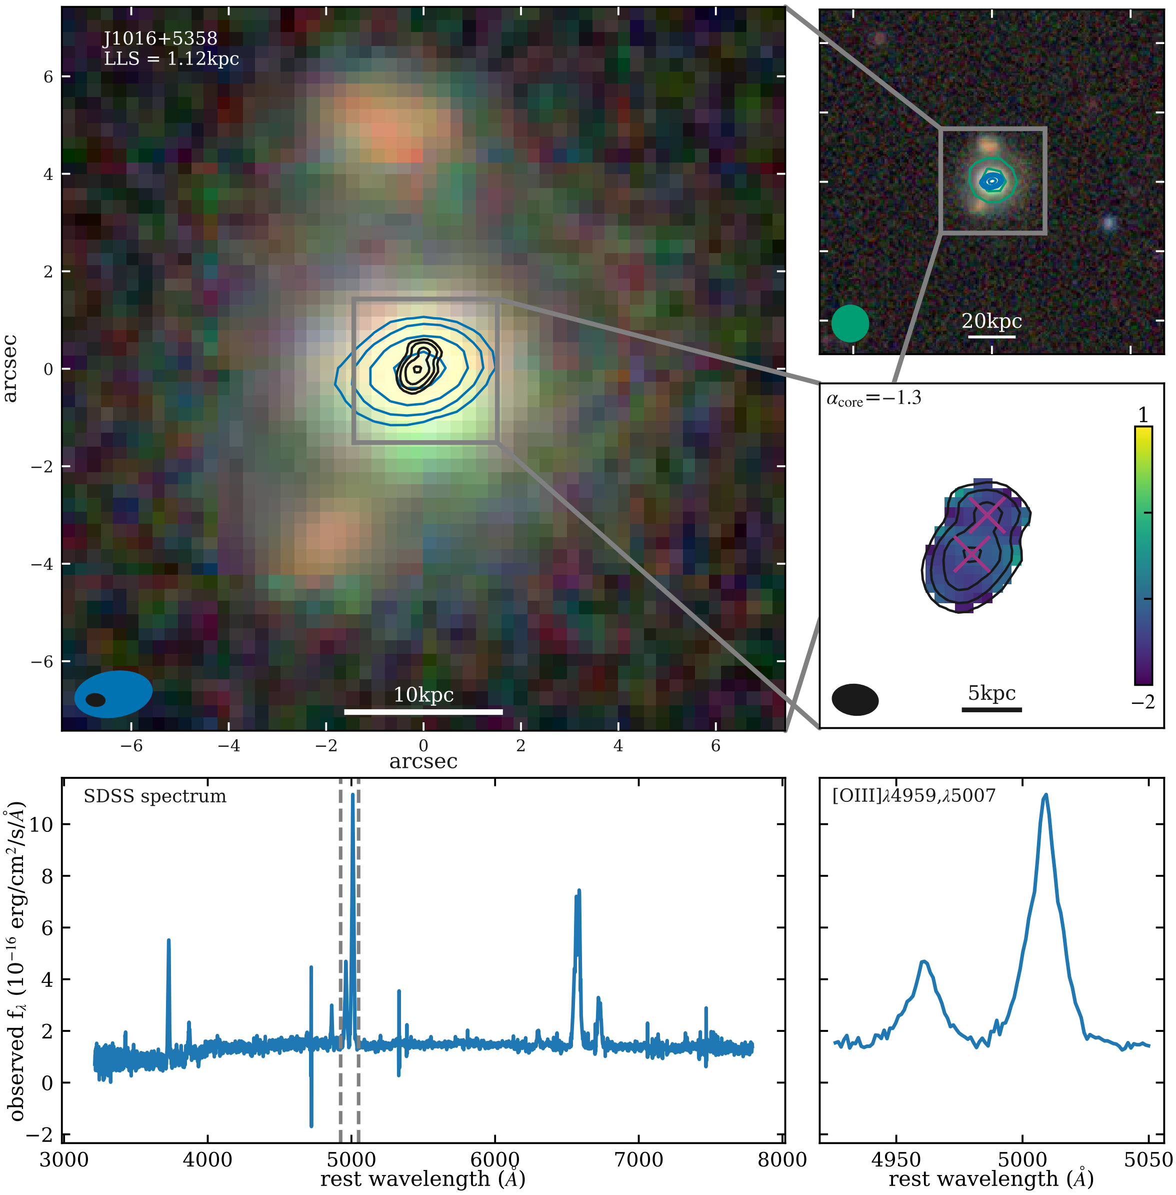


**Figure B16.** As Fig. 2 but for J1016+5358. Radio contours for all data are plotted at ±[8, 16, 32, 64, 128]$\sigma$.

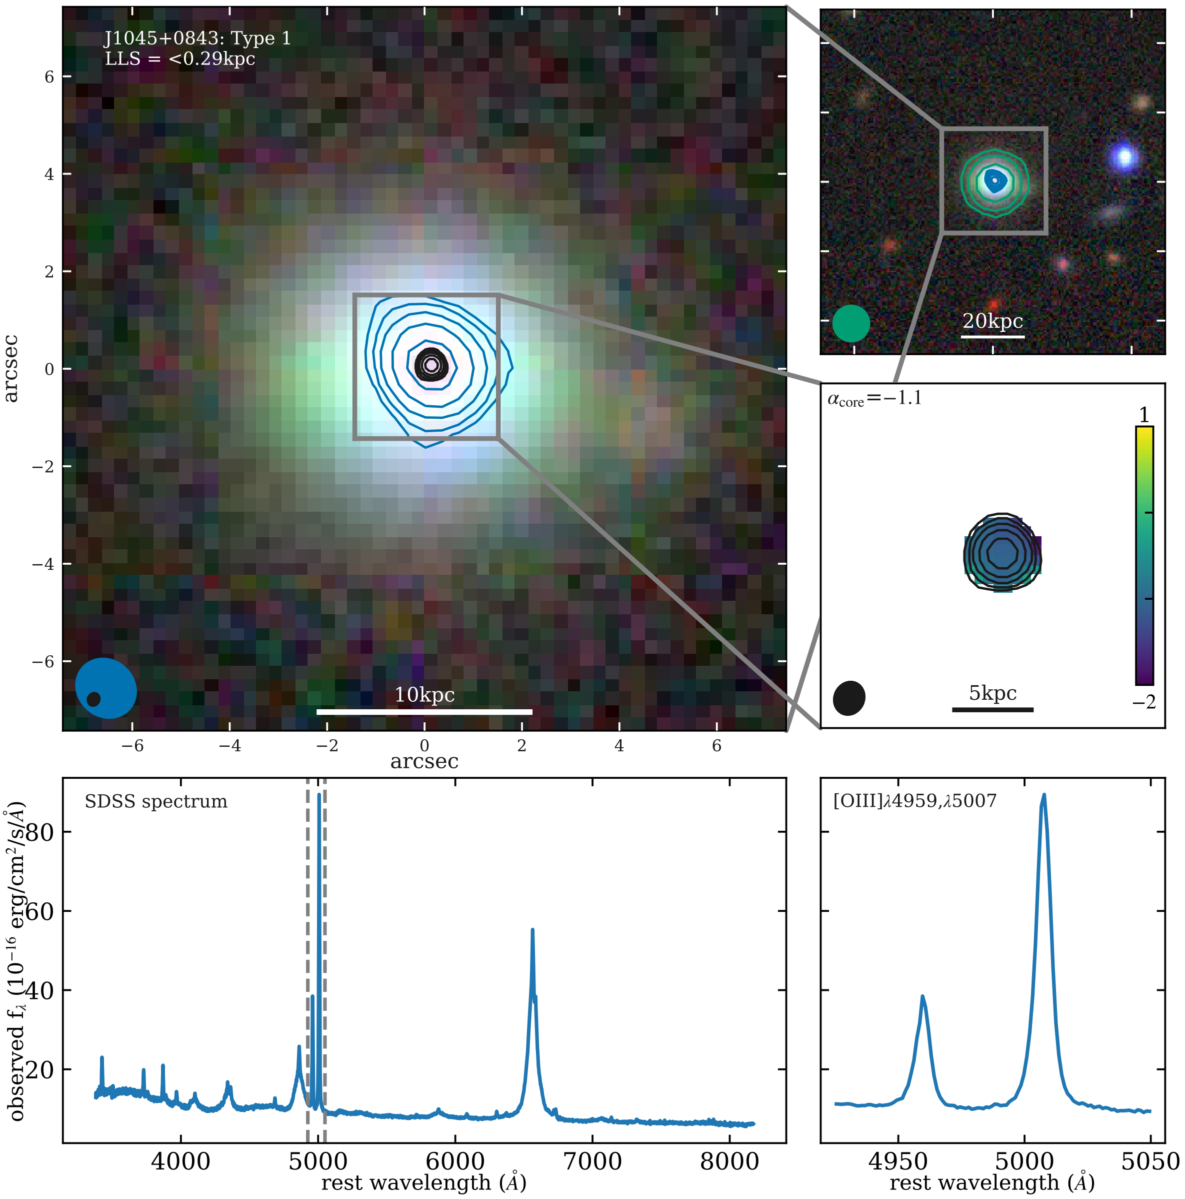


**Figure B17.** As Fig. 2 but for J1045+0843. Radio contours for all data are plotted at ±[8, 16, 32, 64, 128]$\sigma$.

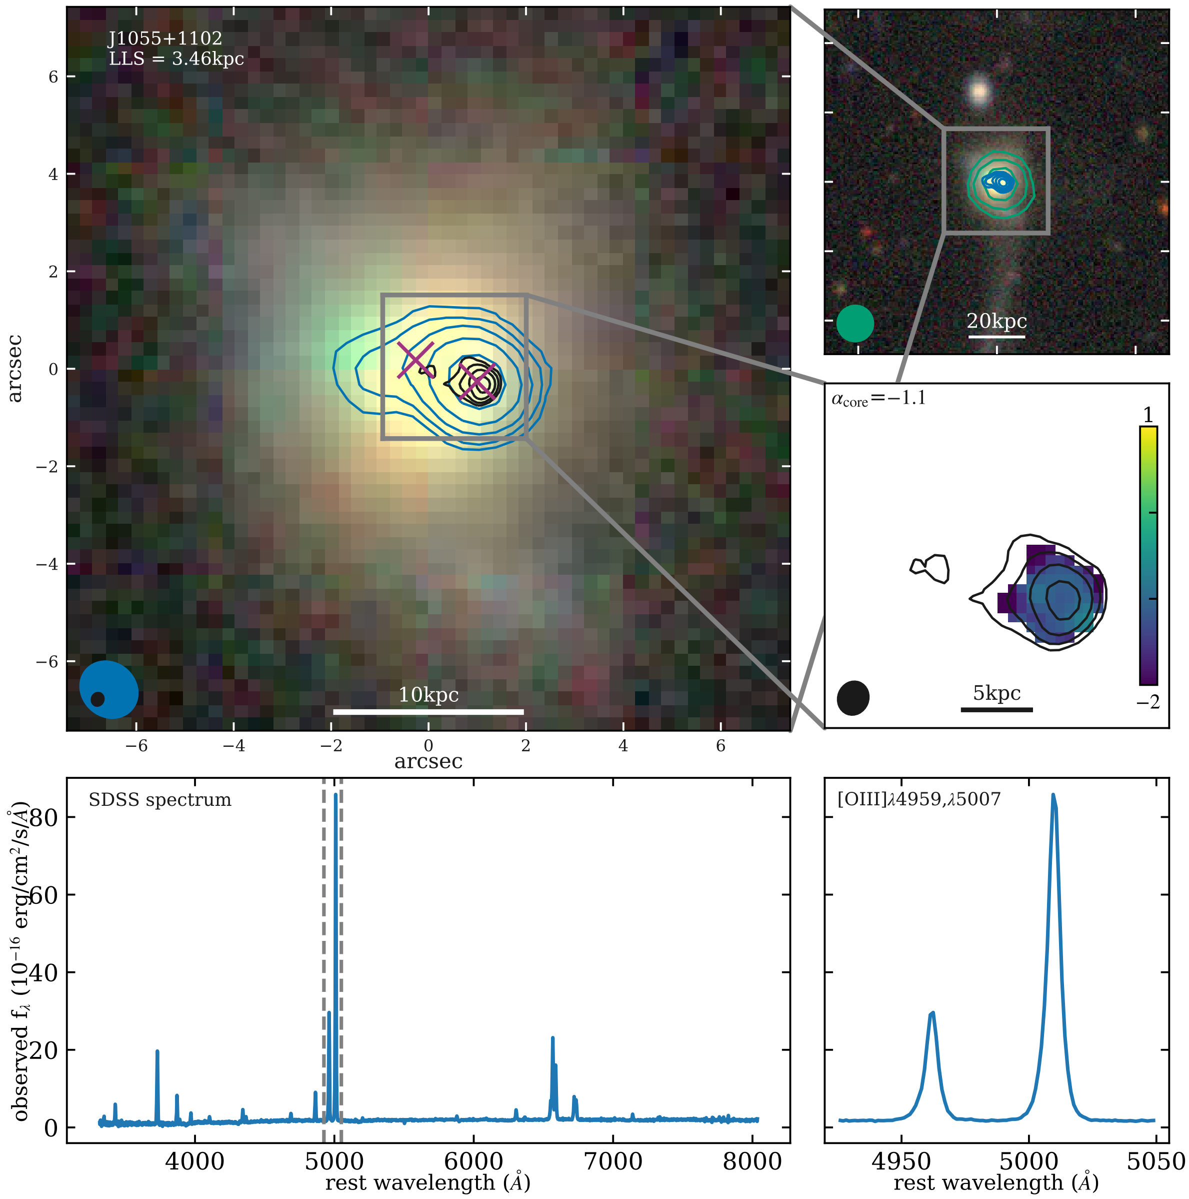


**Figure B18.** As Fig. 2 but for J1055+1102. Radio contours for all data are plotted at ±[4, 8, 16, 32, 64, 128]$\sigma$.

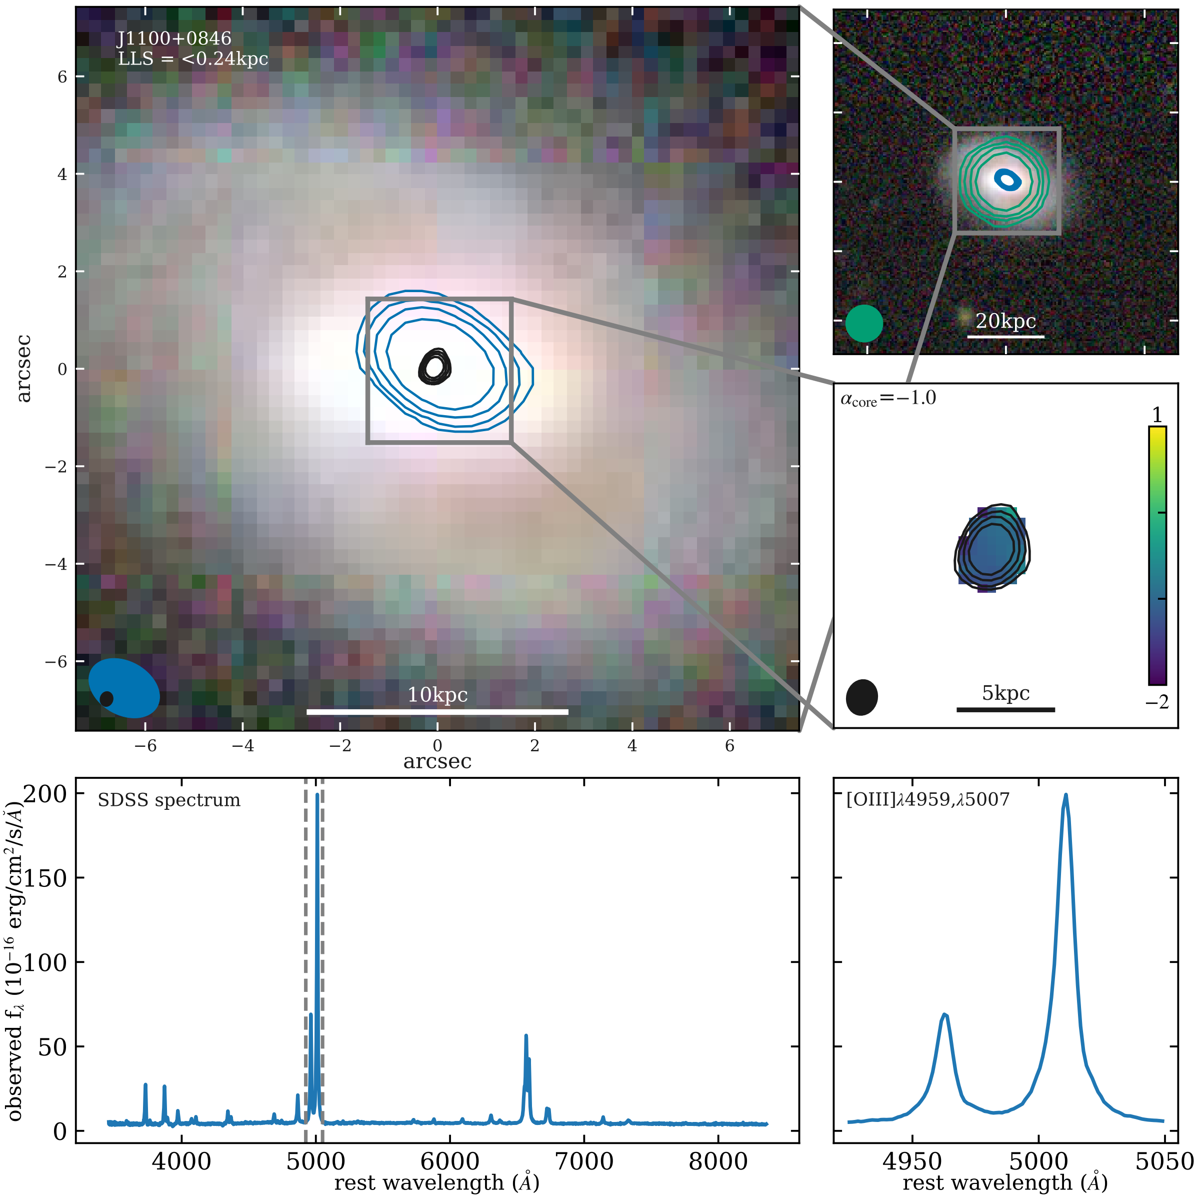


**Figure B19.** As Fig. 2 but for J1100+0846. Radio contours for all data are plotted at ±[16, 32, 64, 128]$\sigma$.

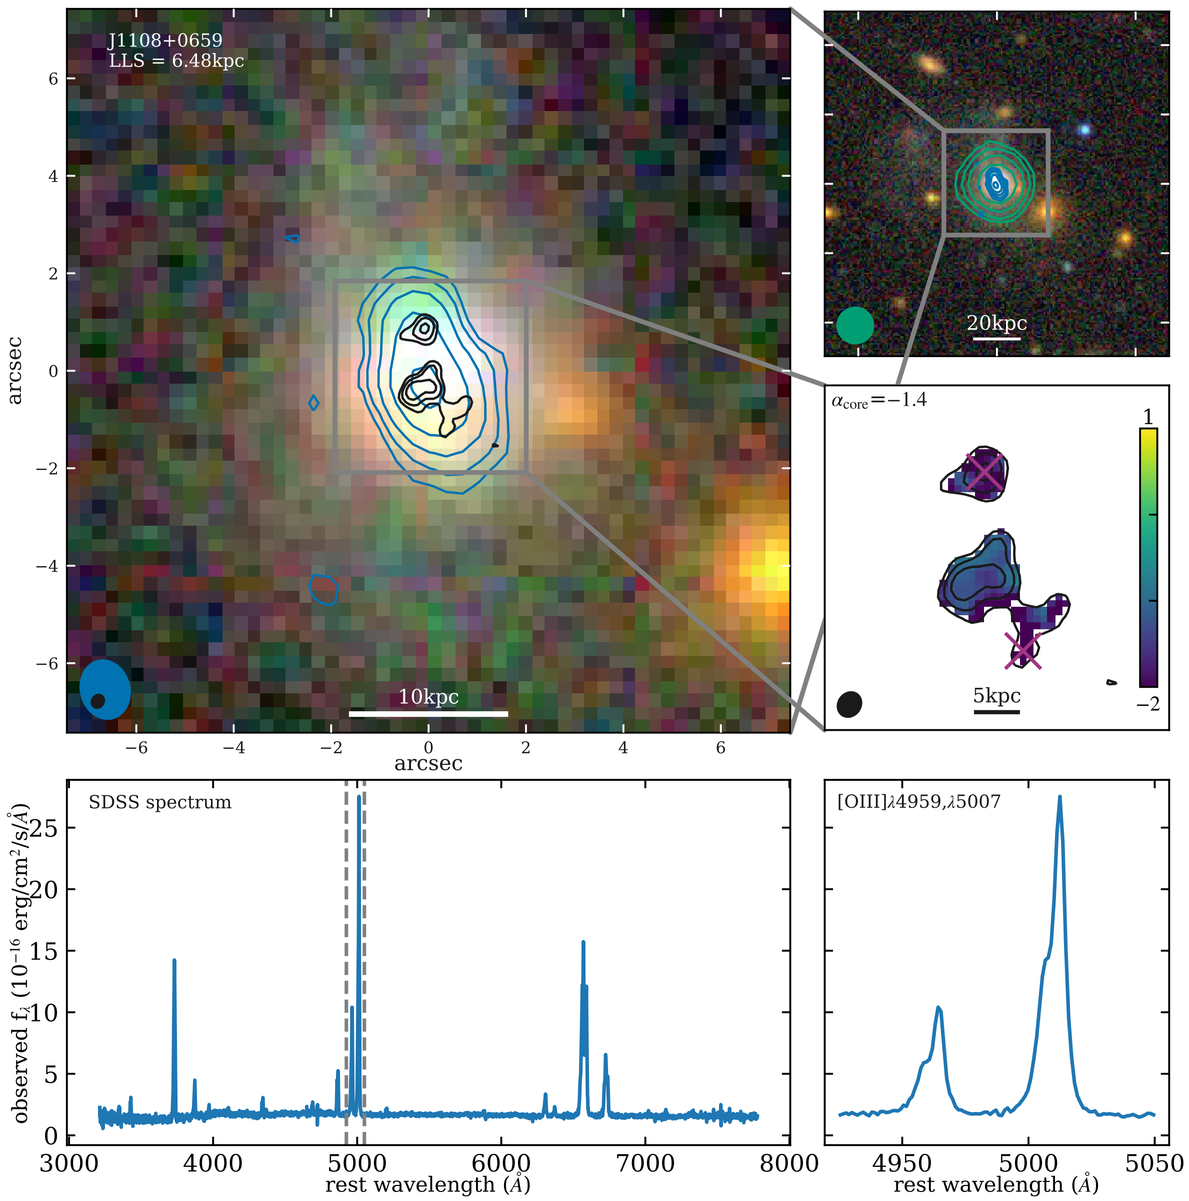


**Figure B20.** As Fig. 2 but for J1108+0659. Radio contours for all data are plotted at ±[4, 8, 16, 32, 64, 128]$\sigma$.

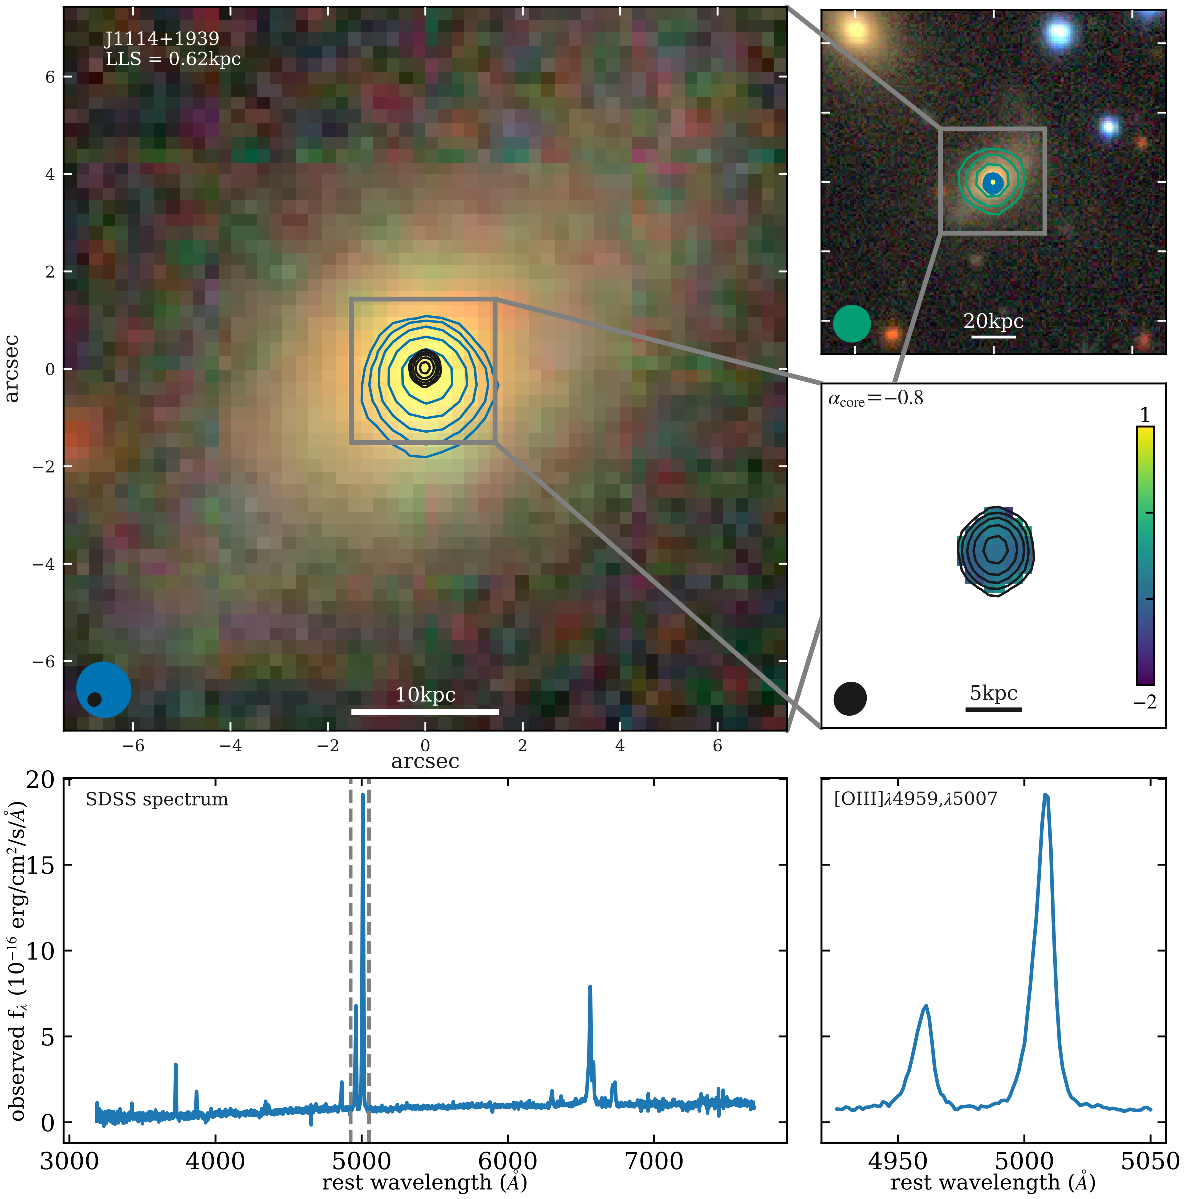


**Figure B21.** As Fig. 2 but for J1114+1939. Radio contours for all data are plotted at ±[8, 16, 32, 64, 128]$\sigma$.

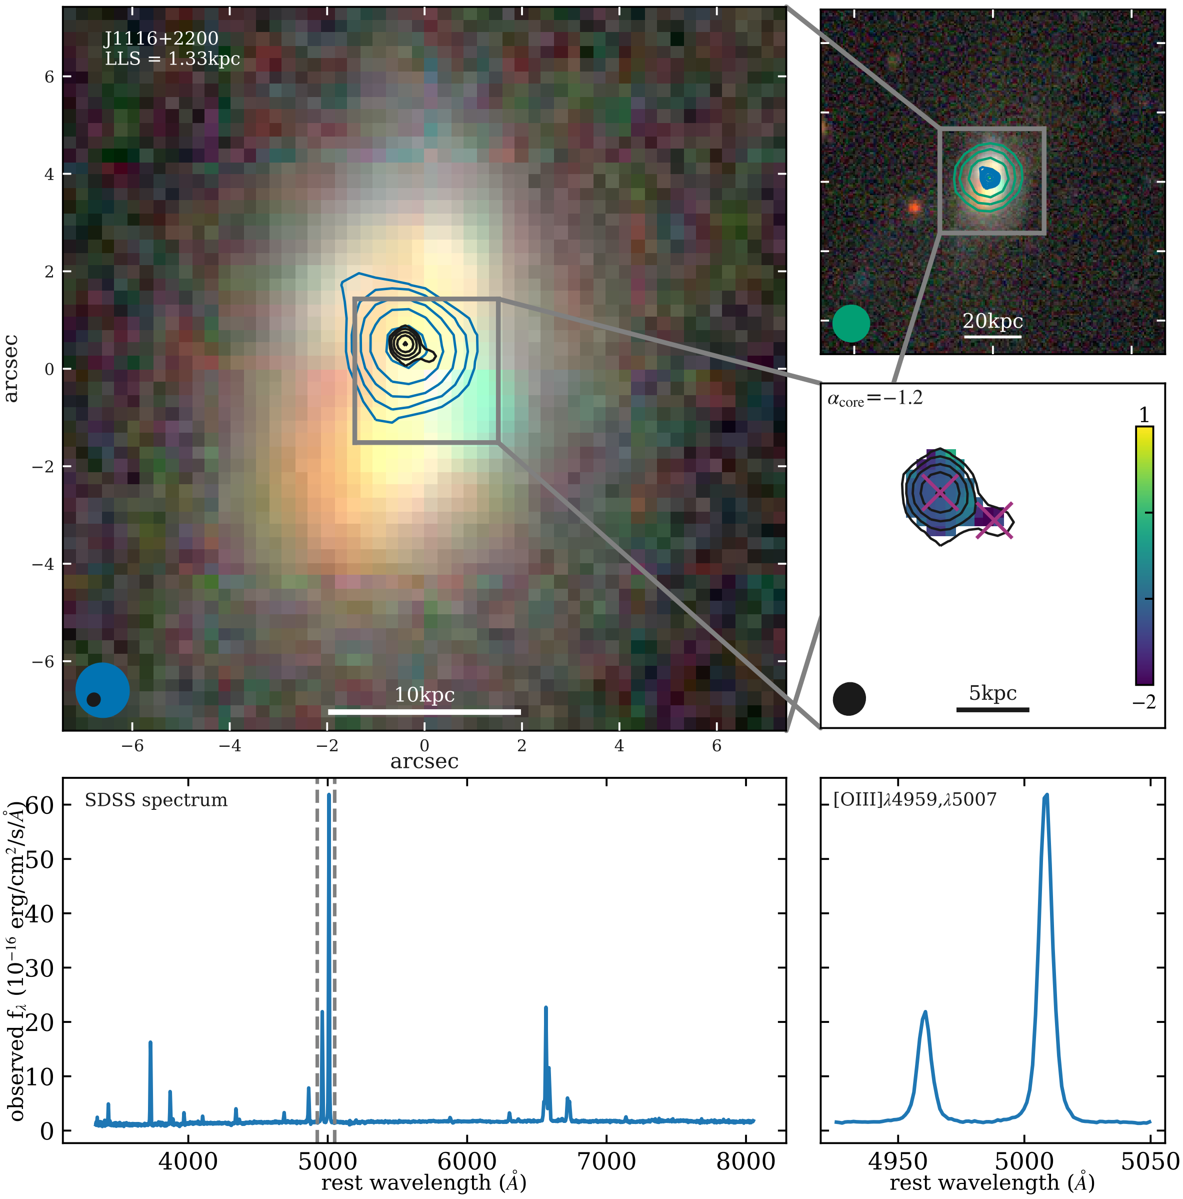


**Figure B22.** As Fig. 2 but for J1116+2200. Radio contours for all data are plotted at ±[8, 16, 32, 64, 128]$\sigma$.

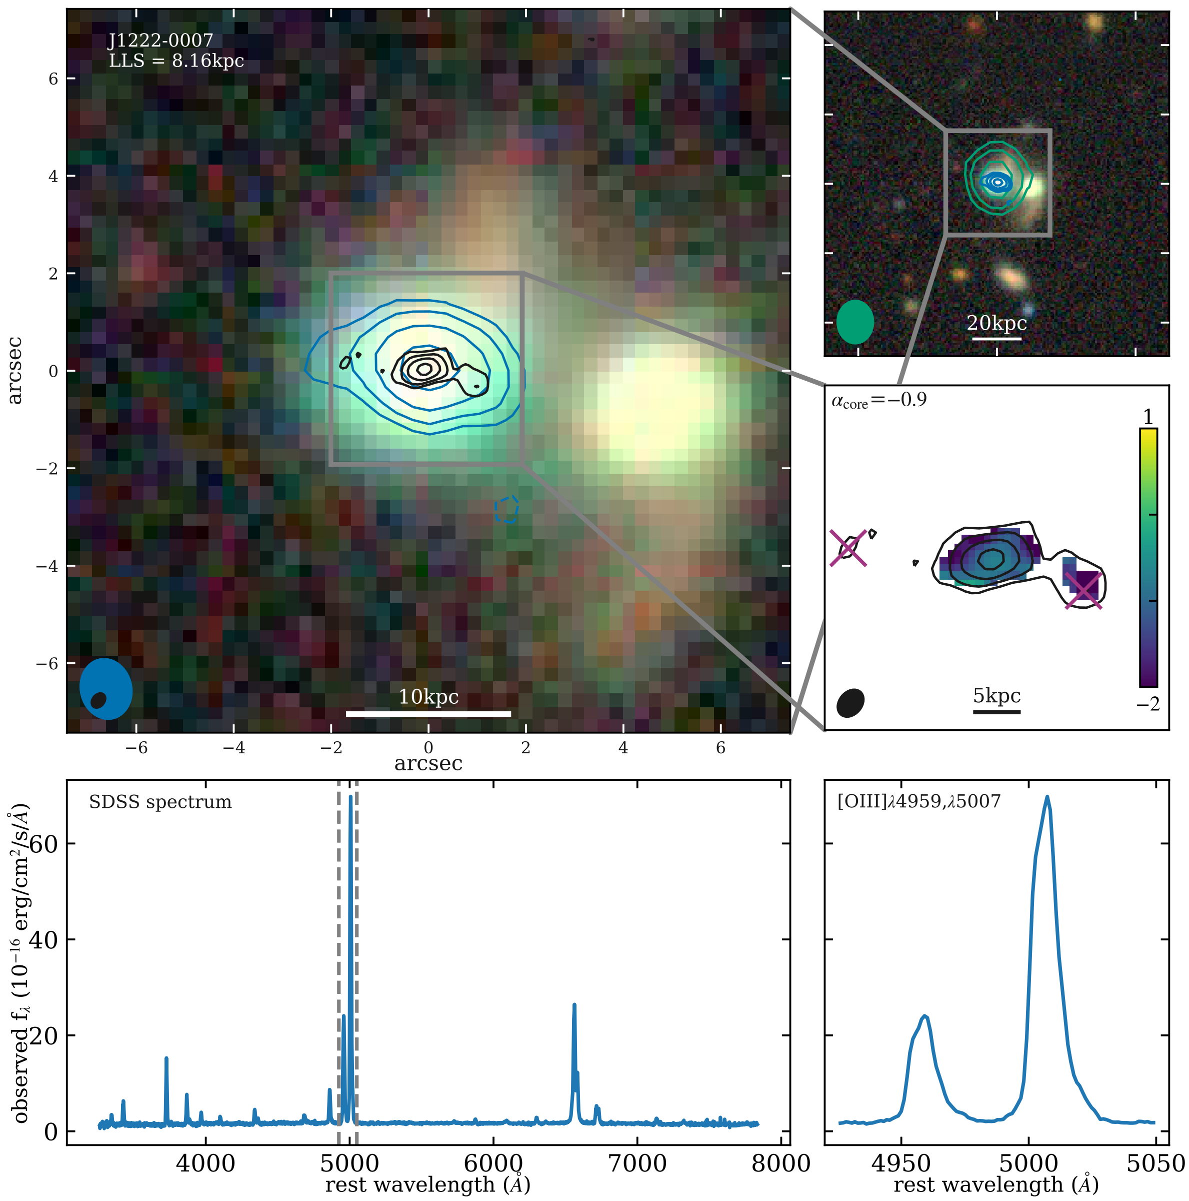


**Figure B23.** As Fig. 2 but for J1222-0007. Radio contours for all data are plotted at ±[4, 8, 16, 32, 64, 128]$\sigma$.

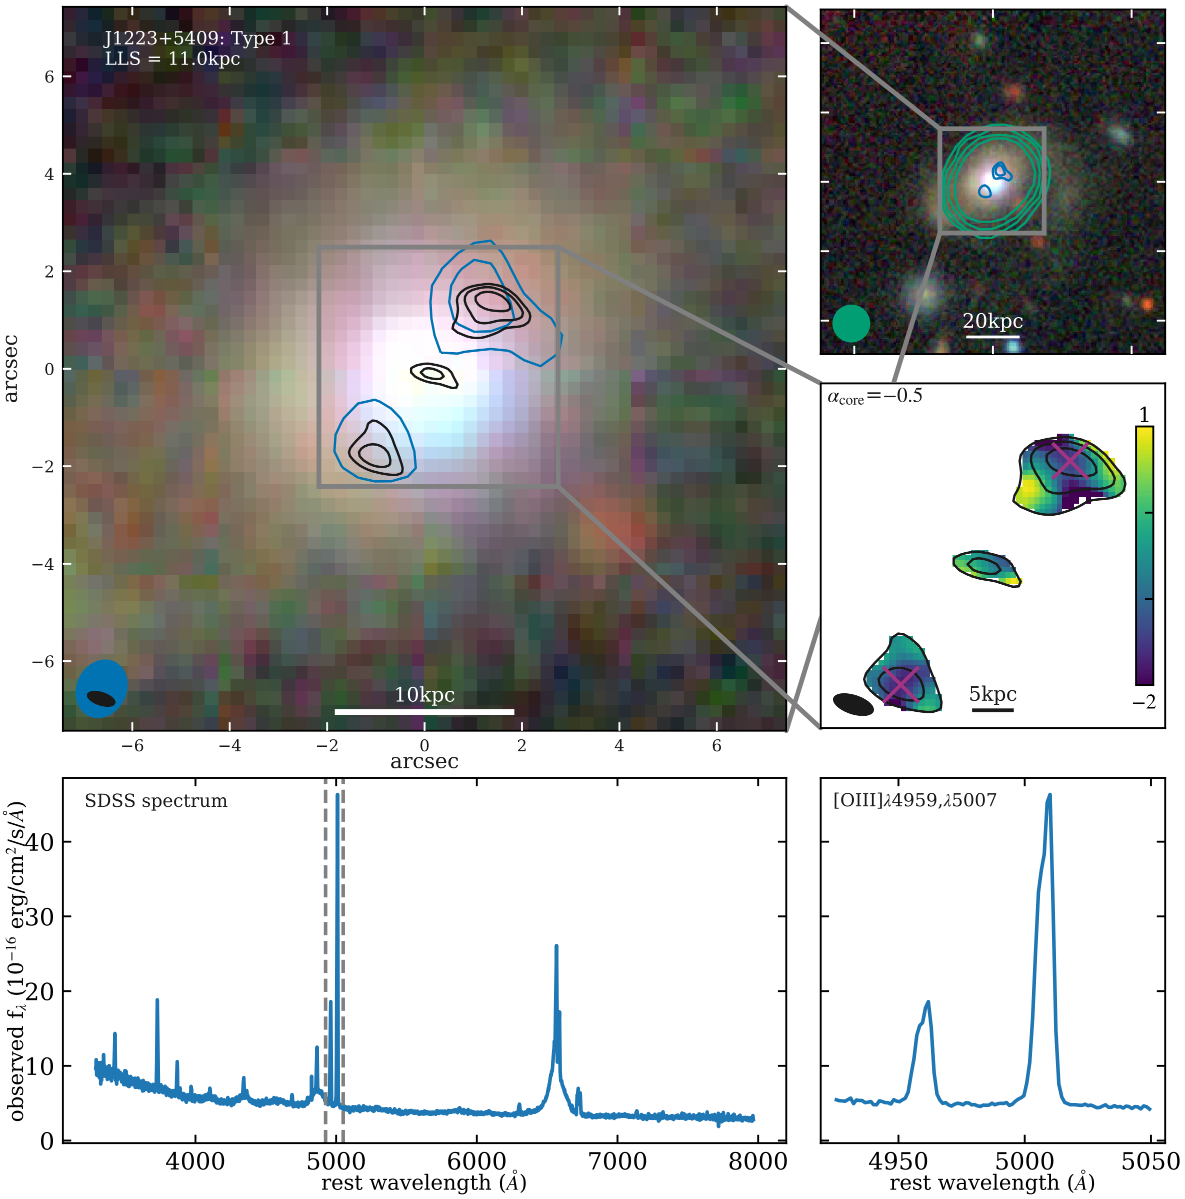


**Figure B24.** As Fig. 2 but for J1223+5409. Radio contours for all data are plotted at ±[16, 32, 64, 128]$\sigma$.

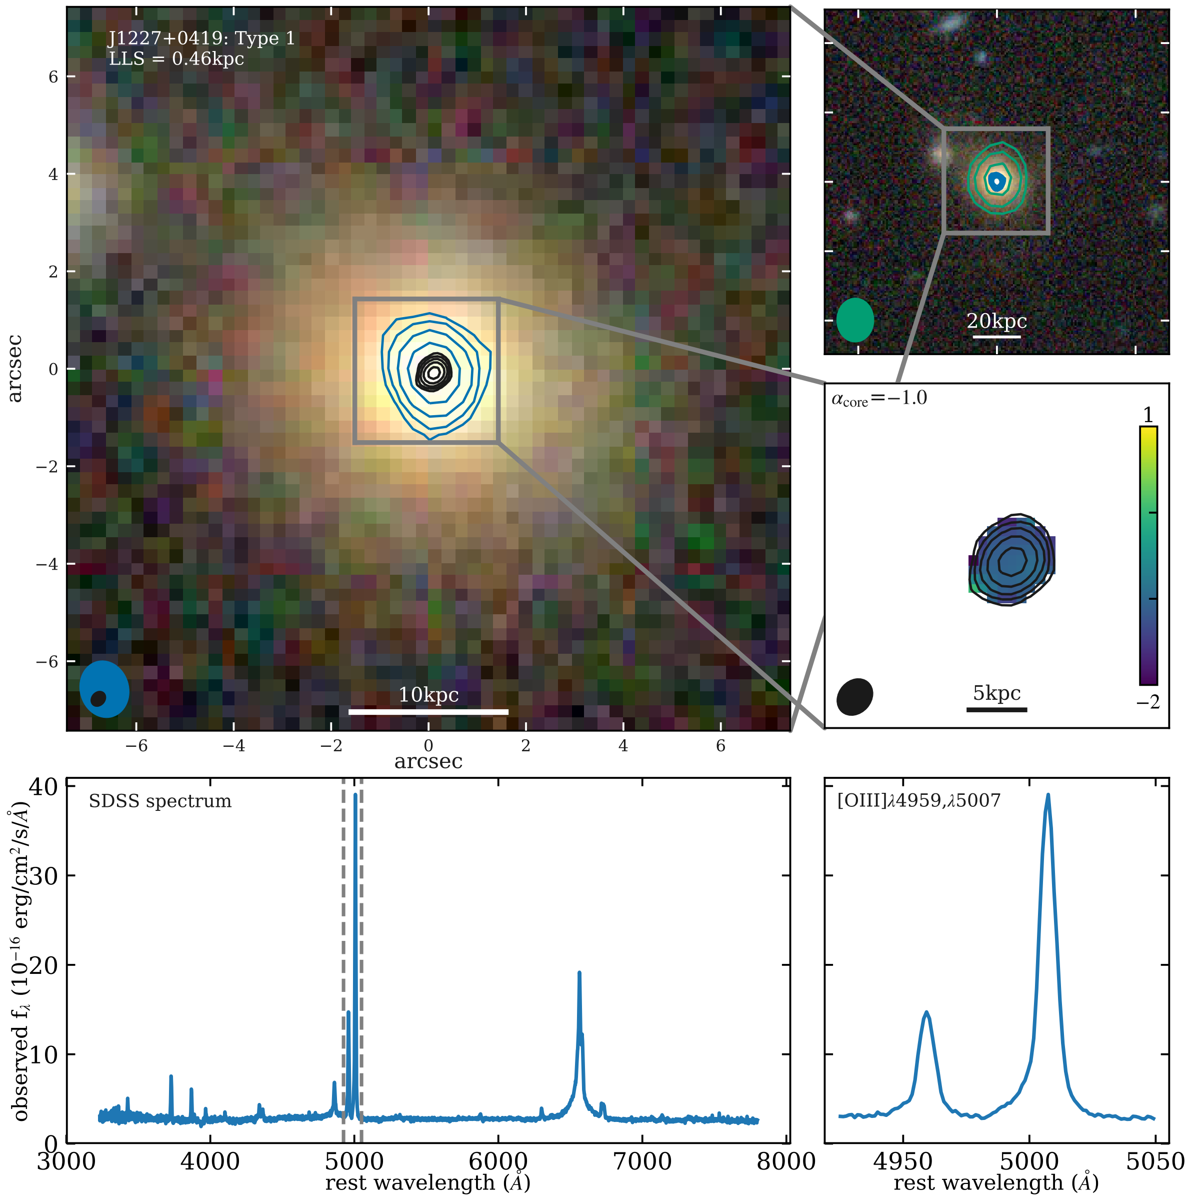


**Figure B25.** As Fig. 2 but for J1227+0419. Radio contours for all data are plotted at ±[8, 16, 32, 64, 128]$\sigma$.

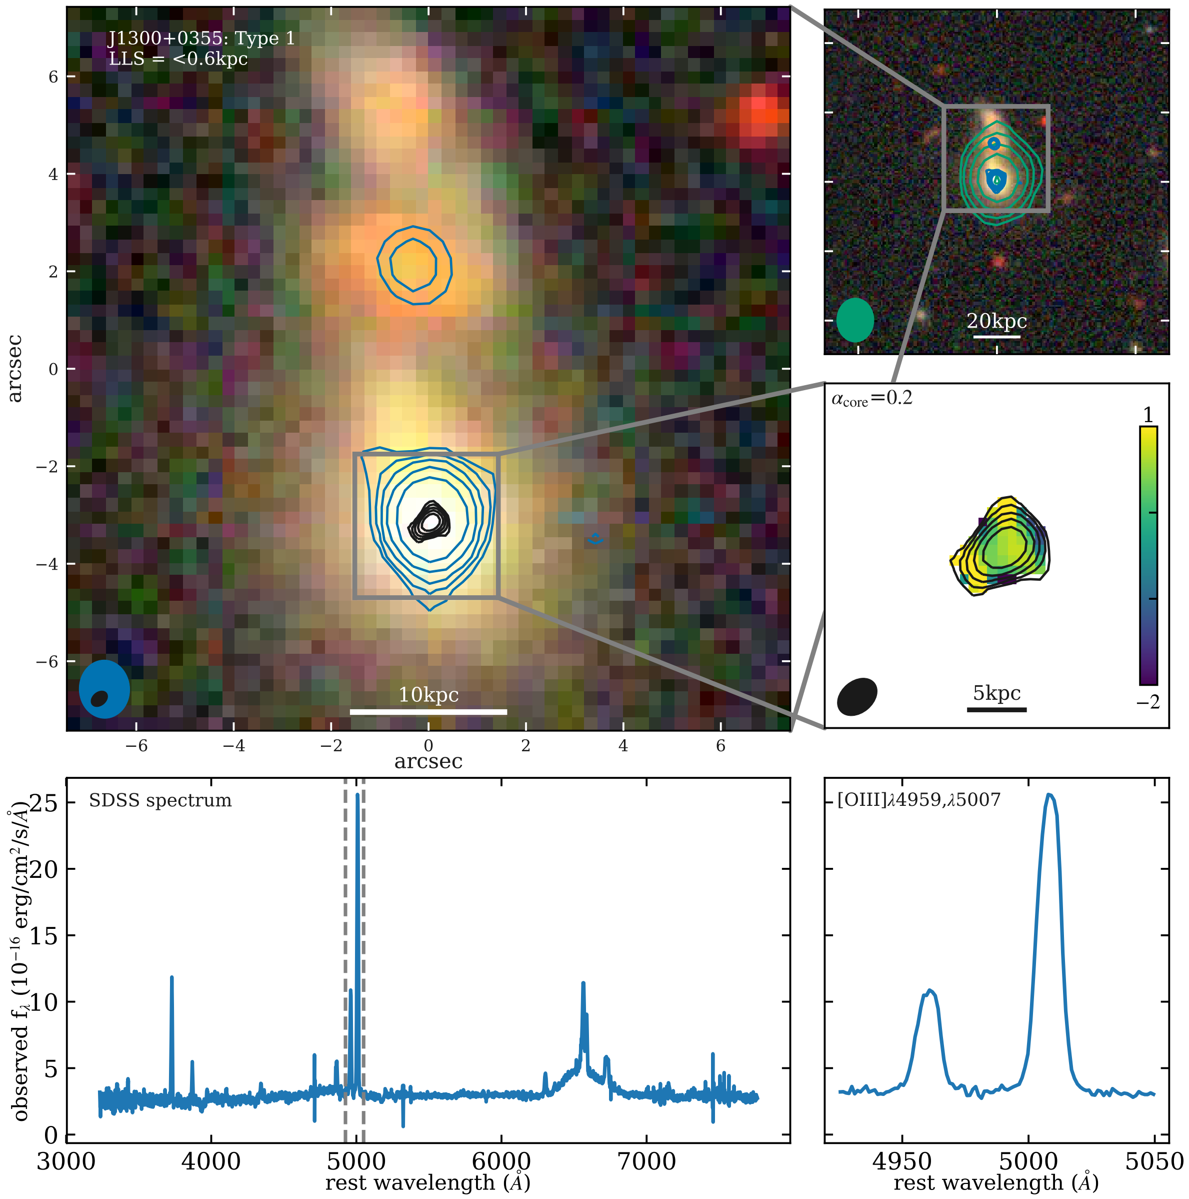


**Figure B26.** As Fig. 2 but for J1300+0355. Radio contours for all data are plotted at ±[8, 16, 32, 64, 128]$\sigma$. As discussed in Section B26 the northern radio component is not associated with the primary target and is therefore not used to calculate the largest linear size for this source.

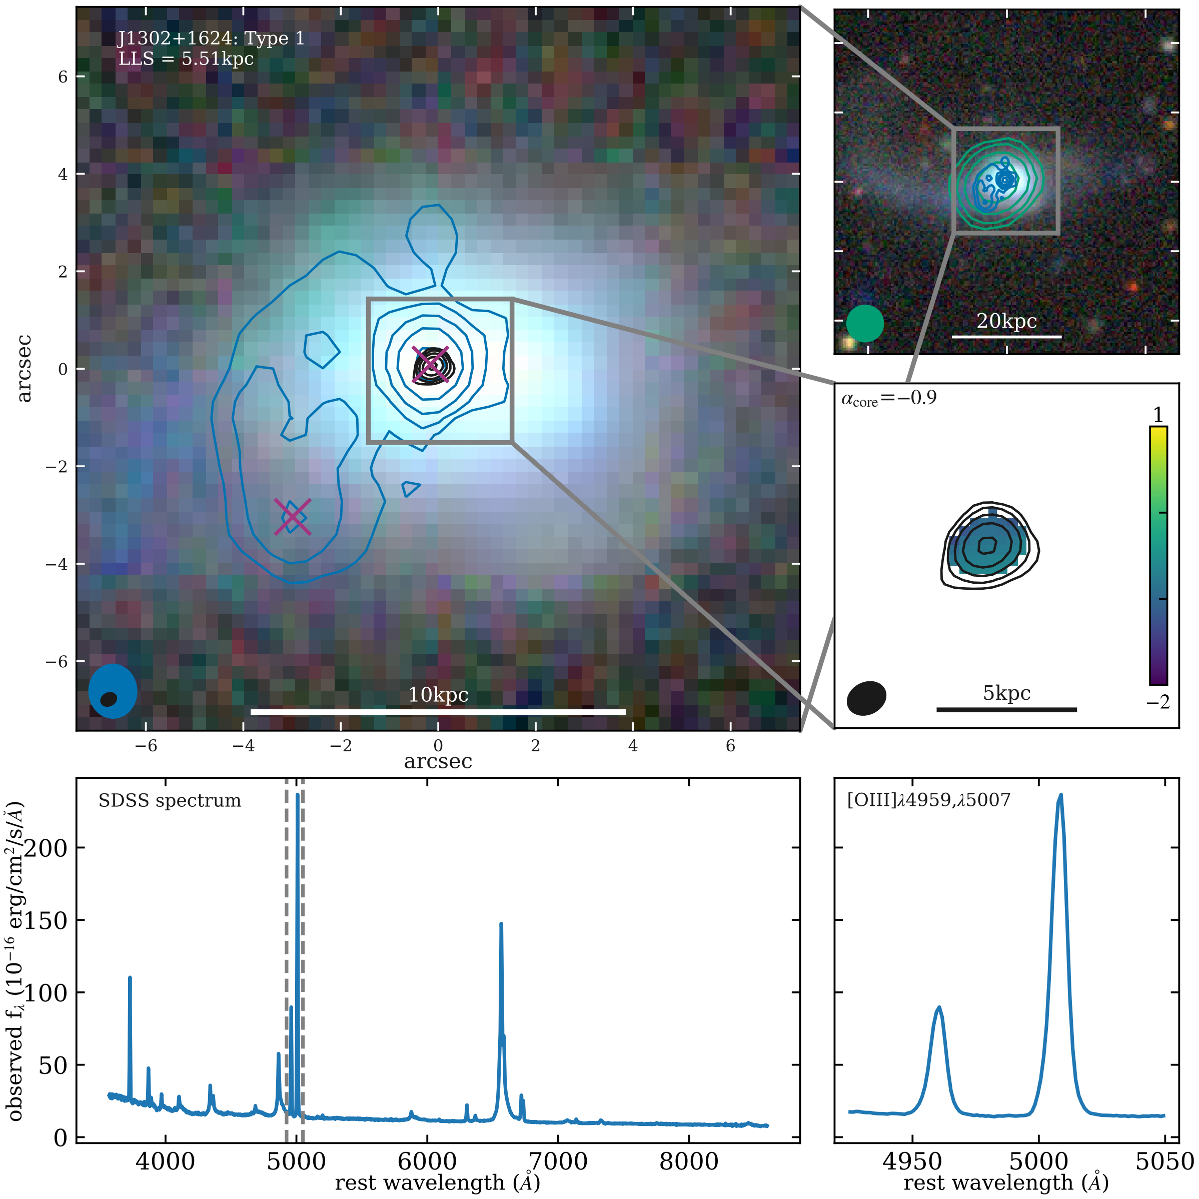


**Figure B27.** As Fig. 2 but for J1302+1624. Radio contours for all data are plotted at ±[8, 16, 32, 64, 128]$\sigma$.

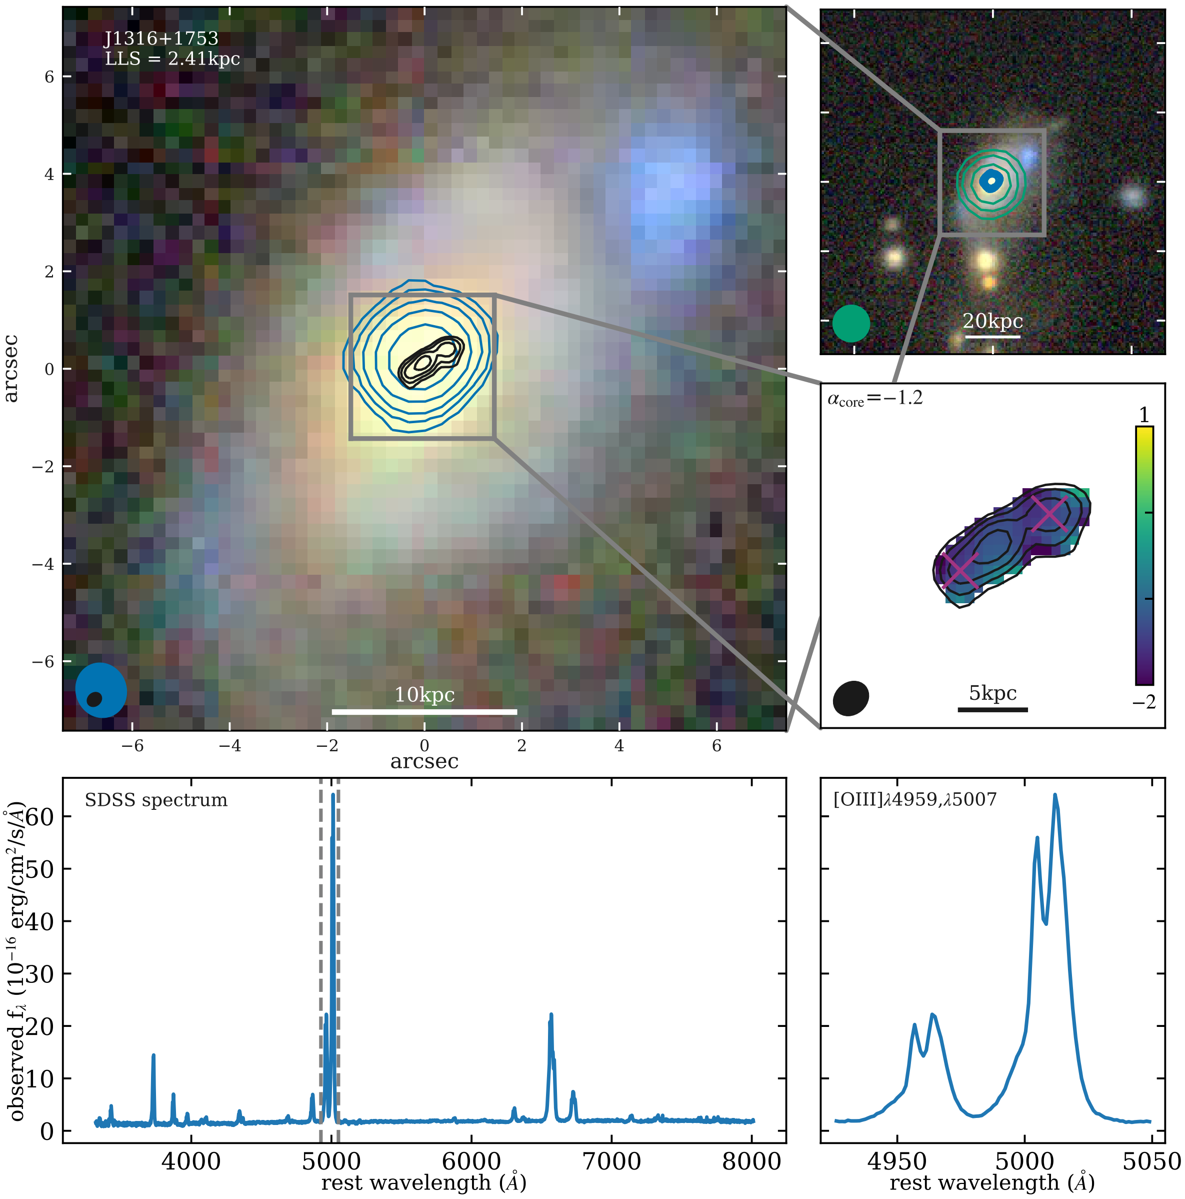


**Figure B28.** As Fig. 2 but for J1316+1753. Radio contours for all data are plotted at ±[8, 16, 32, 64, 128]$\sigma$.

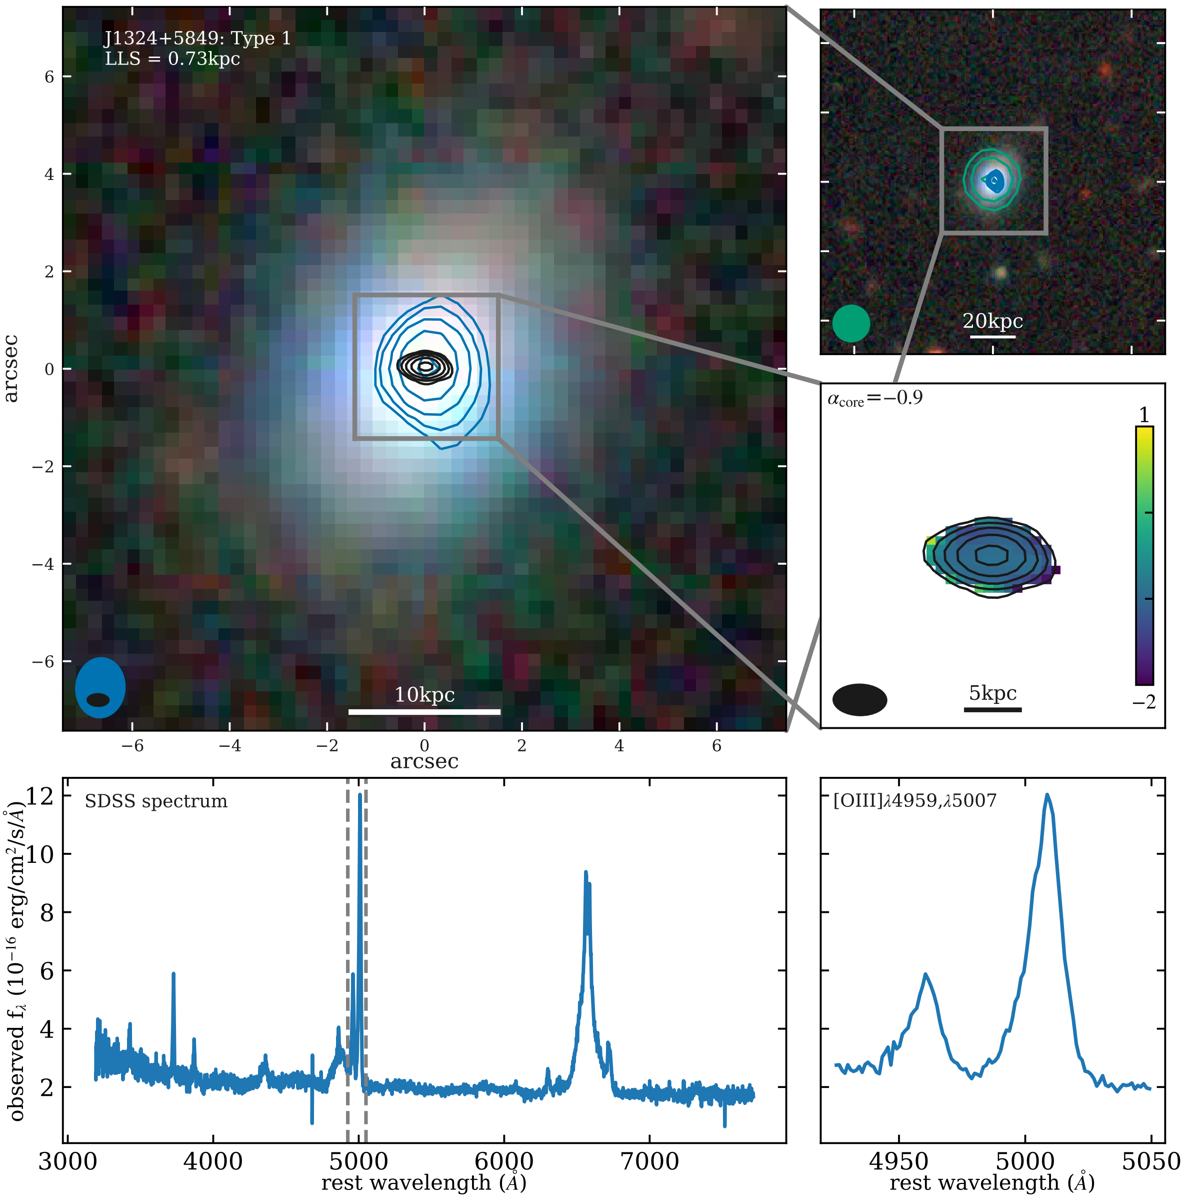


**Figure B29.** As Fig. 2 but for J1324+5849. Radio contours for all data are plotted at ±[8, 16, 32, 64, 128]$\sigma$.

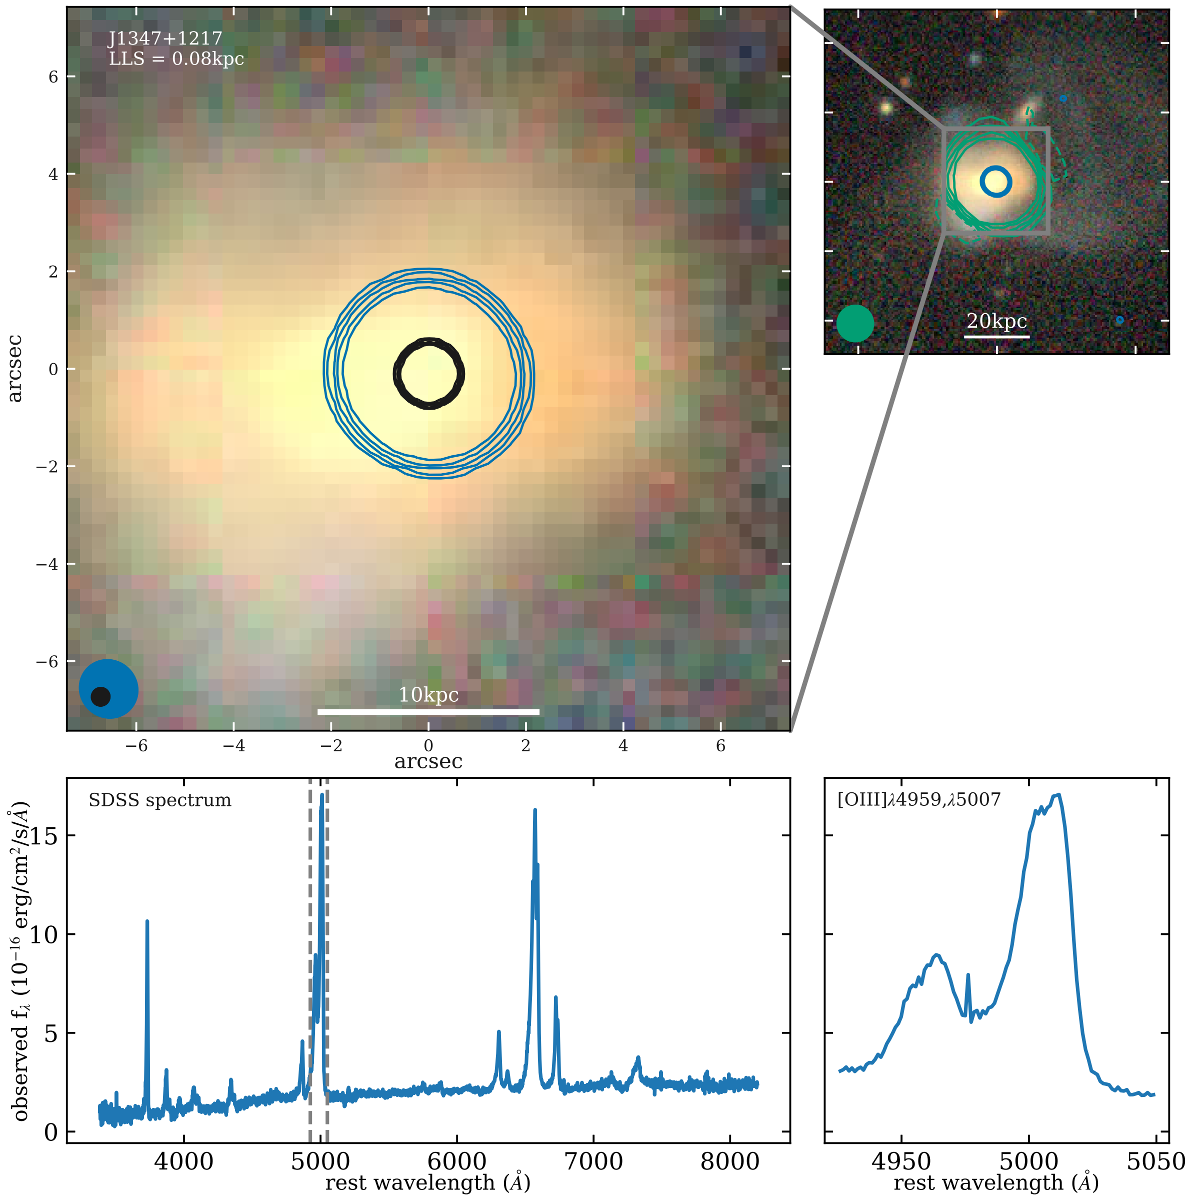


**Figure B30.** As Fig. 2 but for J1347+1217. Radio contours for all data are plotted at ±[8, 16, 32, 64, 128]$\sigma$.

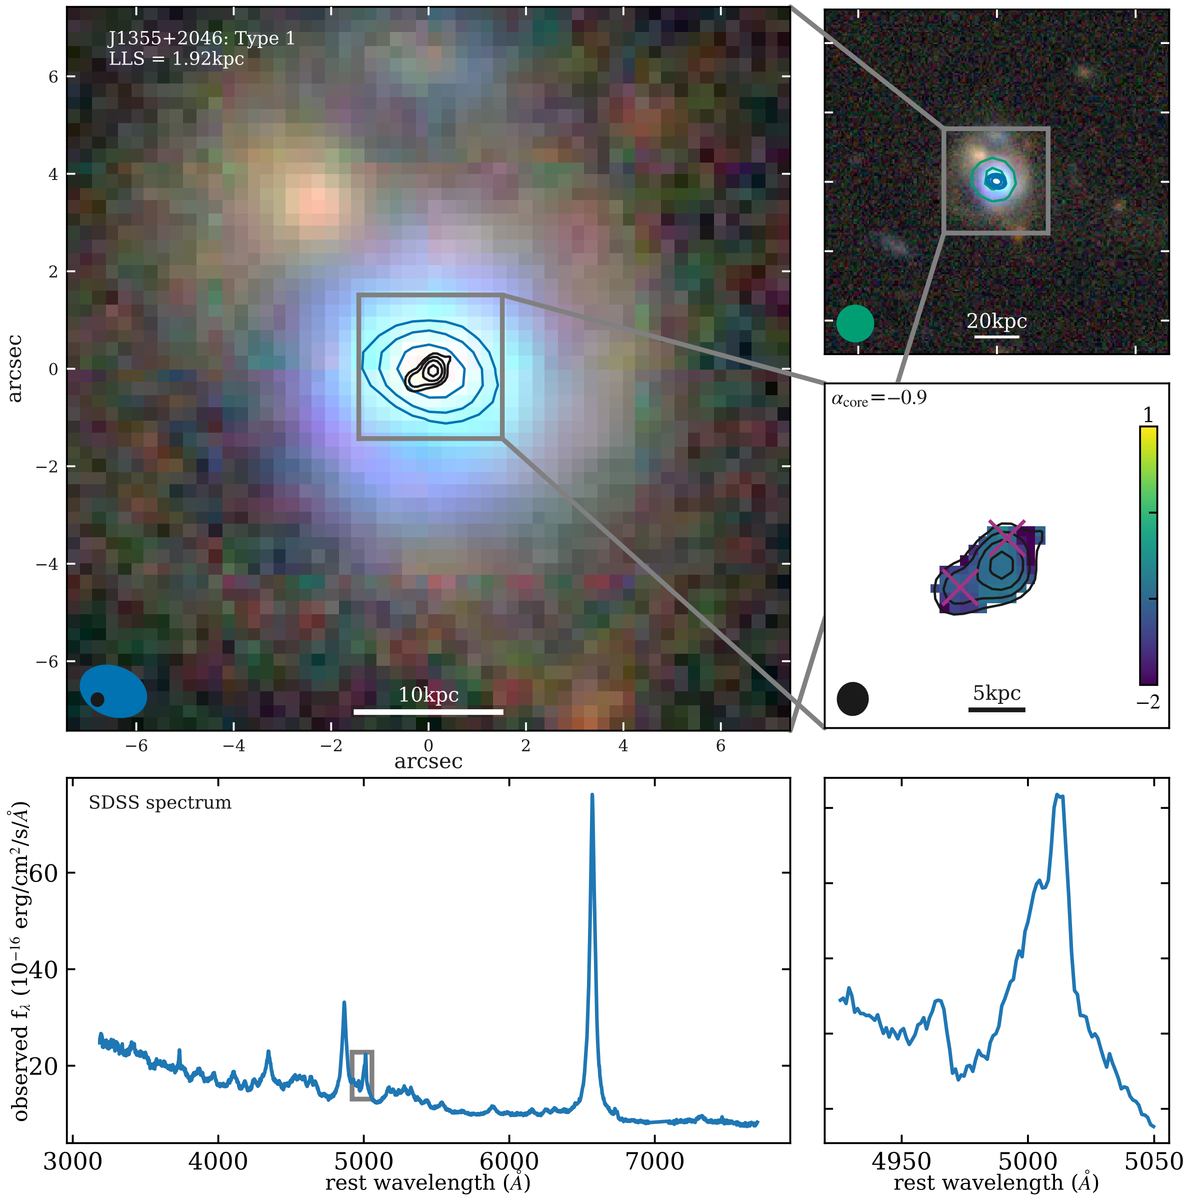


**Figure B31.** As Fig. 2 but for J1355+2046. Radio contours for all data are plotted at ±[8, 16, 32, 64, 128]$\sigma$.

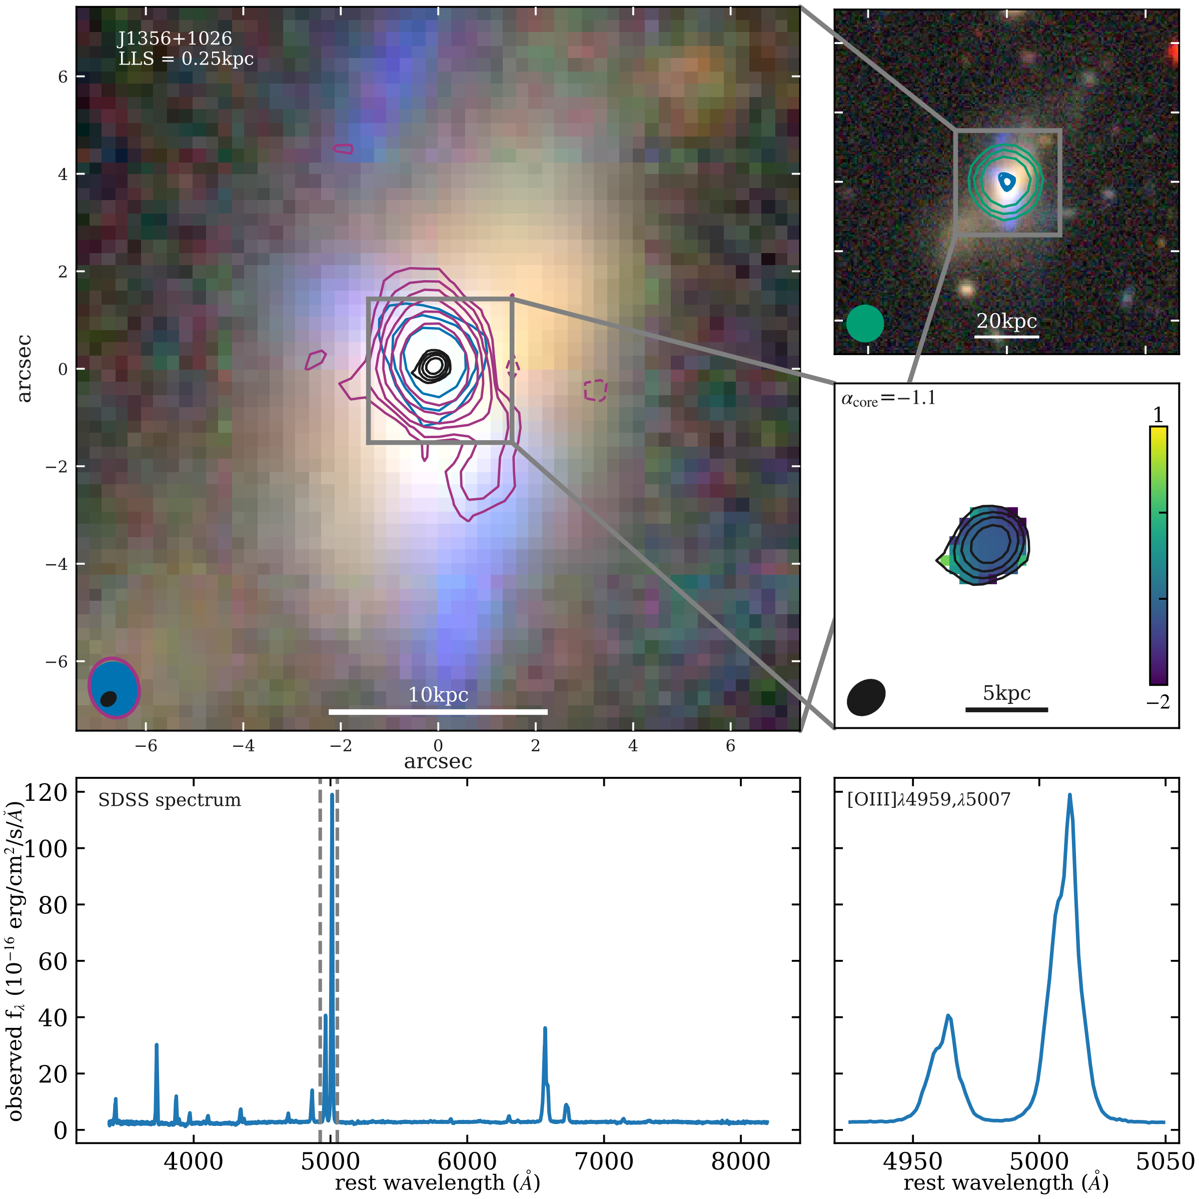


**Figure B32.** As Fig. 2 but for J1356+1026. Radio contours are plotted at ±[32, 64, 128]$\sigma$ in FIRST and our L-band image and at ±[16, 32, 64, 128]$\sigma$ for the C-band data. The magenta contours show the ~1 arcsec C-band radio contours from figure 5 of Jarvis et al. (2019), with contours at ±[4, 8, 16, 32, 64, 128]$\sigma$ and the beam shown as a magenta outline in the bottom left corner.

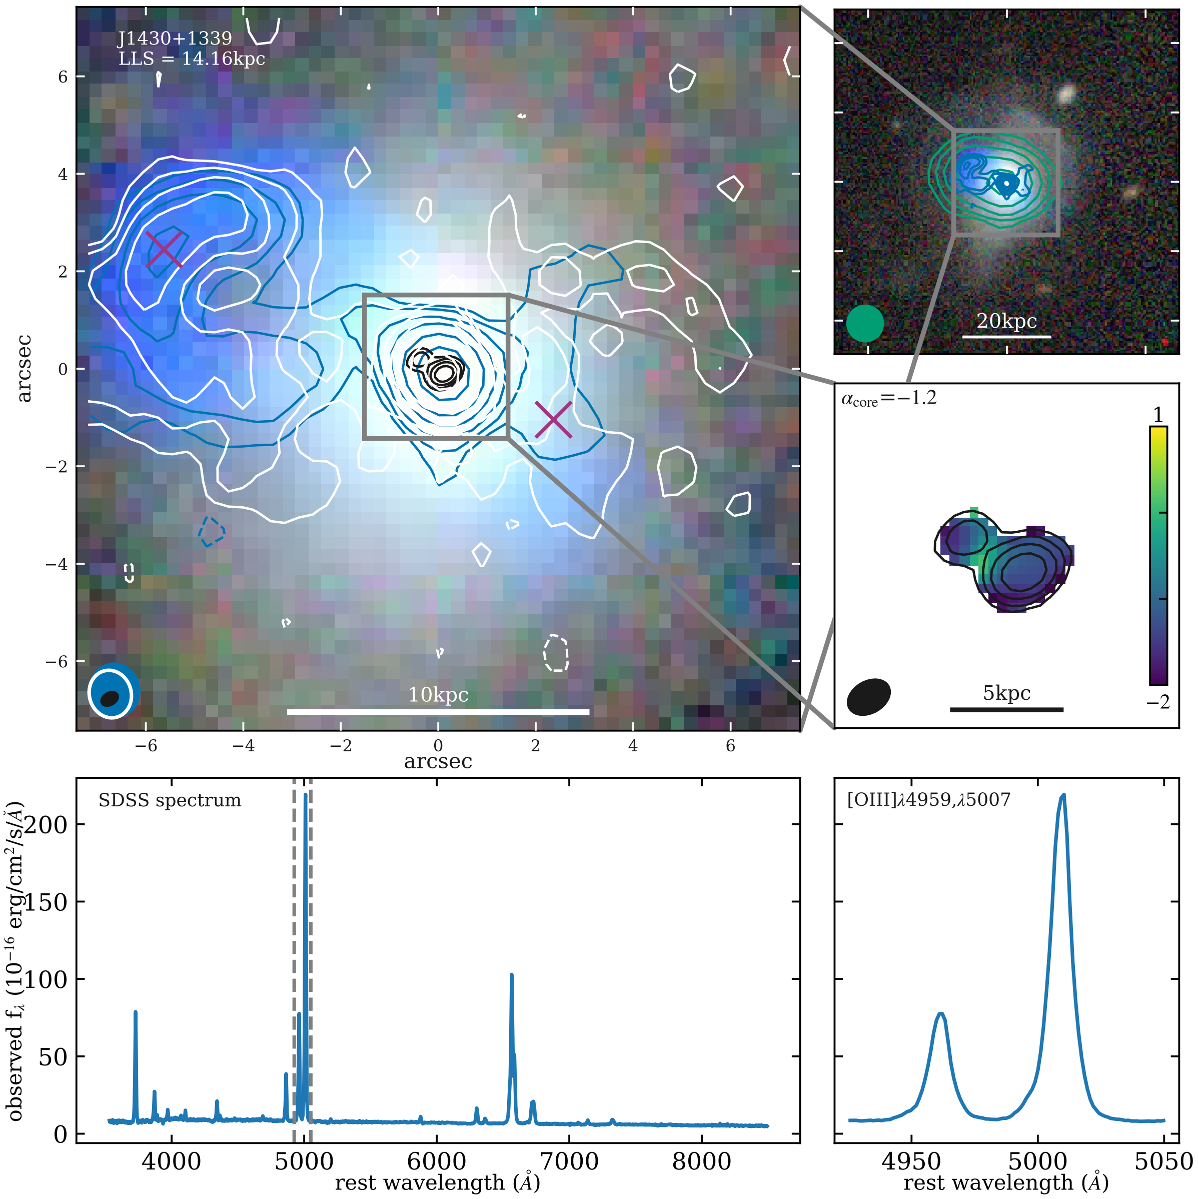


**Figure B33.** As Fig. 2 but for J1430+1339. Radio contours are plotted at ±[4, 8, 16, 32, 64, 128]$\sigma$ in FIRST and our L-band image and at ±[8, 16, 32, 64, 128]$\sigma$ for the C-band data. The white contours show the ∼1 arcsec C-band radio contours from figure 5 of Jarvis et al. (2019) with contours at ±[2, 4, 8, 16, 32, 64, 128]$\sigma$ and the beam shown as a white outline in the bottom left corner.

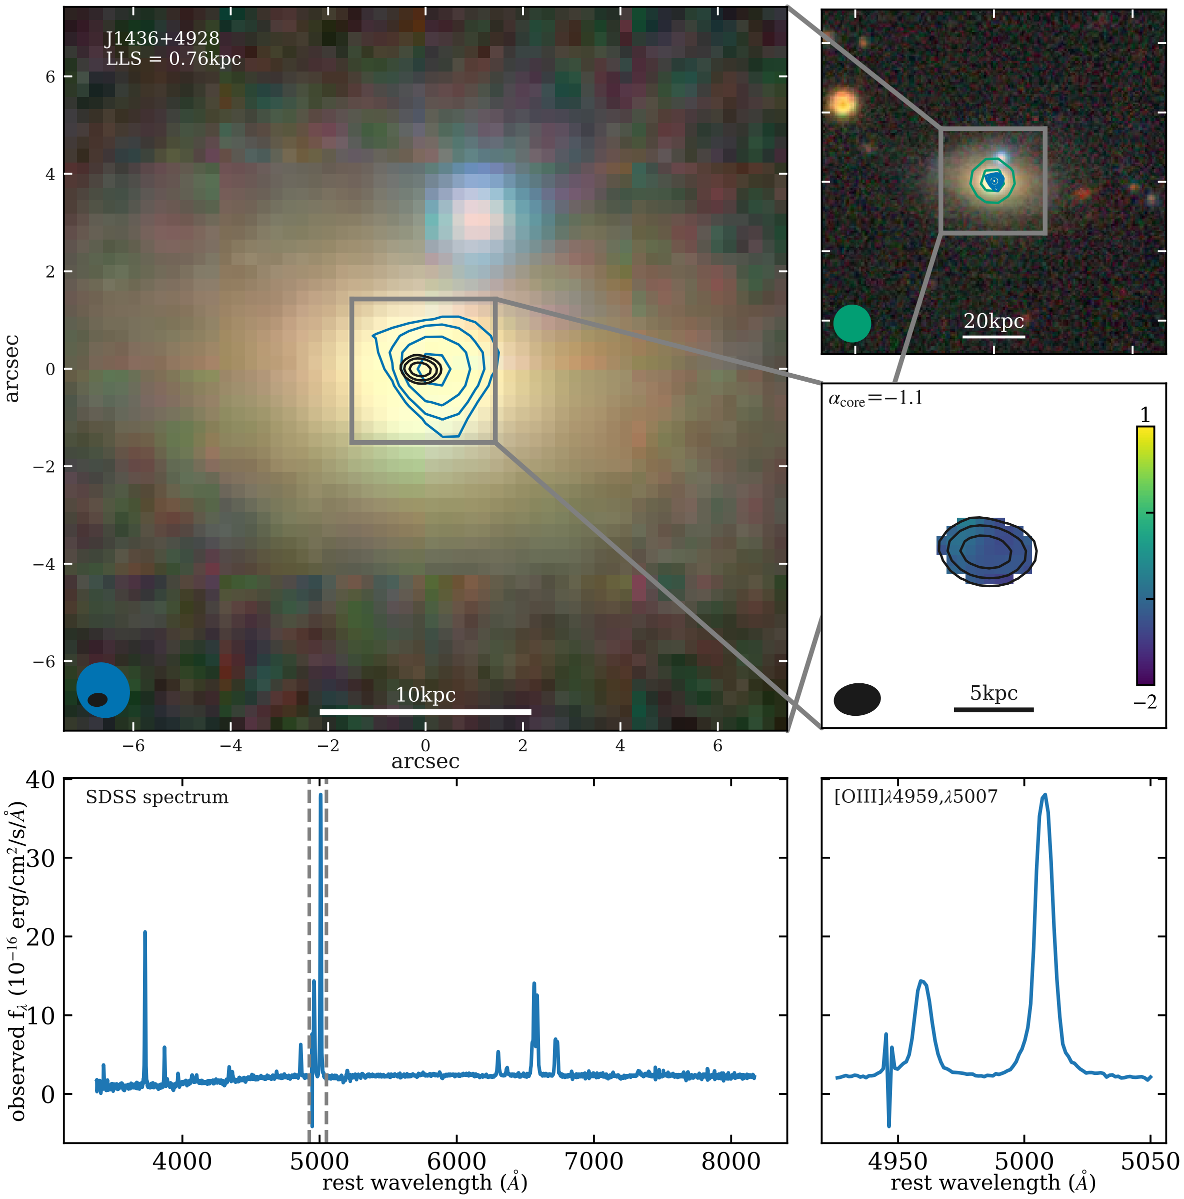


**Figure B34.** As Fig. 2 but for J1436+4928. Radio contours for all data are plotted at ±[16, 32, 64, 128]$\sigma$.

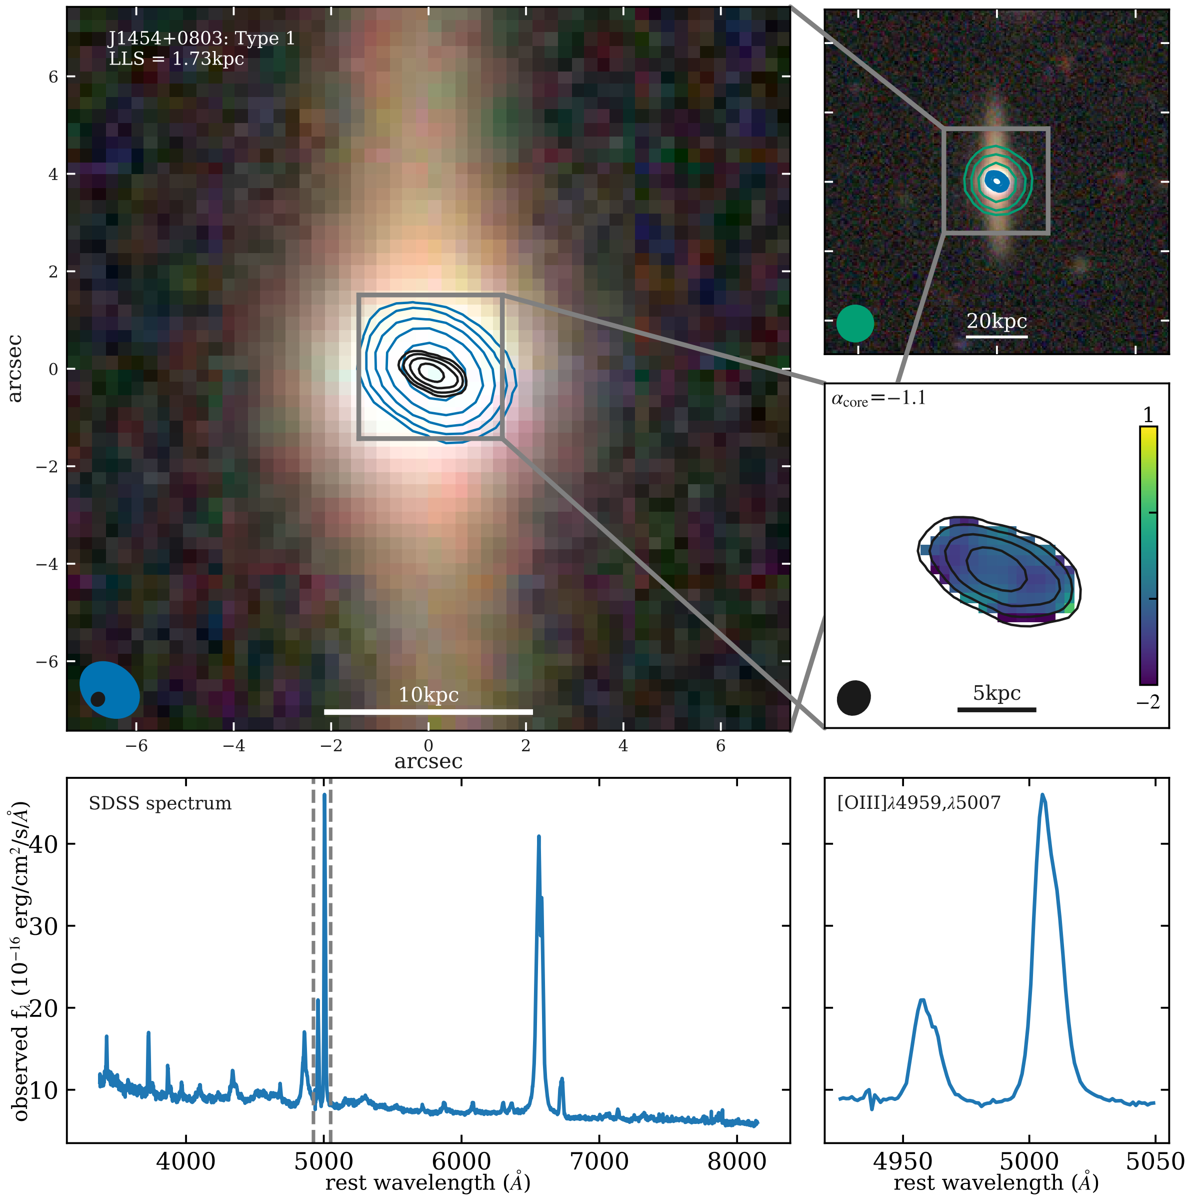


**Figure B35.** As Fig. 2 but for J1454+0803. Radio contours for all data are plotted at ±[8, 16, 32, 64, 128]$\sigma$.

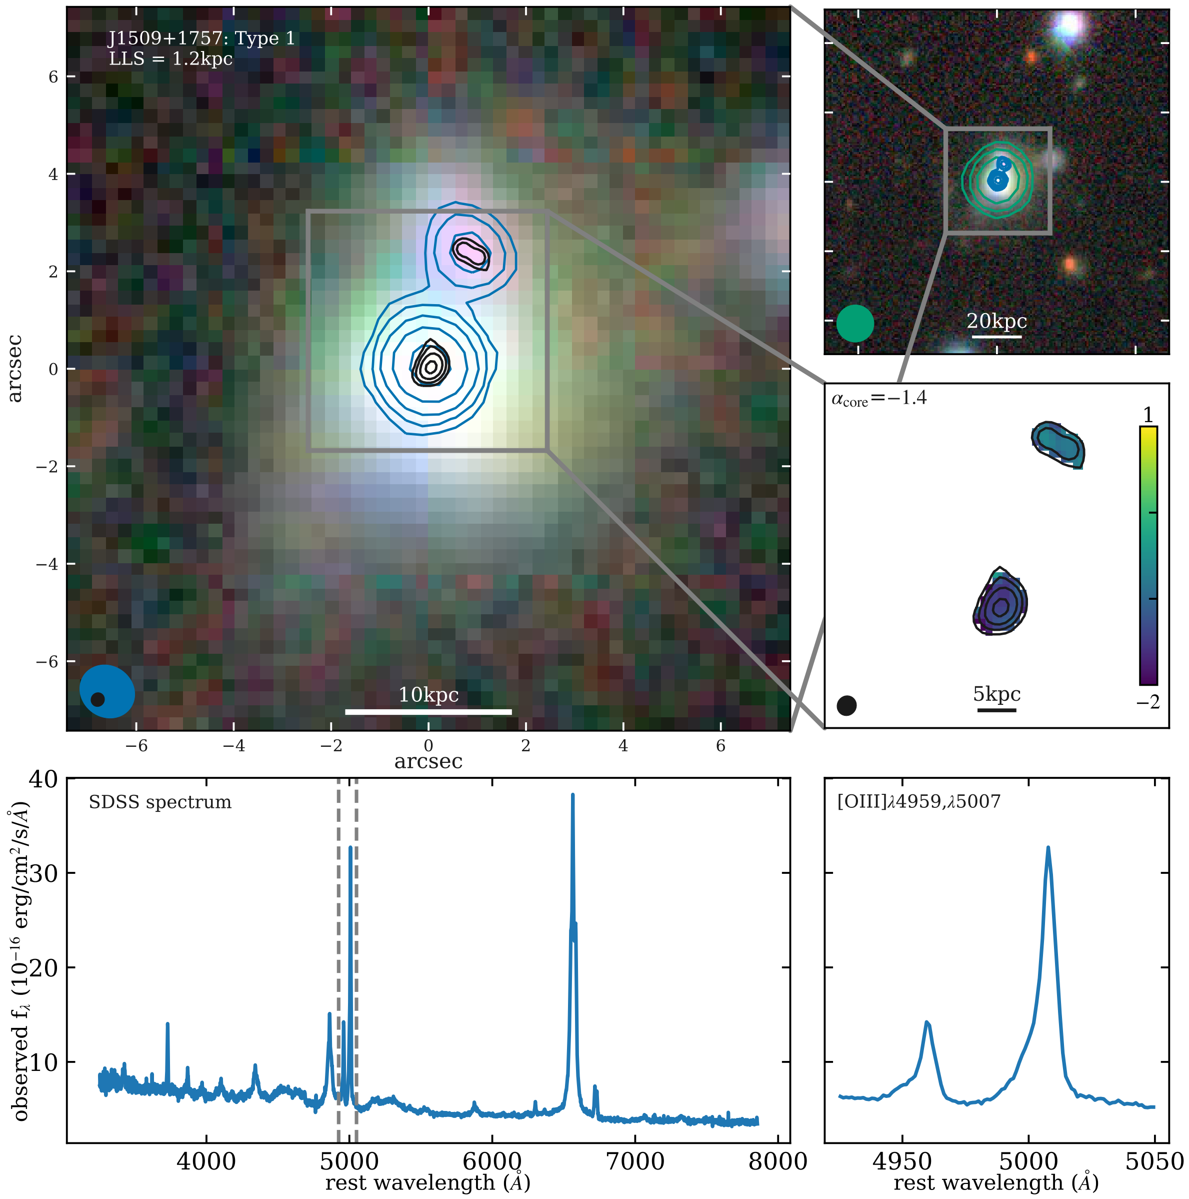


**Figure B36.** As Fig. 2 but for J1509+1757. Radio contours for all data are plotted at ±[8, 16, 32, 64, 128]$\sigma$. As discussed in Section B36 the northern radio component is not associated with the primary target and is therefore not used to calculate the largest linear size for this source.

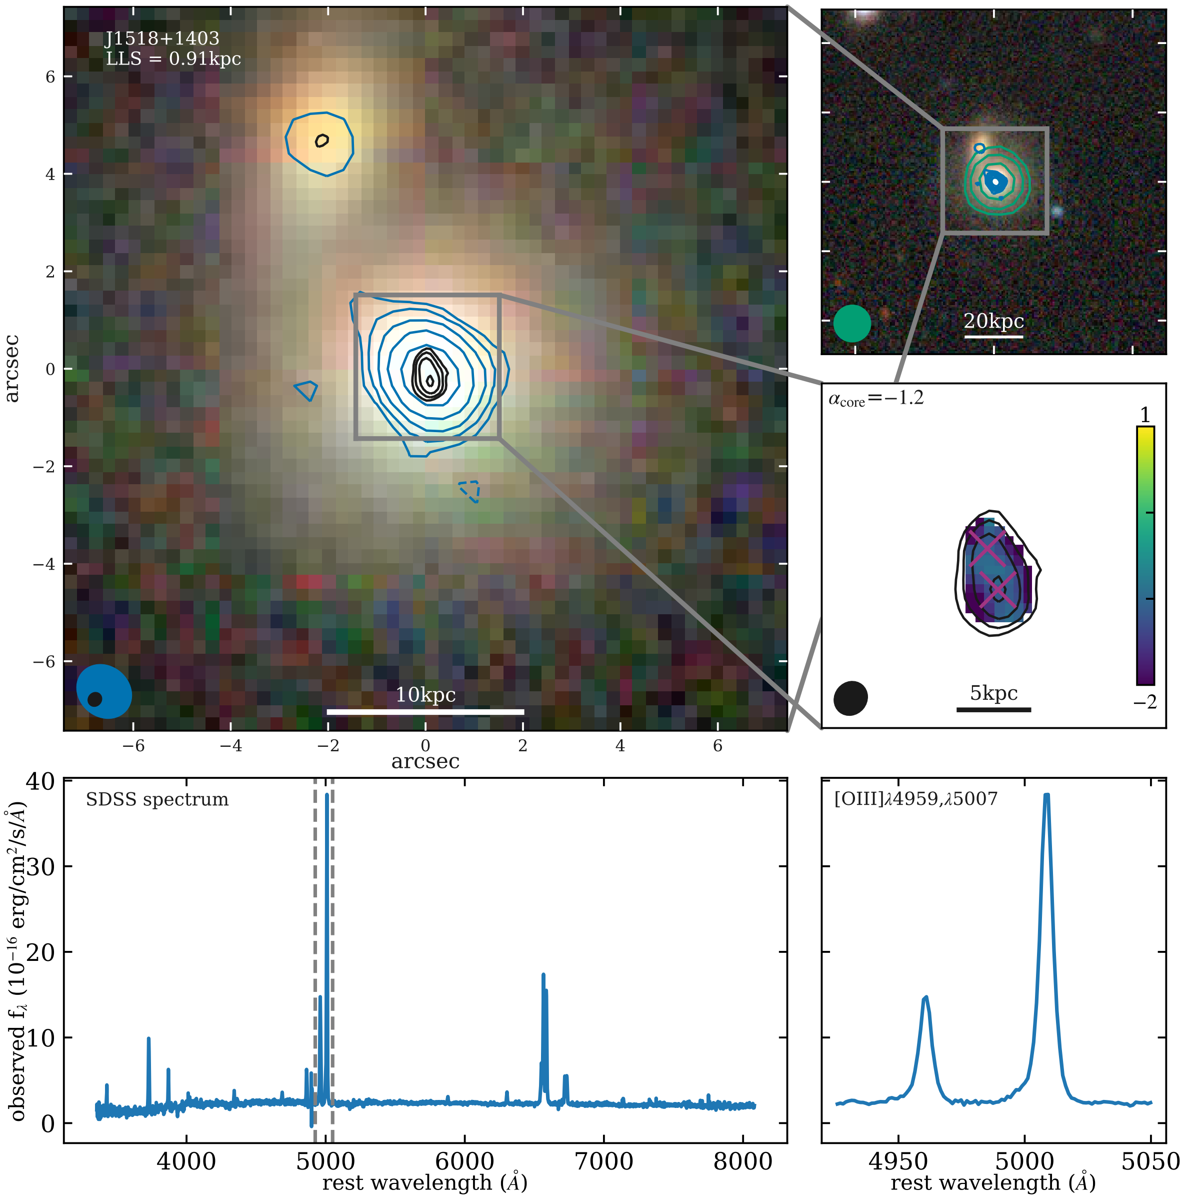


**Figure B37.** As Fig. 2 but for J1518+1403. Radio contours for all data are plotted at ±[4, 8, 16, 32, 64, 128]$\sigma$. As discussed in Section B37 the northern radio component is not associated with the primary target and is therefore not used to calculate the largest linear size for this source.

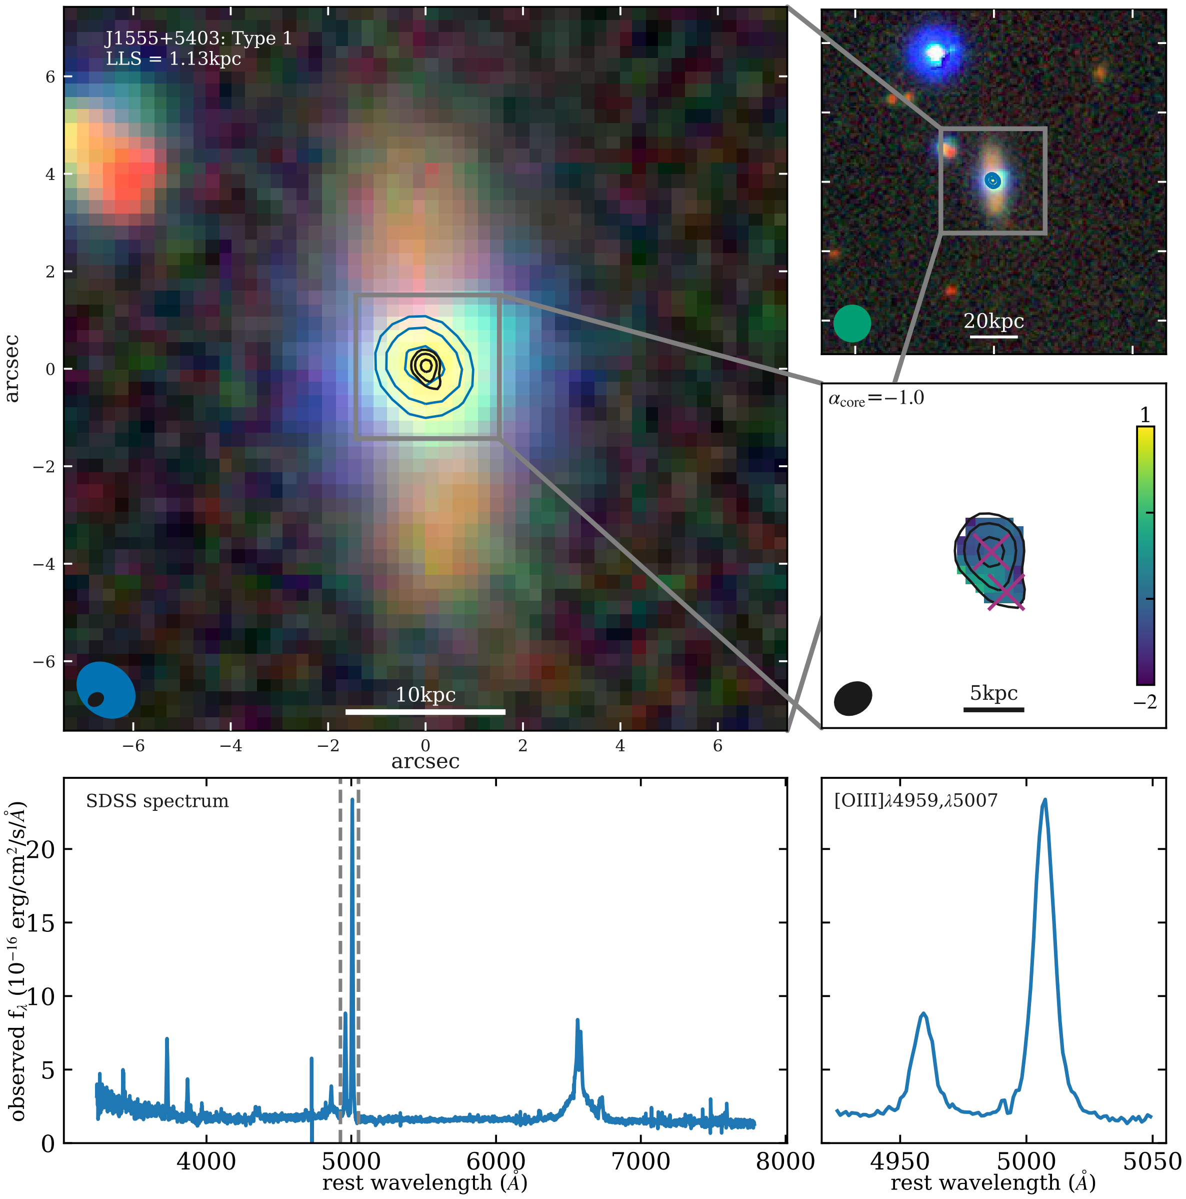


**Figure B38.** As Fig. 2 but for J1555+5403. Radio contours for all data are plotted at ±[4, 8, 16, 32, 64, 128]$\sigma$.

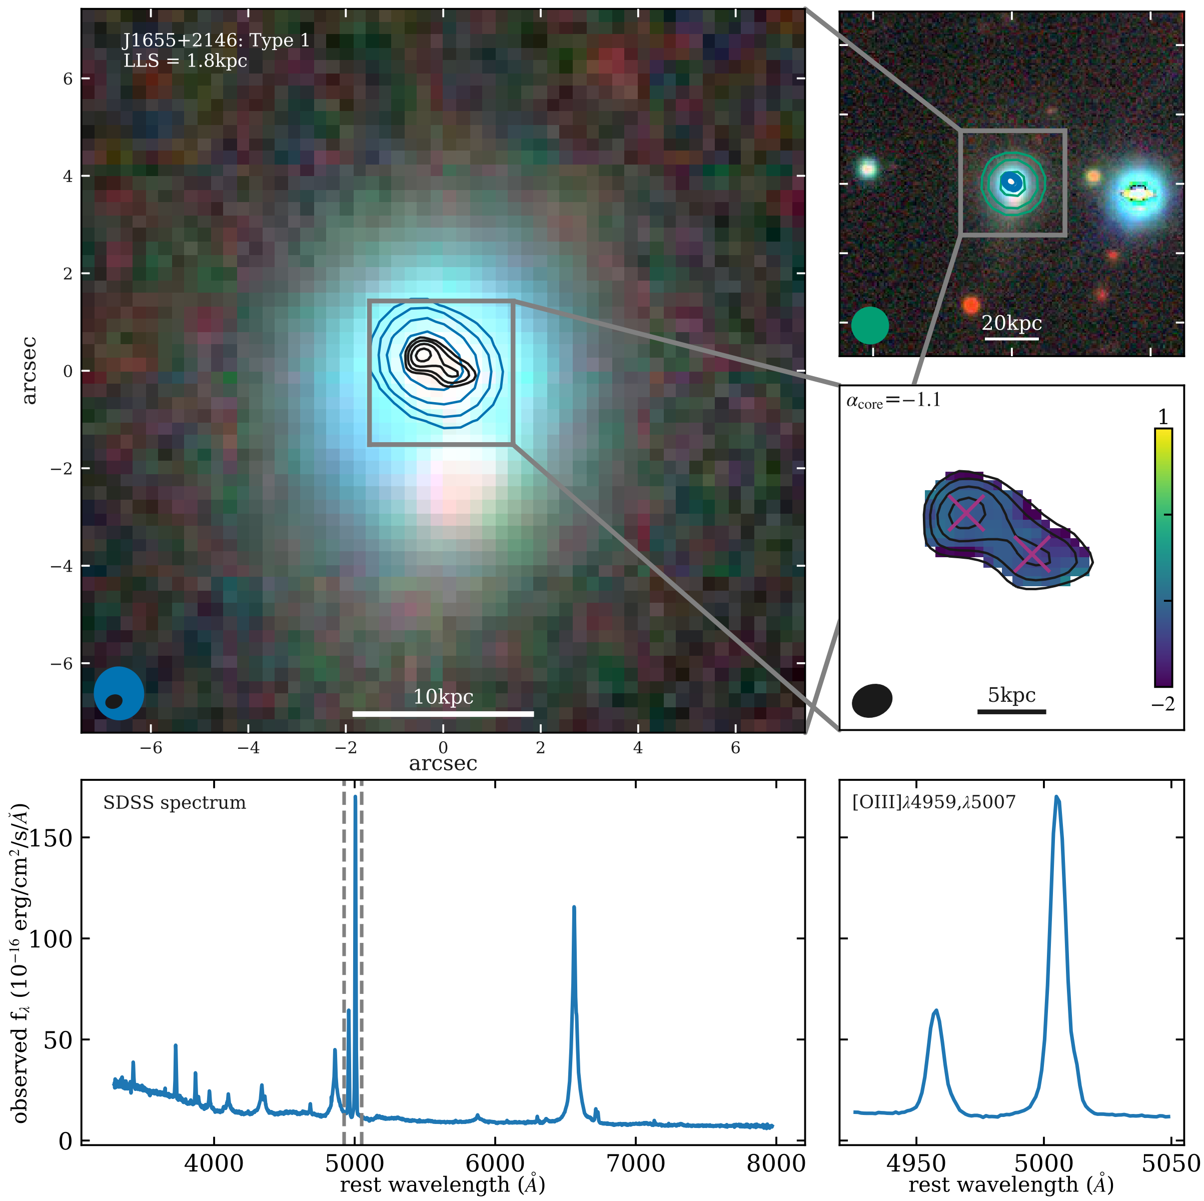


**Figure B39.** As Fig. 2 but for J1655+2146. Radio contours for all data are plotted at ±[8, 16, 32, 64, 128]$\sigma$.

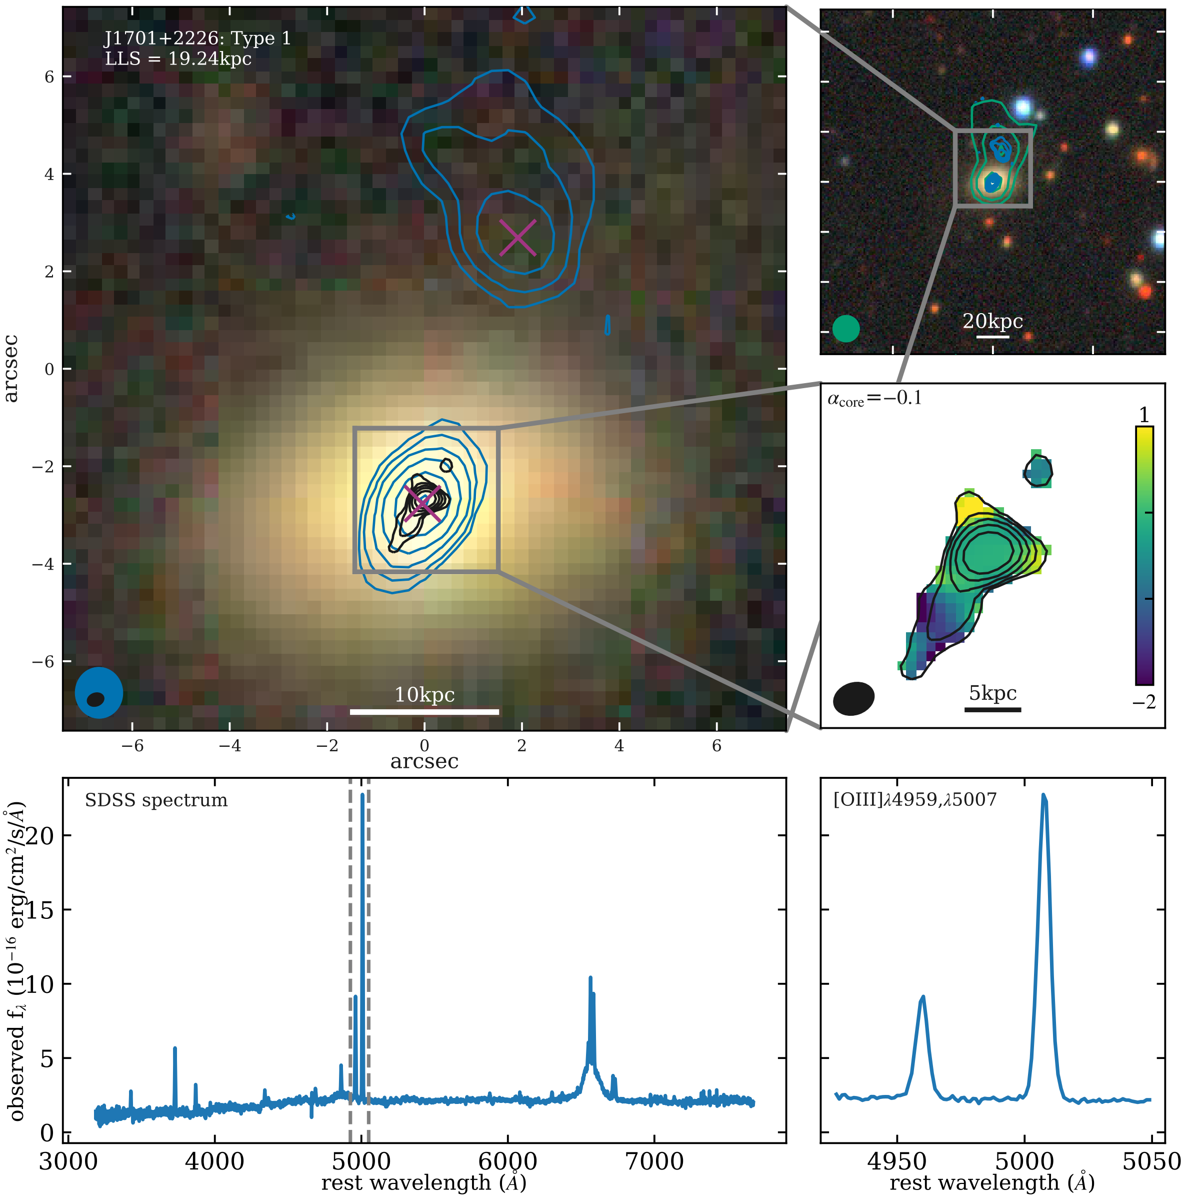


**Figure B40.** As Fig. 2 but for J1701+2226. Radio contours are plotted at ±[4, 8, 16, 32, 64, 128]$\sigma$ in FIRST and our L-band image and at ±[8, 16, 32, 64, 128]$\sigma$ for the C-band data.

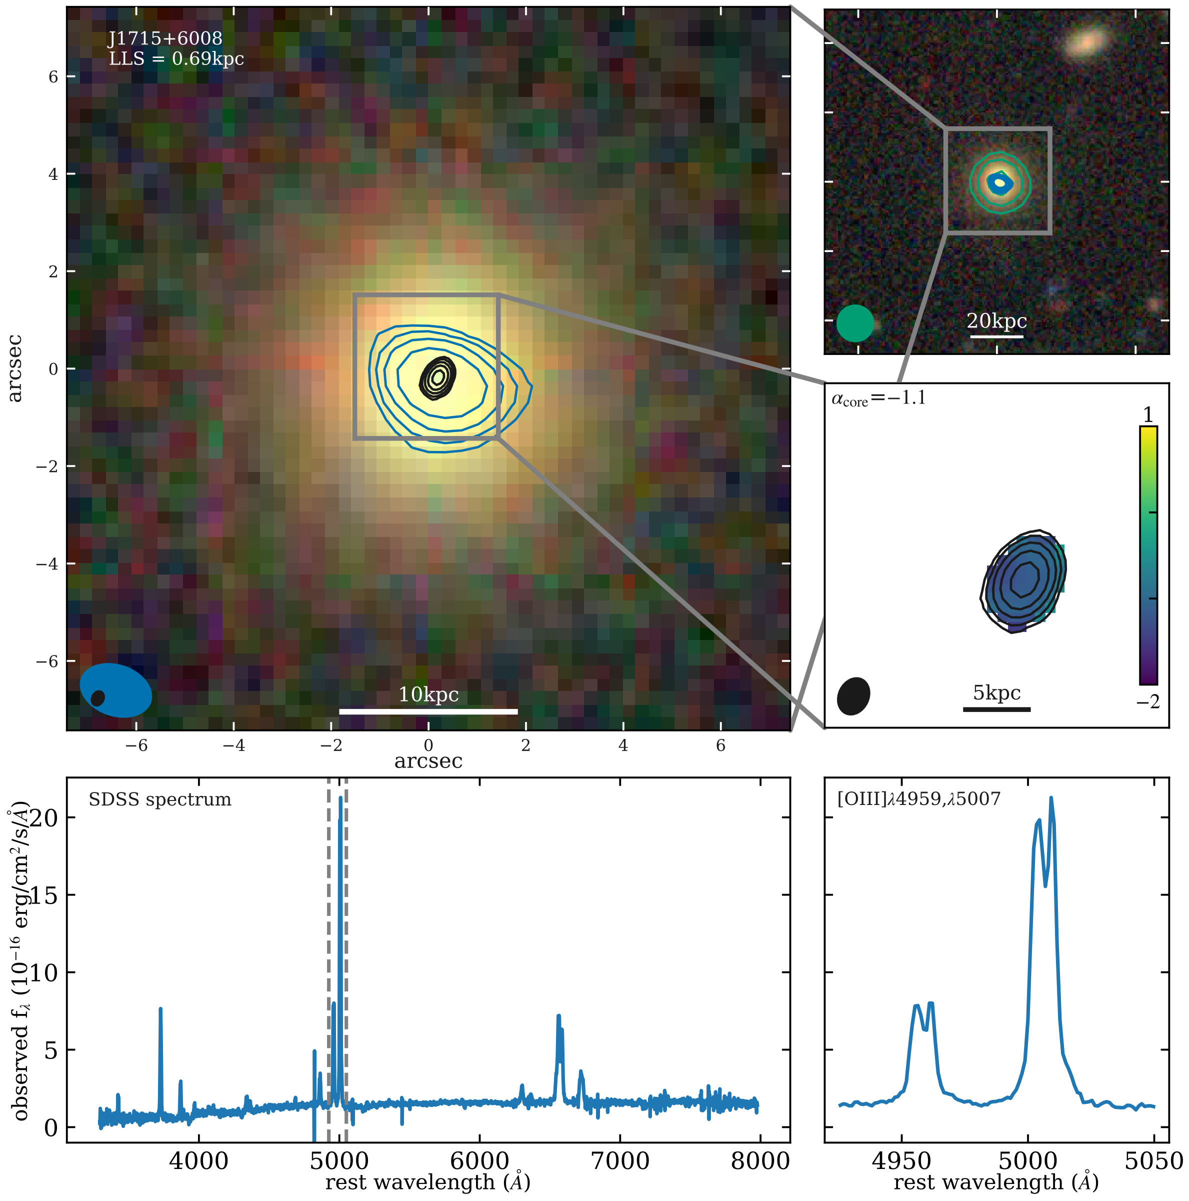


**Figure B41.** As Fig. 2 but for J1715+6008. Radio contours are plotted at ±[16, 32, 64, 128]$\sigma$ in FIRST and our L-band image and at ±[8, 16, 32, 64, 128]$\sigma$ for the C-band data.
